# Supplementary material for: Visual Embodied Brain: Let Multimodal Large Language Models See, Think, and Control in Spaces
Source: arXiv:2506.00123 source file (2025-05-30)
Supplement: Supplementary file 1 [file appendix_3d_demo.tex]

\begin{table}[ht]
    \centering
    \begin{tabular}{cccc}
    \toprule
    \multicolumn{4}{c}{\textbf{Spatial Reasoning: Example \#1 from Multi3DRef.}} \\
    \midrule
    \includegraphics[width=0.22\linewidth]{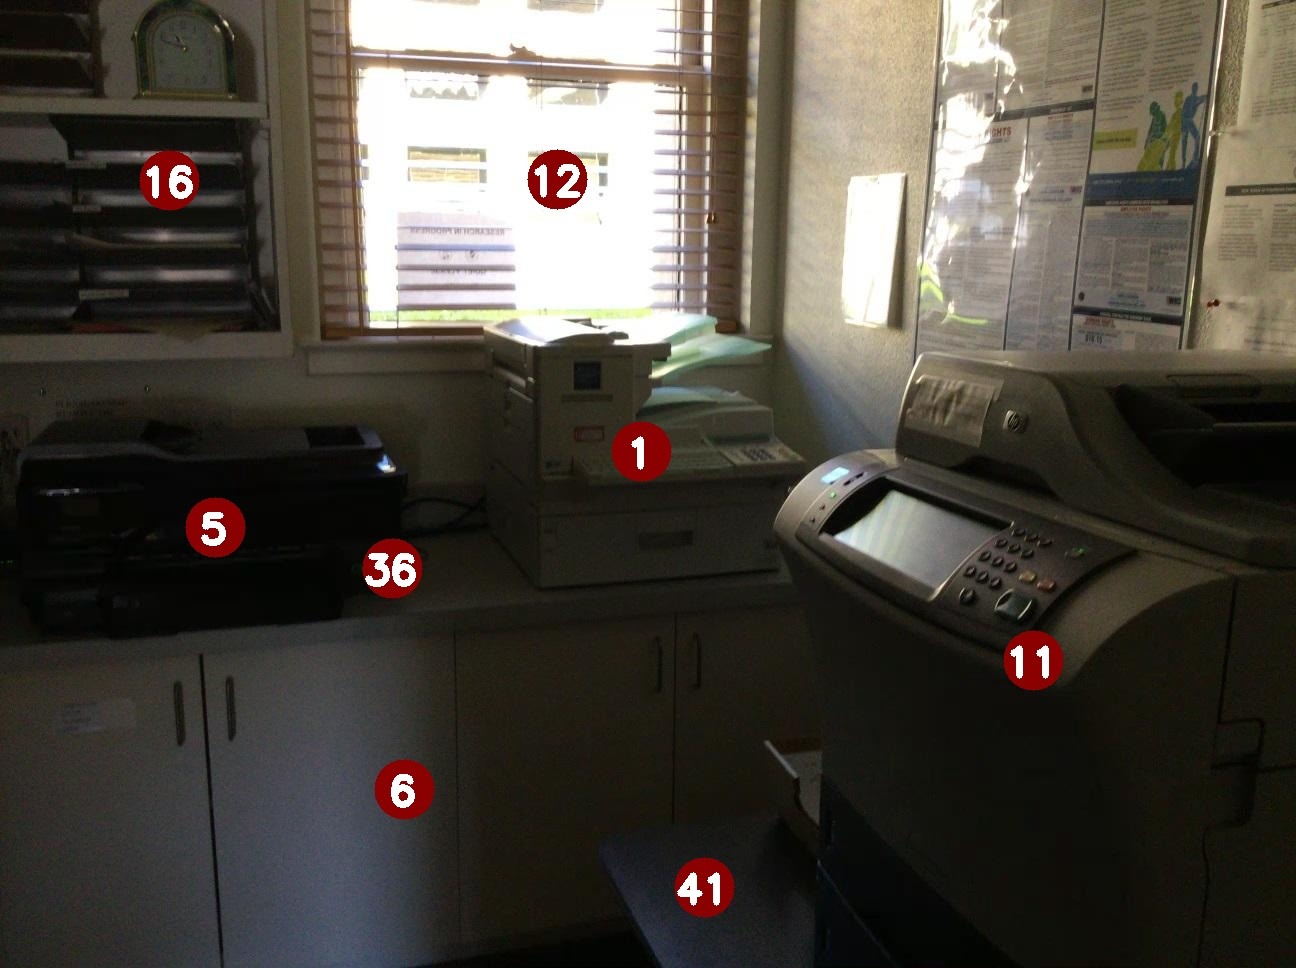} &
    \includegraphics[width=0.22\linewidth]{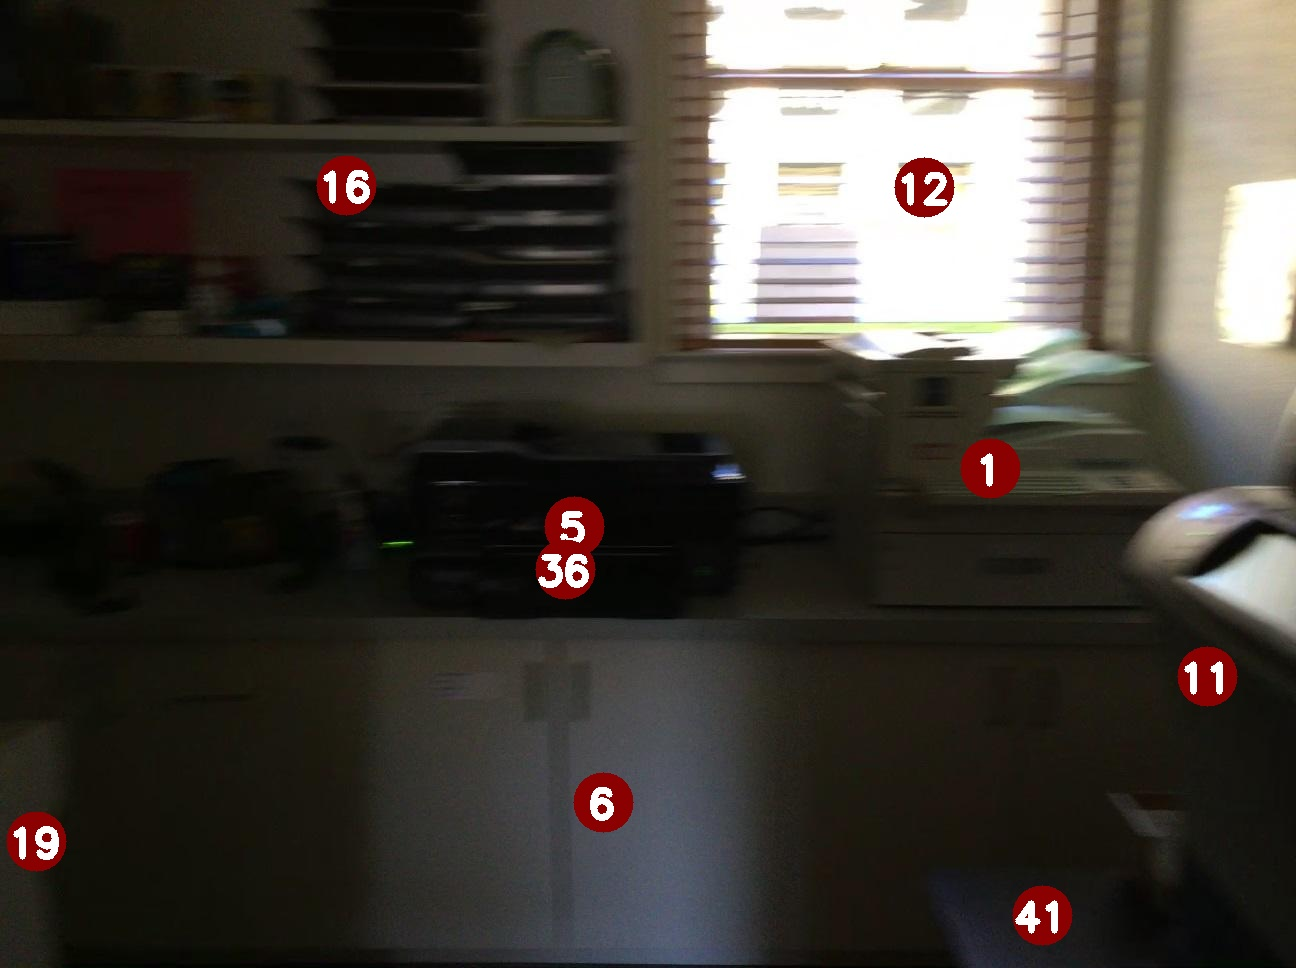} &
    \includegraphics[width=0.22\linewidth]{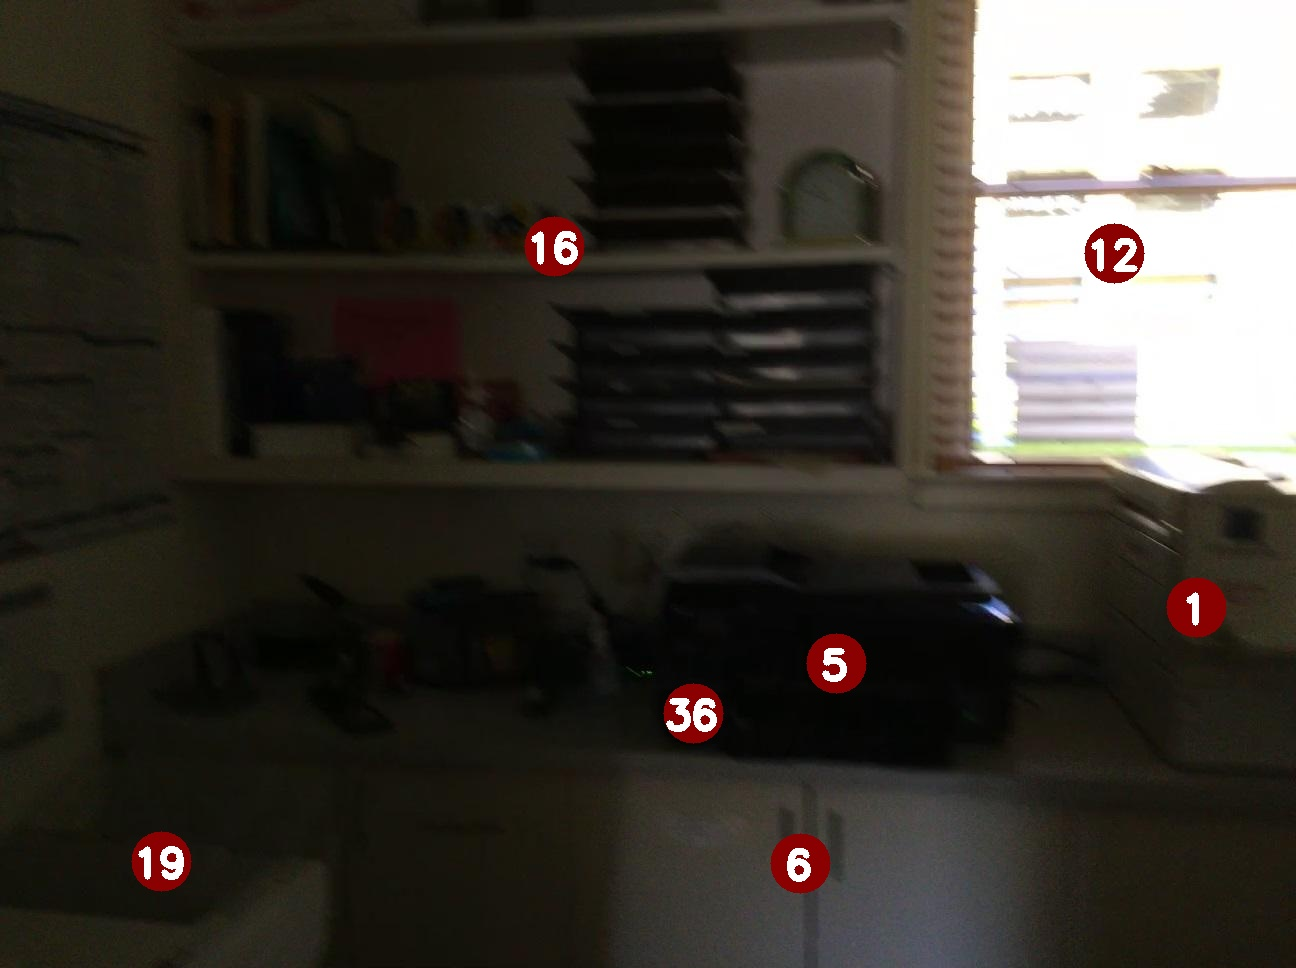} &
    \includegraphics[width=0.22\linewidth]{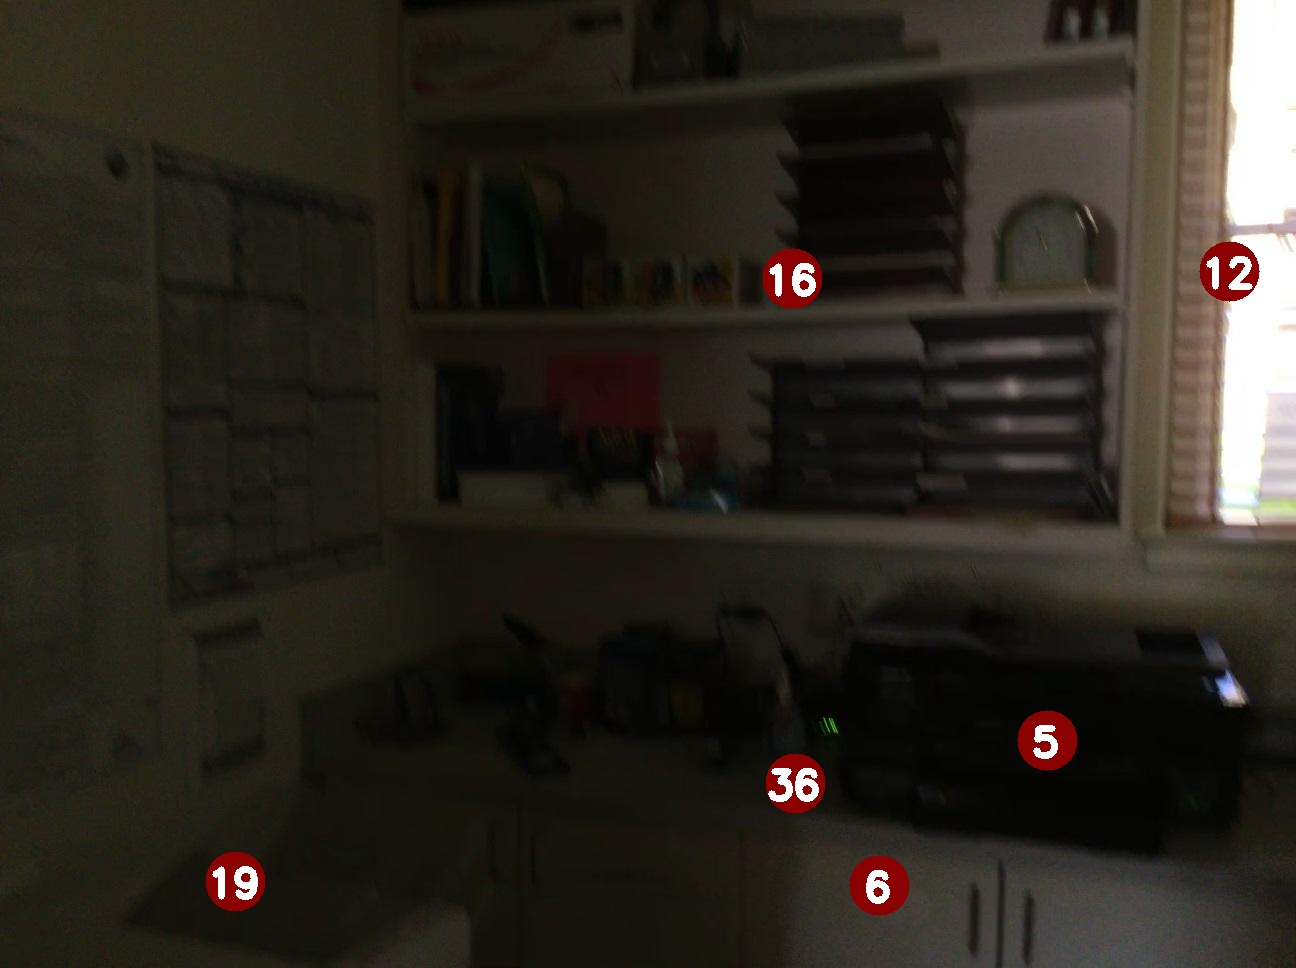} \\
    \vspace{0.1em} \\
    \includegraphics[width=0.22\linewidth]{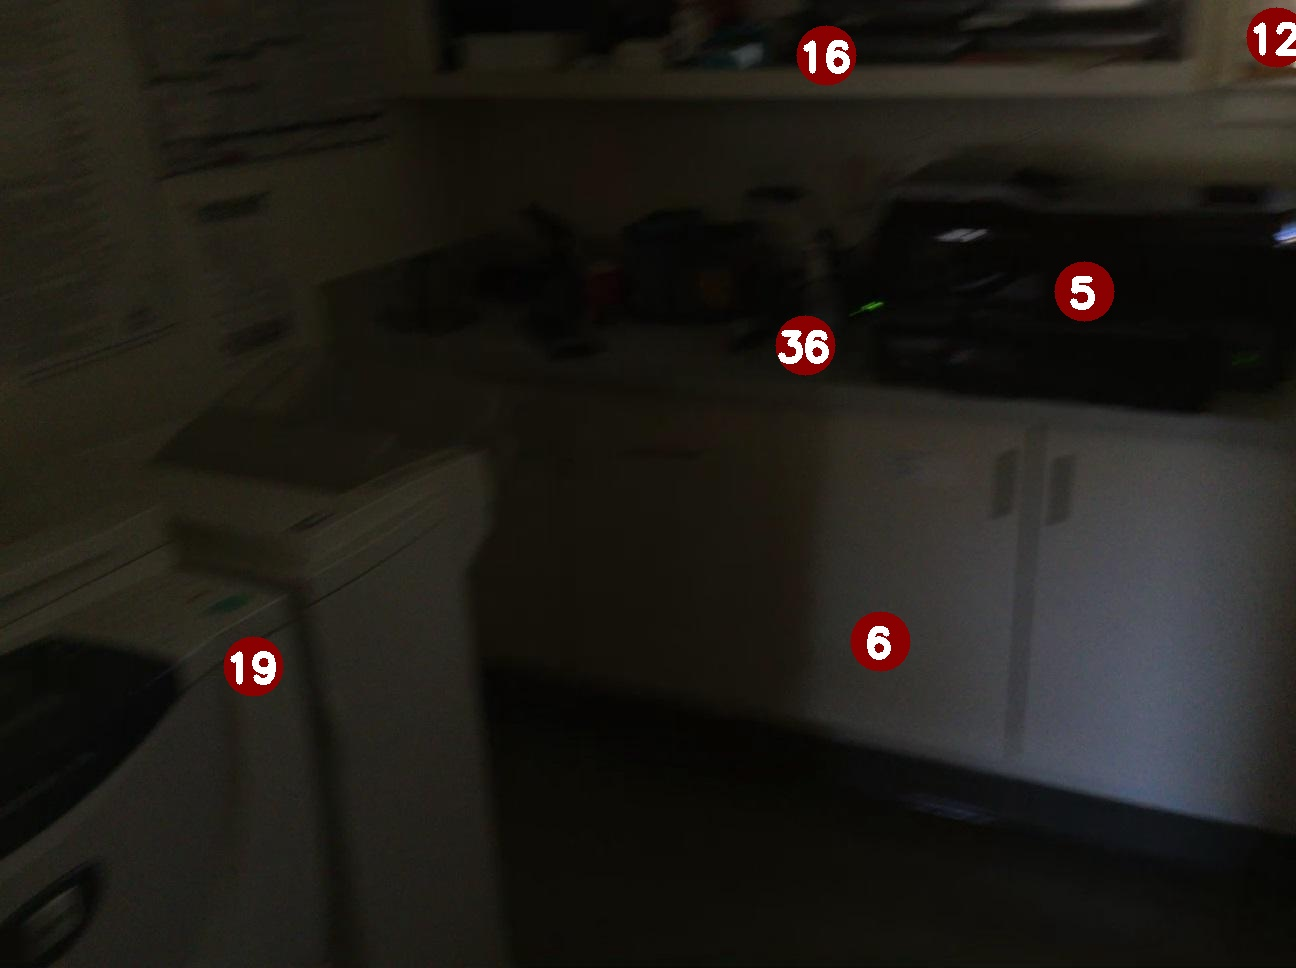} &
    \includegraphics[width=0.22\linewidth]{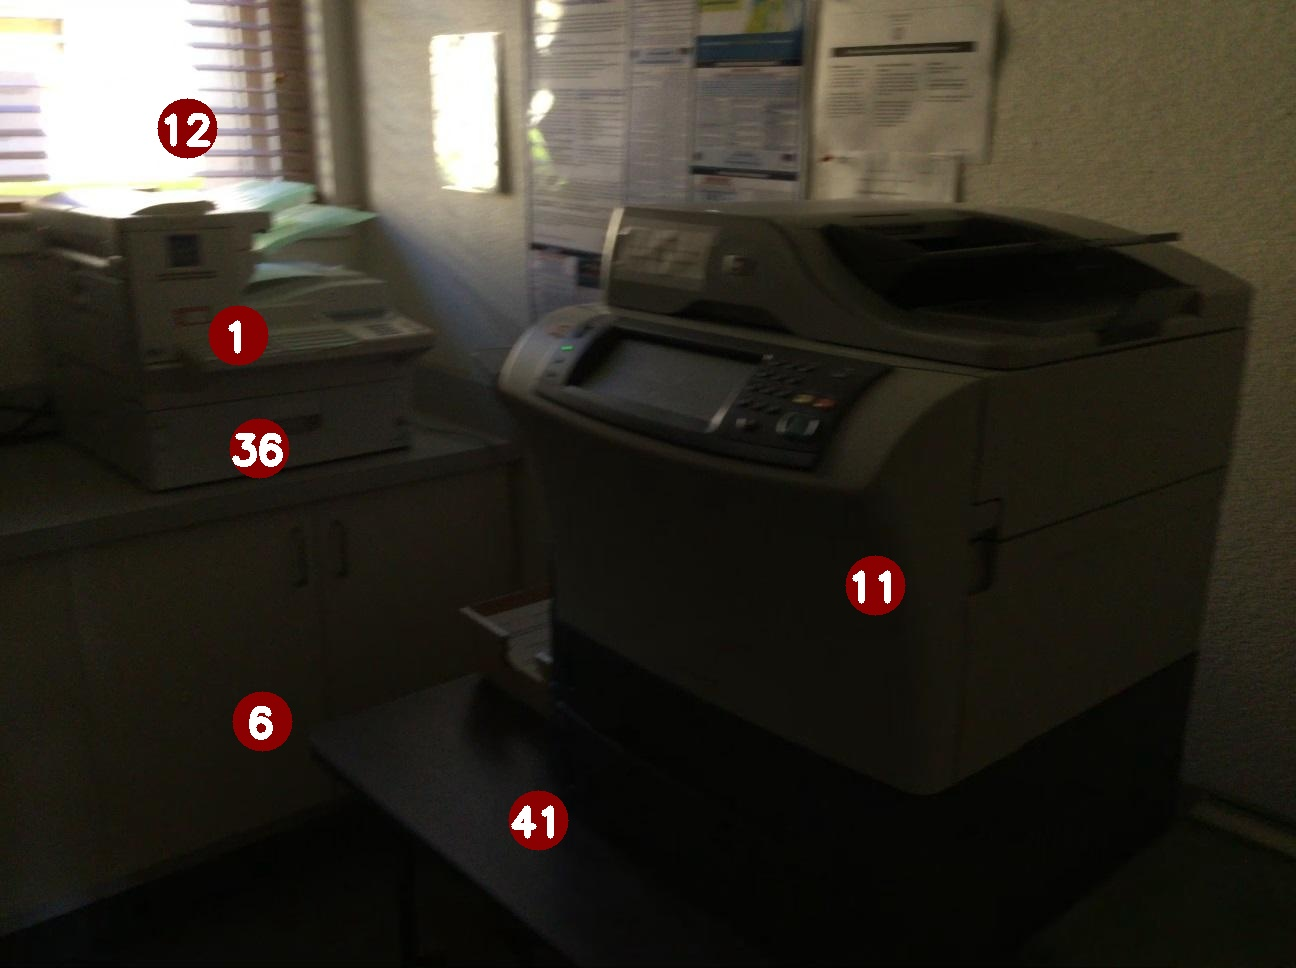} &
    \includegraphics[width=0.22\linewidth]{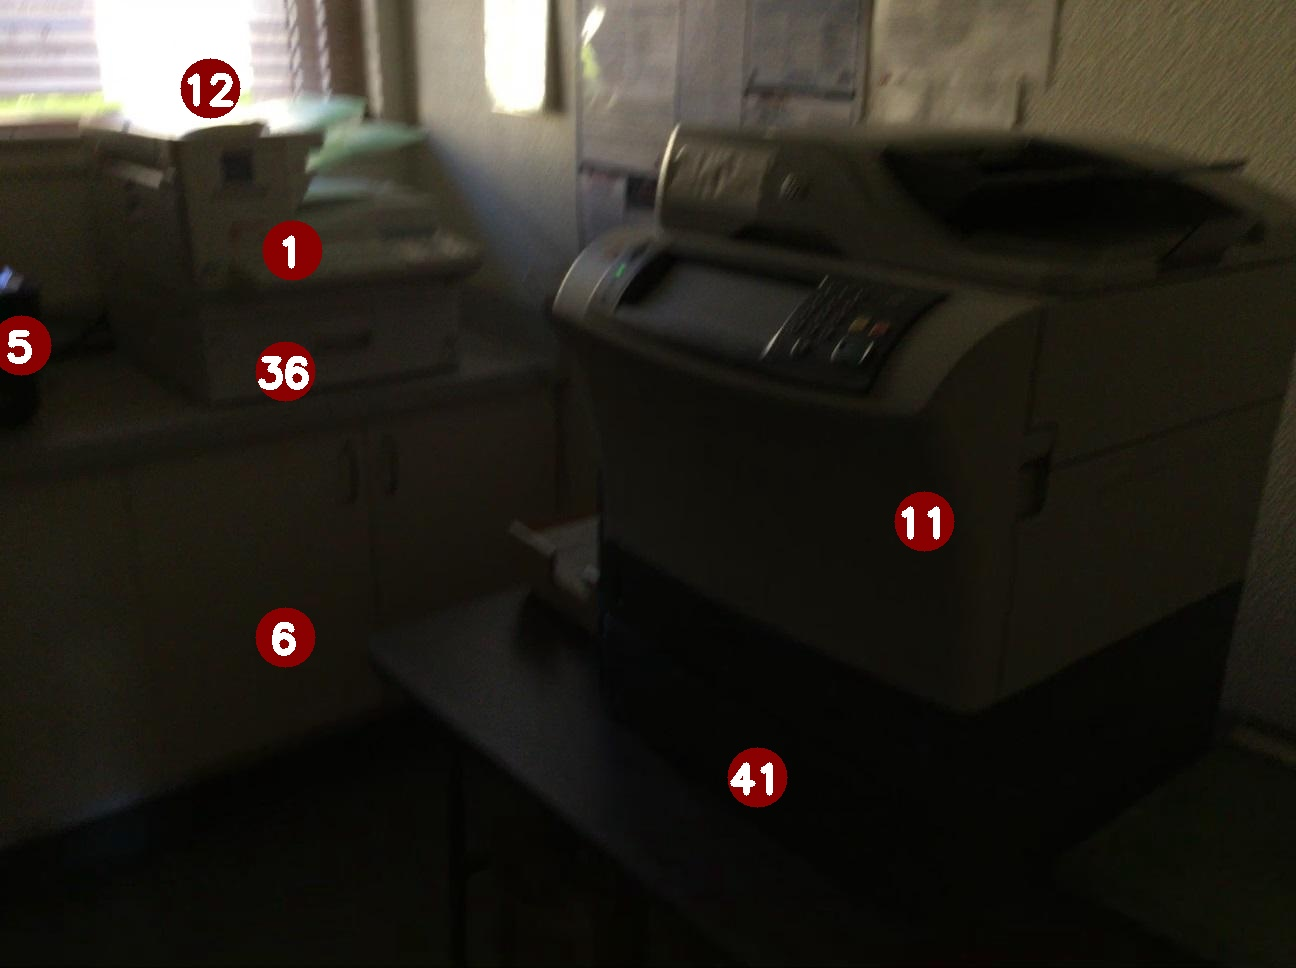} &
    \includegraphics[width=0.22\linewidth]{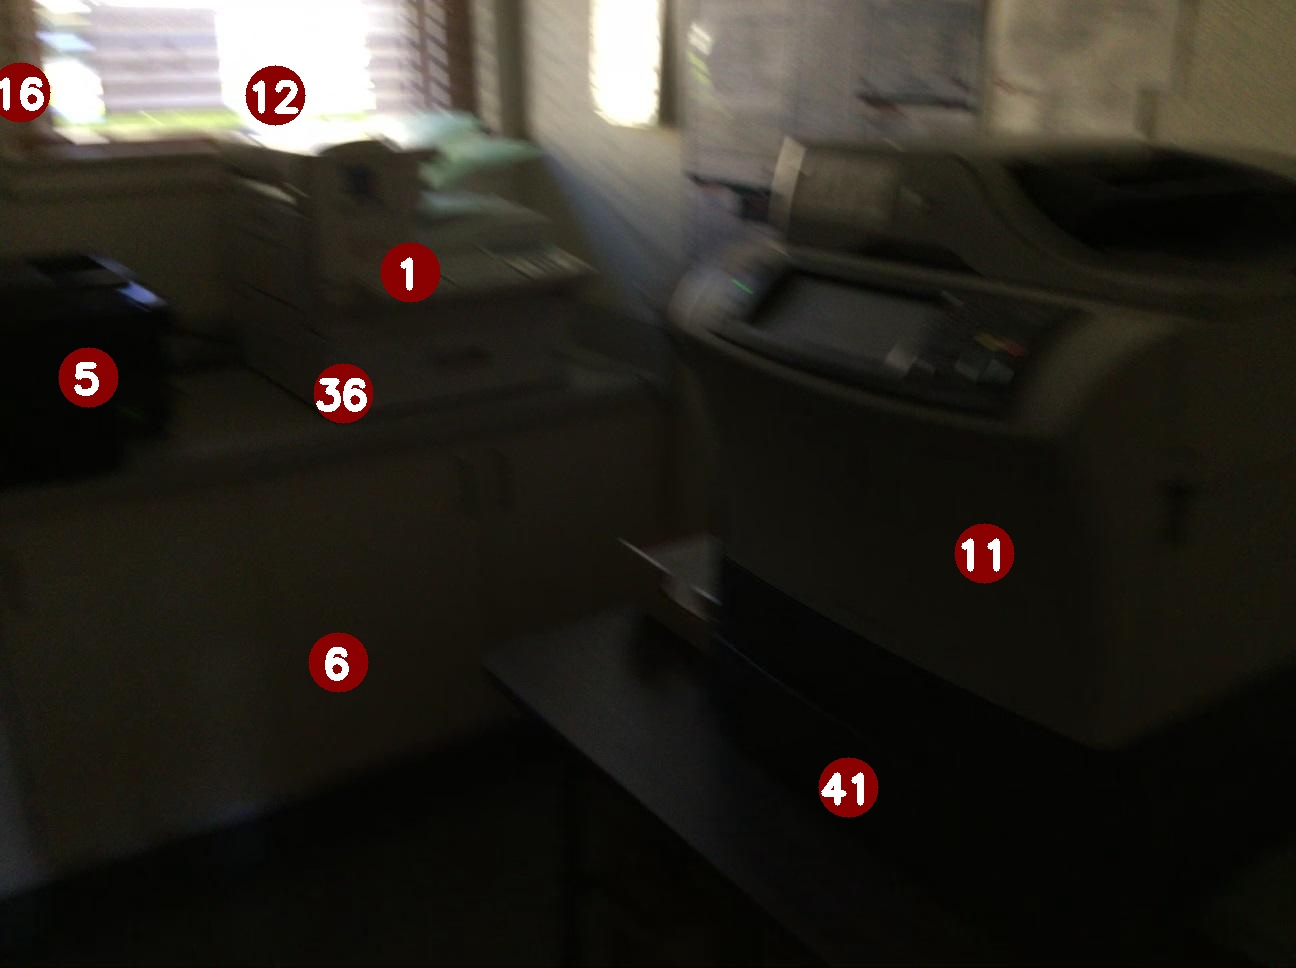} \\
    \textbf{Question}: & \multicolumn{3}{p{0.72\linewidth}}{Are there any objects that correspond to the description "at the end of the room, against a wall and is a rectangular cabinet"? If yes, could you share the IDs for those objects?} \\
    \midrule
    \textbf{Qwen2.5-VL}: & \multicolumn{3}{p{0.72\linewidth}}{\colorbox{red!20}{No}} \\
    \midrule
    \textbf{VeBrain}: & \multicolumn{3}{p{0.72\linewidth}}{\colorbox{green!20}{Yes}. <OBJ006>.} \\
    \bottomrule
    \end{tabular}
\end{table}

\begin{table}[ht]
    \centering
    % \caption{\textbf{An Example from Scan2Cap.}}
    % 第一行图片
    % \begin{tabular}{>{\centering\arraybackslash}m{0.22\linewidth}
    %                 >{\centering\arraybackslash}m{0.22\linewidth}
    %                 >{\centering\arraybackslash}m{0.22\linewidth}
    %                 >{\centering\arraybackslash}m{0.22\linewidth}}
    
    \begin{tabular}{cccc}
    \toprule
    \multicolumn{4}{c}{\textbf{Spatial Reasoning: Example \#2 from Scan2Cap.}} \\
    \midrule
    \includegraphics[width=0.22\linewidth]{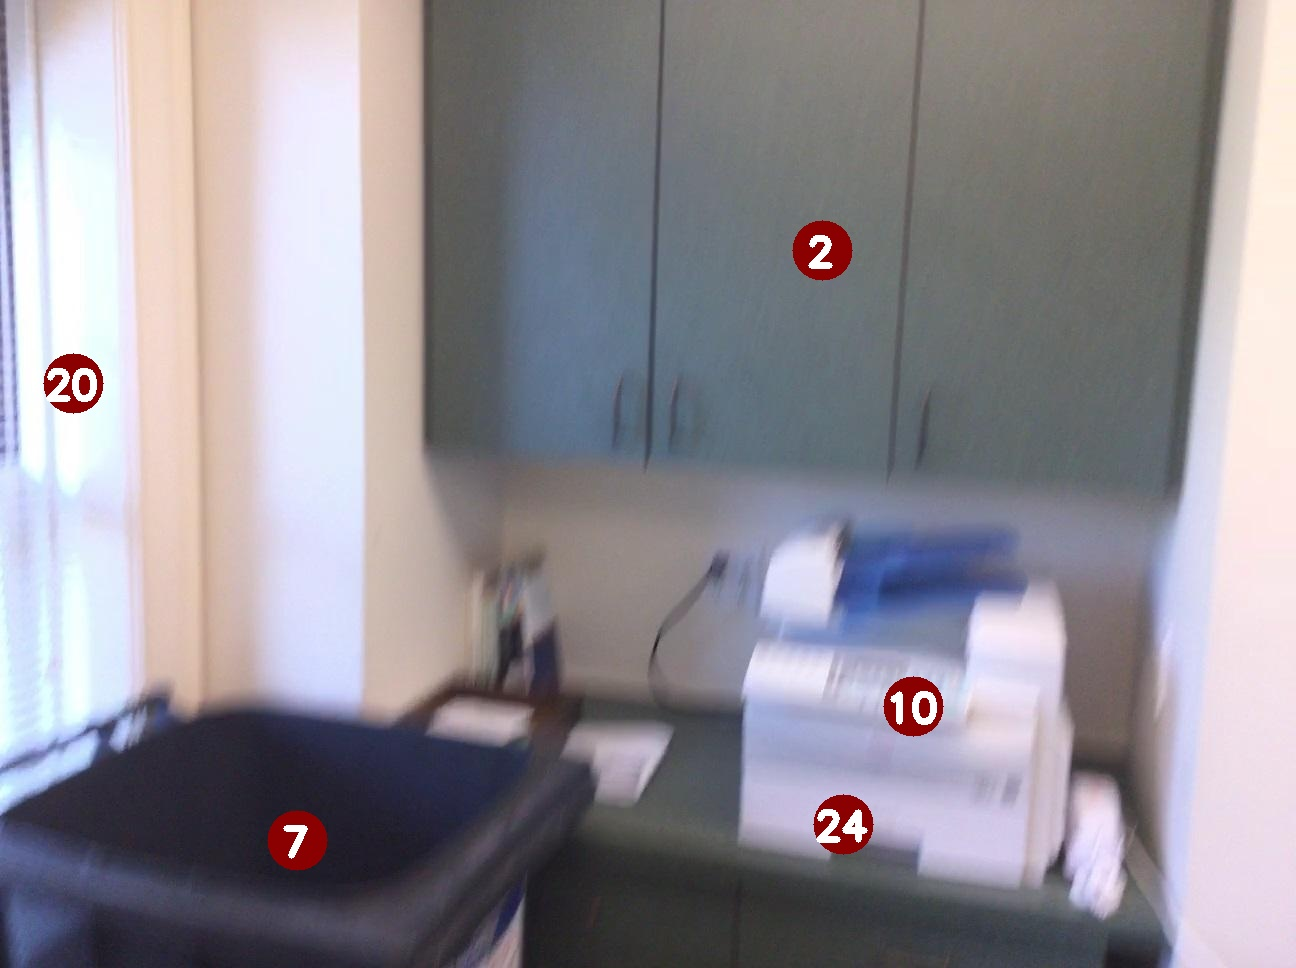} &
    \includegraphics[width=0.22\linewidth]{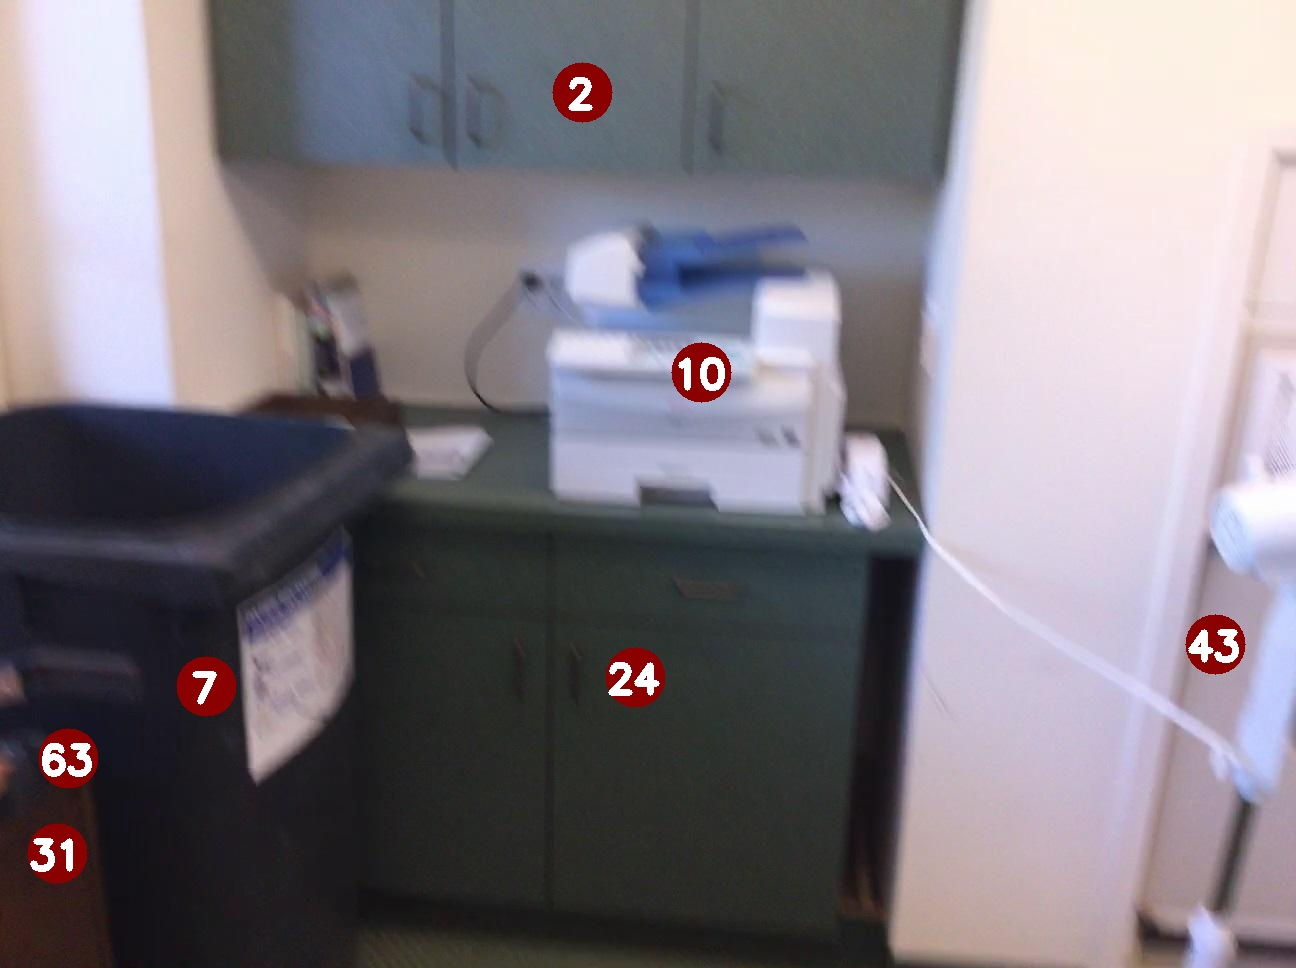} &
    \includegraphics[width=0.22\linewidth]{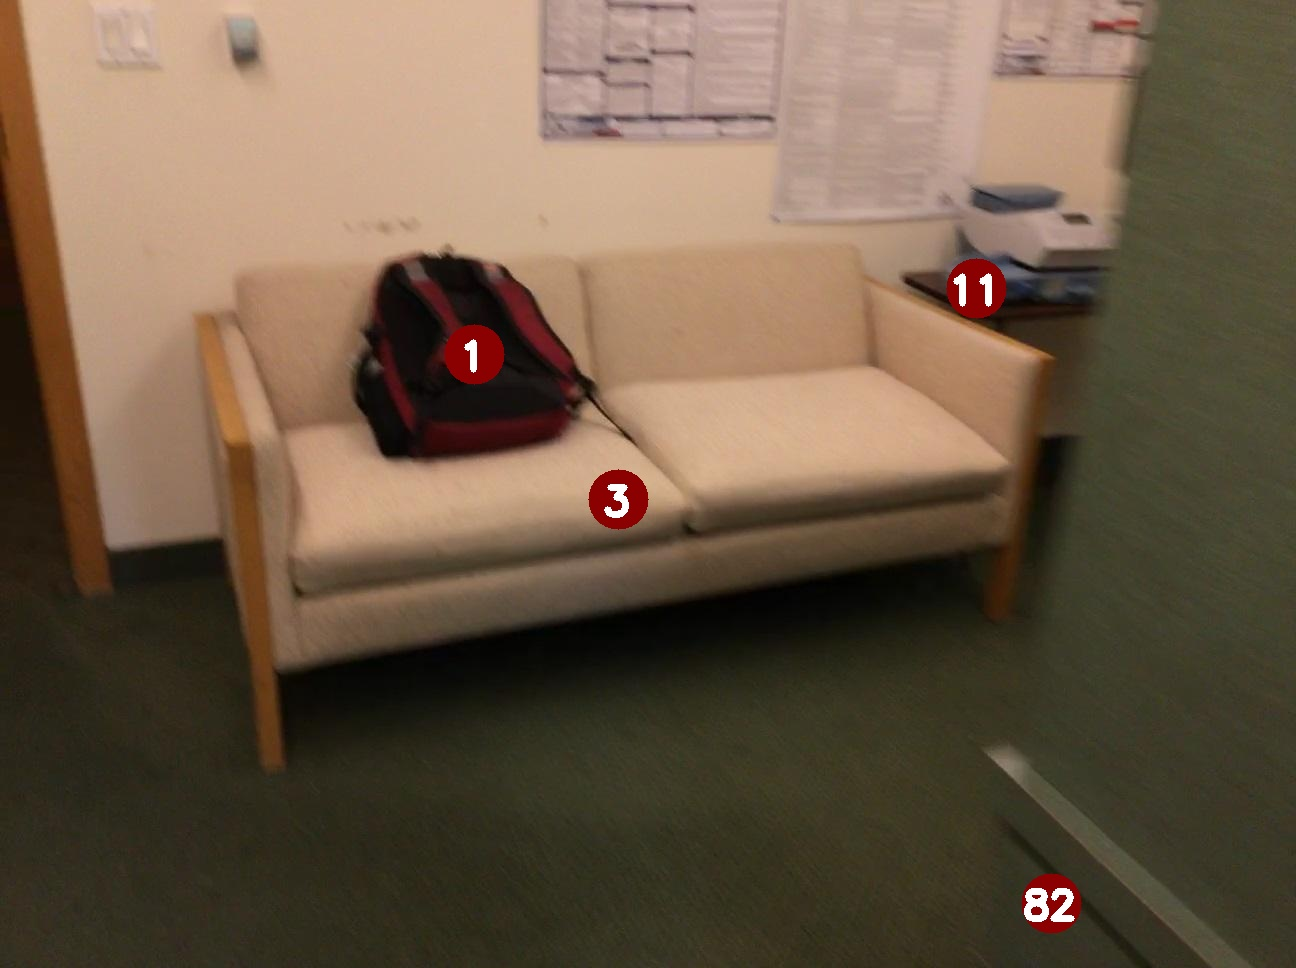} &
    \includegraphics[width=0.22\linewidth]{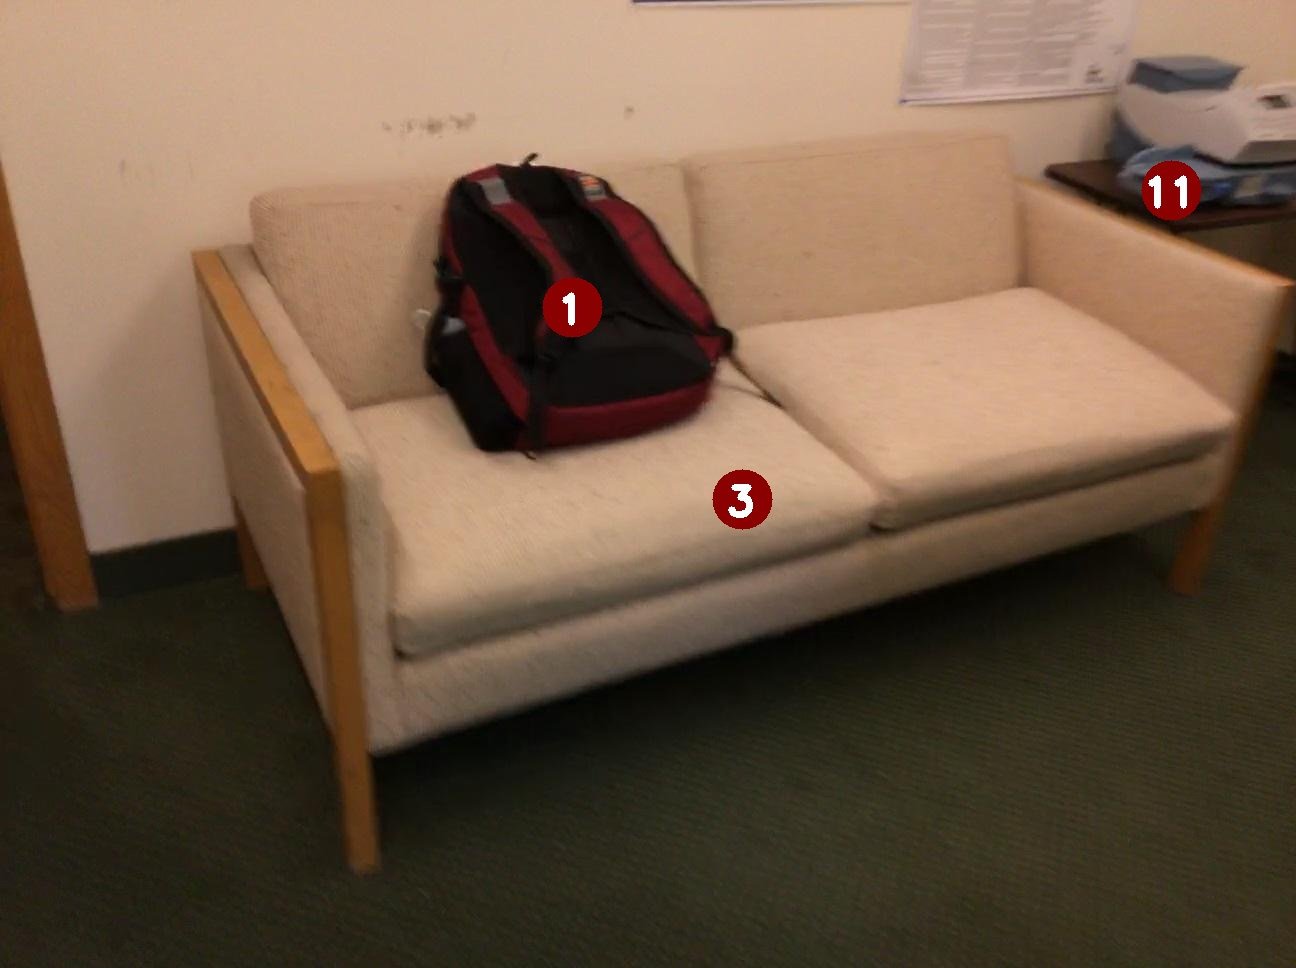} \\
    \vspace{0.1em} \\
    \includegraphics[width=0.22\linewidth]{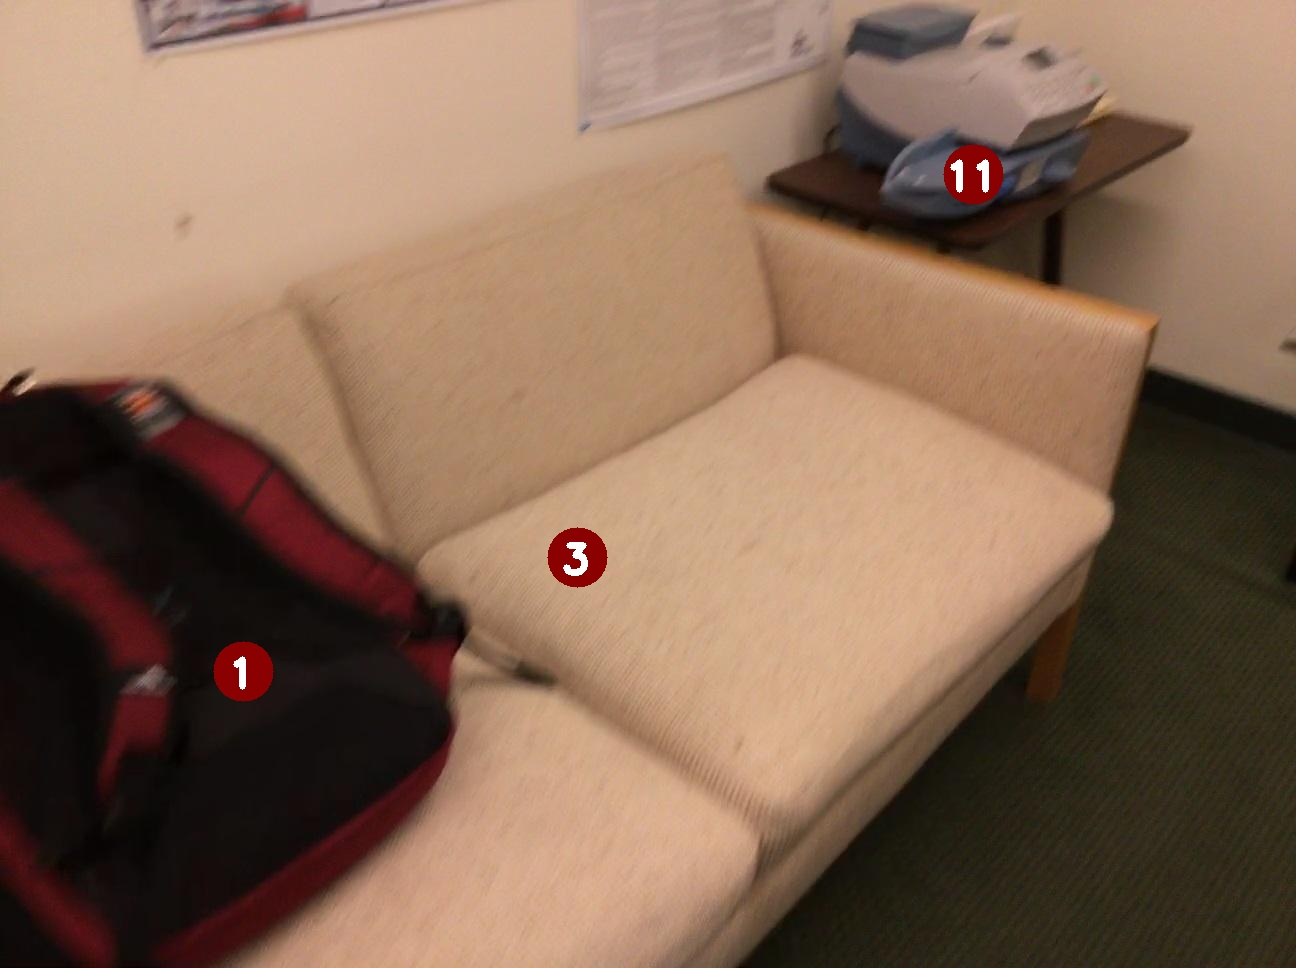} &
    \includegraphics[width=0.22\linewidth]{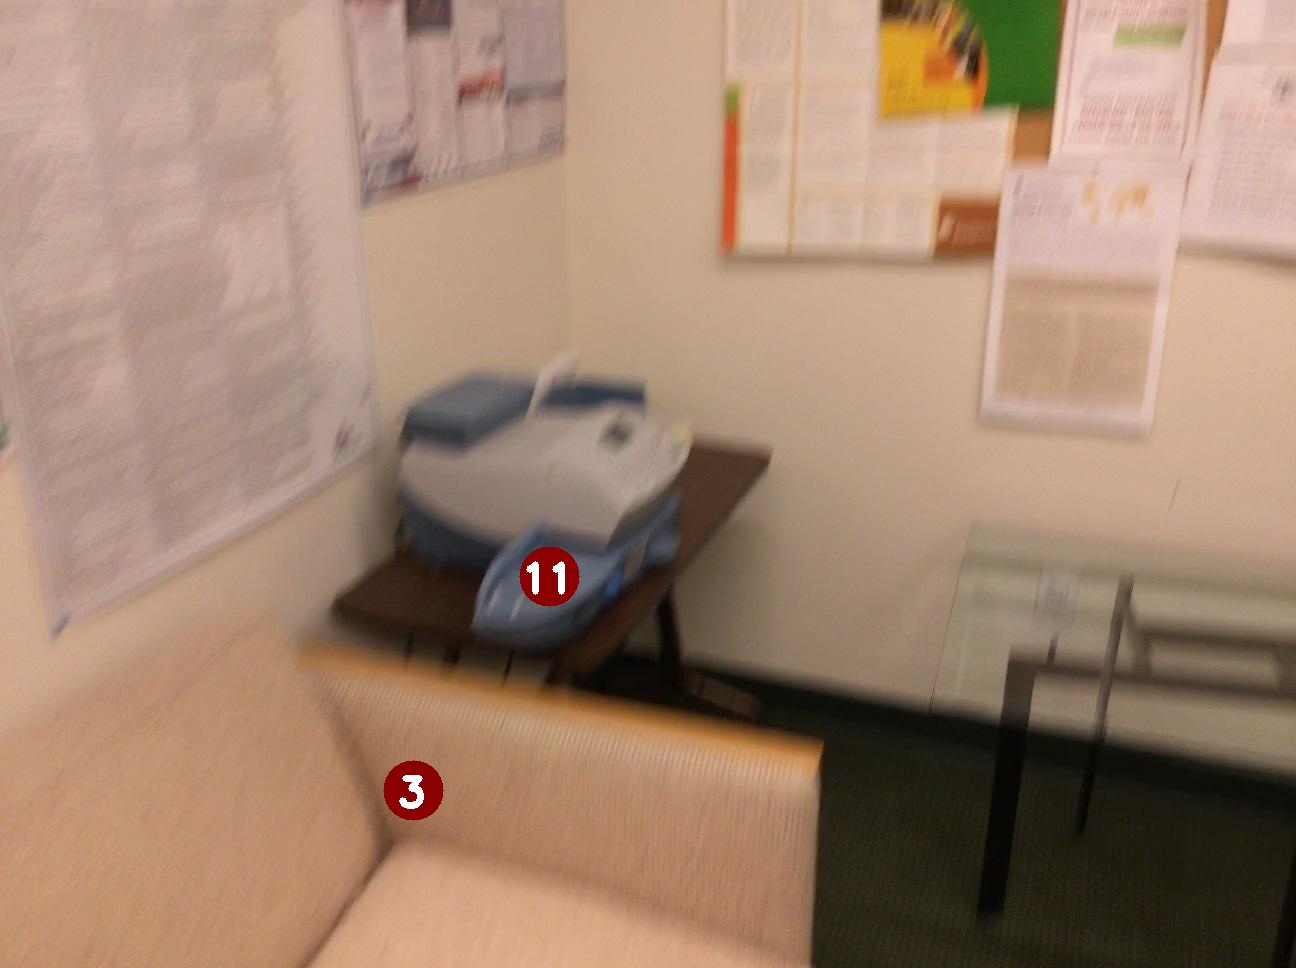} &
    \includegraphics[width=0.22\linewidth]{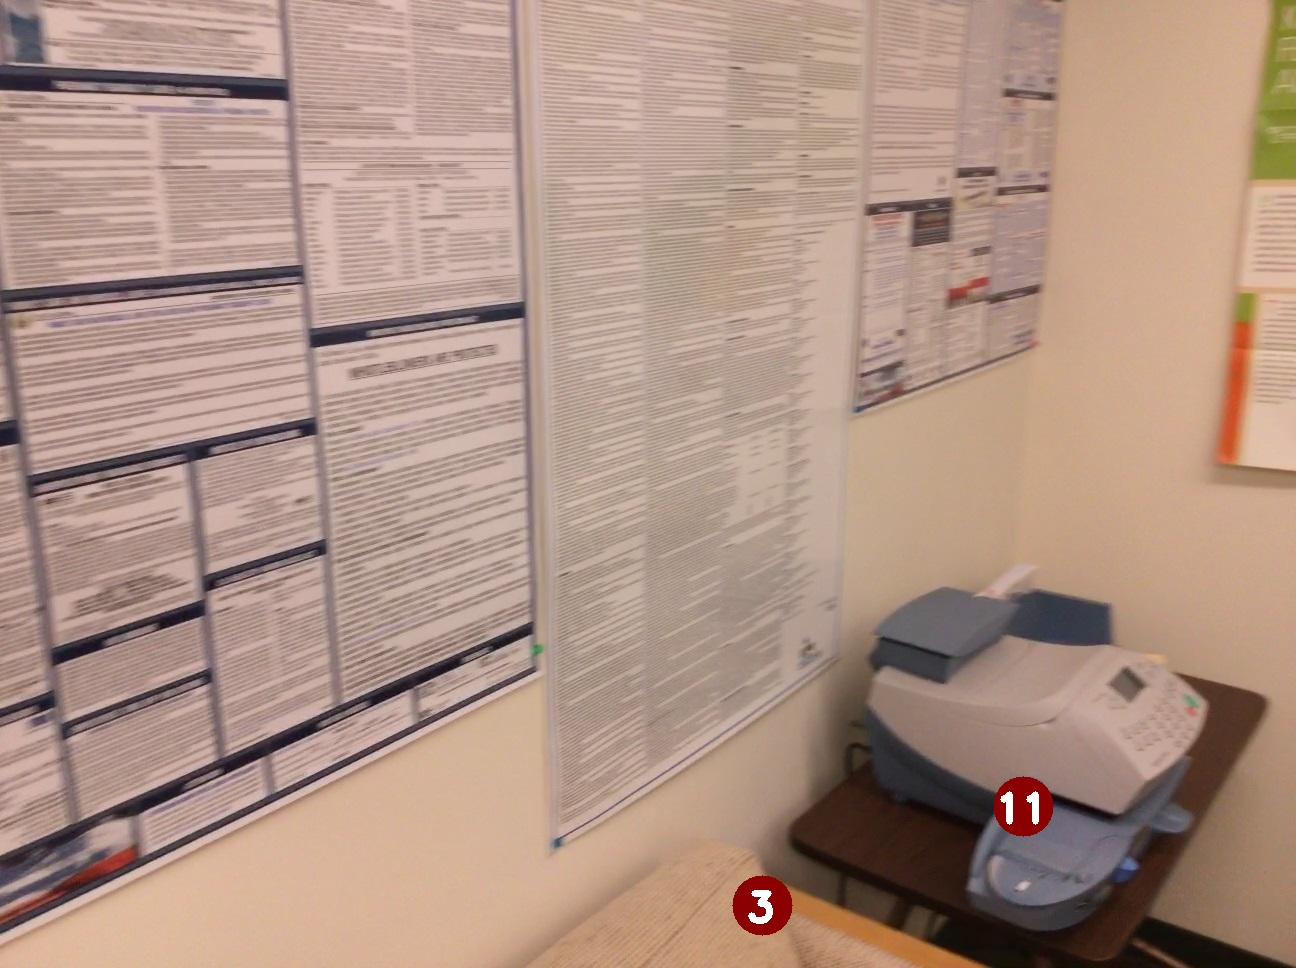} &
    \includegraphics[width=0.22\linewidth]{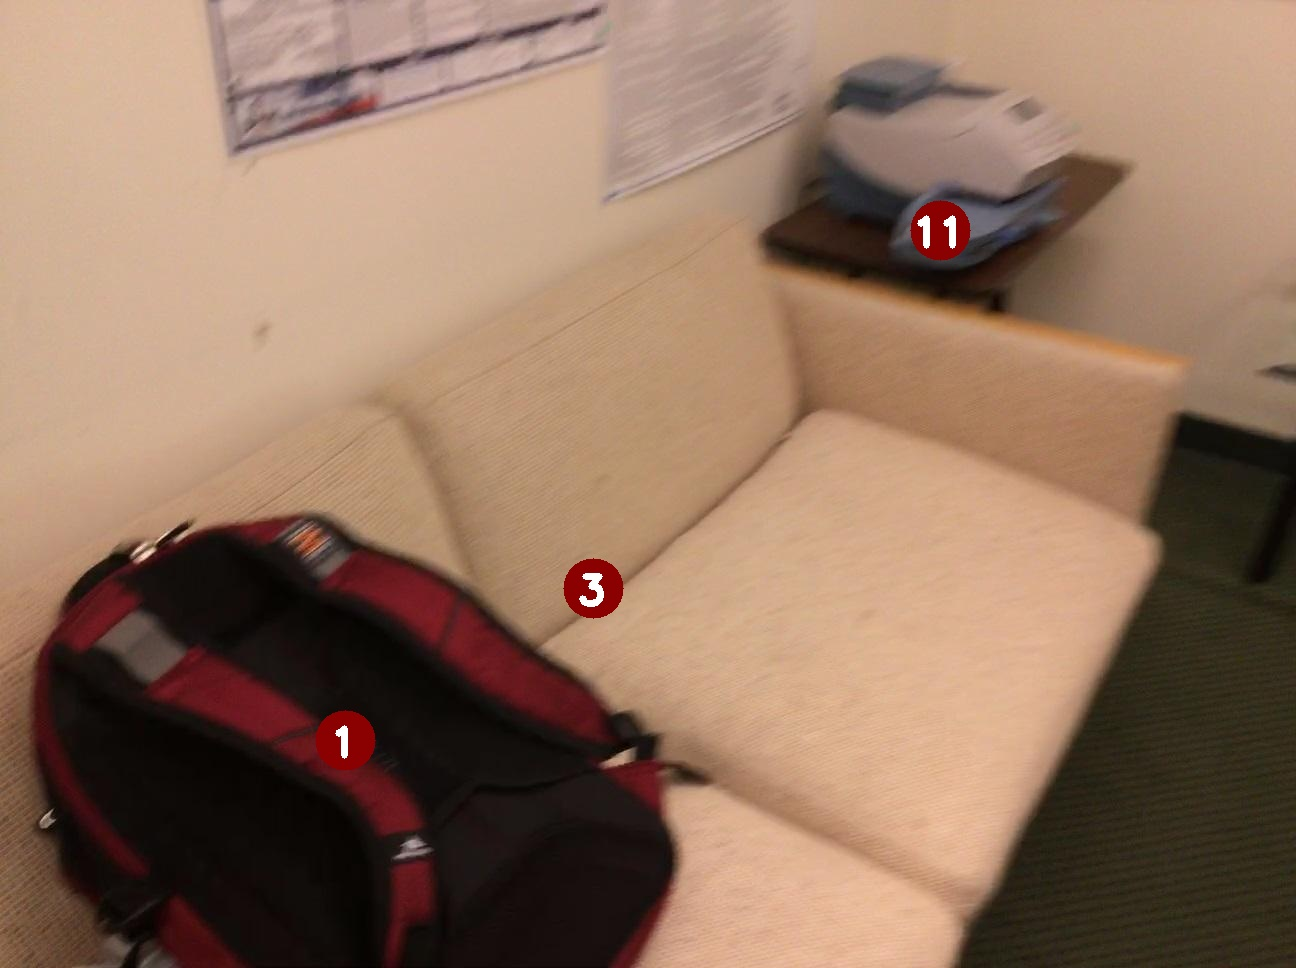} \\
    \textbf{Question}: & \multicolumn{3}{p{0.72\linewidth}}{Describe the visual traits of <OBJ003> first, then elucidate its spatial arrangements in relation to neighboring elements.} \\
    \midrule
    % \textbf{Ground Truth 1}: & \multicolumn{3}{p{0.72\linewidth}}{This sofa is tan. It is smooth.} \\
    % \textbf{Ground Truth 2}: & \multicolumn{3}{p{0.72\linewidth}}{It is a cream couch. The cream couch is sitting at the front left of the room.} \\
    % \textbf{Ground Truth 3}: & \multicolumn{3}{p{0.72\linewidth}}{The couch is located along the left wall. There is a red and black backpack atop the couch.} \\
    % \textbf{Ground Truth 4}: & \multicolumn{3}{p{0.72\linewidth}}{This is a white couch. It is to the left of the table.} \\
    % \textbf{Ground Truth 5}: & \multicolumn{3}{p{0.72\linewidth}}{A small size compact couch. It is on the brown sofa.} \\
    % \midrule
    \textbf{Qwen2.5-VL}: & \multicolumn{3}{p{0.72\linewidth}}{
        The object is a \colorbox{red!20}{\textbf{mailbox}} with multiple compartments, each labeled with numbers. It is mounted on a green wall and has a rectangular shape with a grid-like structure. 
        The compartments appear to be filled with various items, possibly letters or packages. \newline
        In terms of spatial arrangement: \newline 
        - It is positioned against a green wall. \newline 
        - To the right of the mailbox is a \textbf{printer} (labeled as 44), which is placed on a desk. \newline 
        - Below the printer, there is a \textbf{trash bin} (labeled as 6). \newline 
        - To the left of the mailbox, there is a \textbf{desk} with a computer monitor.
    } \\
    \midrule
    \textbf{VeBrain}: & \multicolumn{3}{p{0.72\linewidth}}{This is a \colorbox{green!20}{white couch}. It is on the left side of the table and printer.} \\
    \bottomrule
    \end{tabular}
\end{table}

\begin{table}[ht]
    \centering
    \begin{tabular}{cccc}
    \toprule
    \multicolumn{4}{c}{\textbf{Spatial Reasoning: Example \#3 from Scan2Cap.}} \\
    \midrule
    \includegraphics[width=0.22\linewidth]{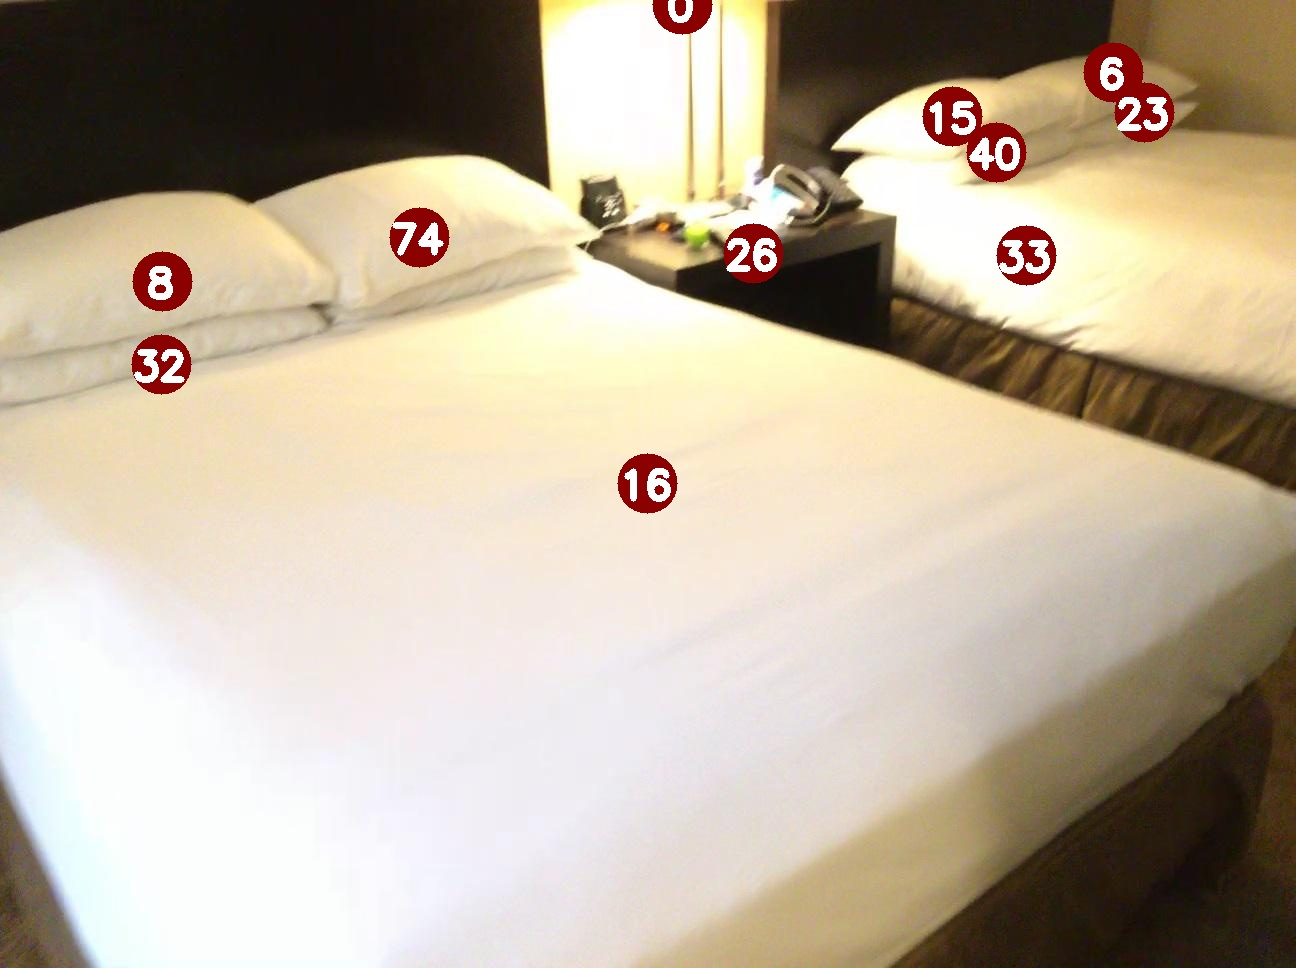} &
    \includegraphics[width=0.22\linewidth]{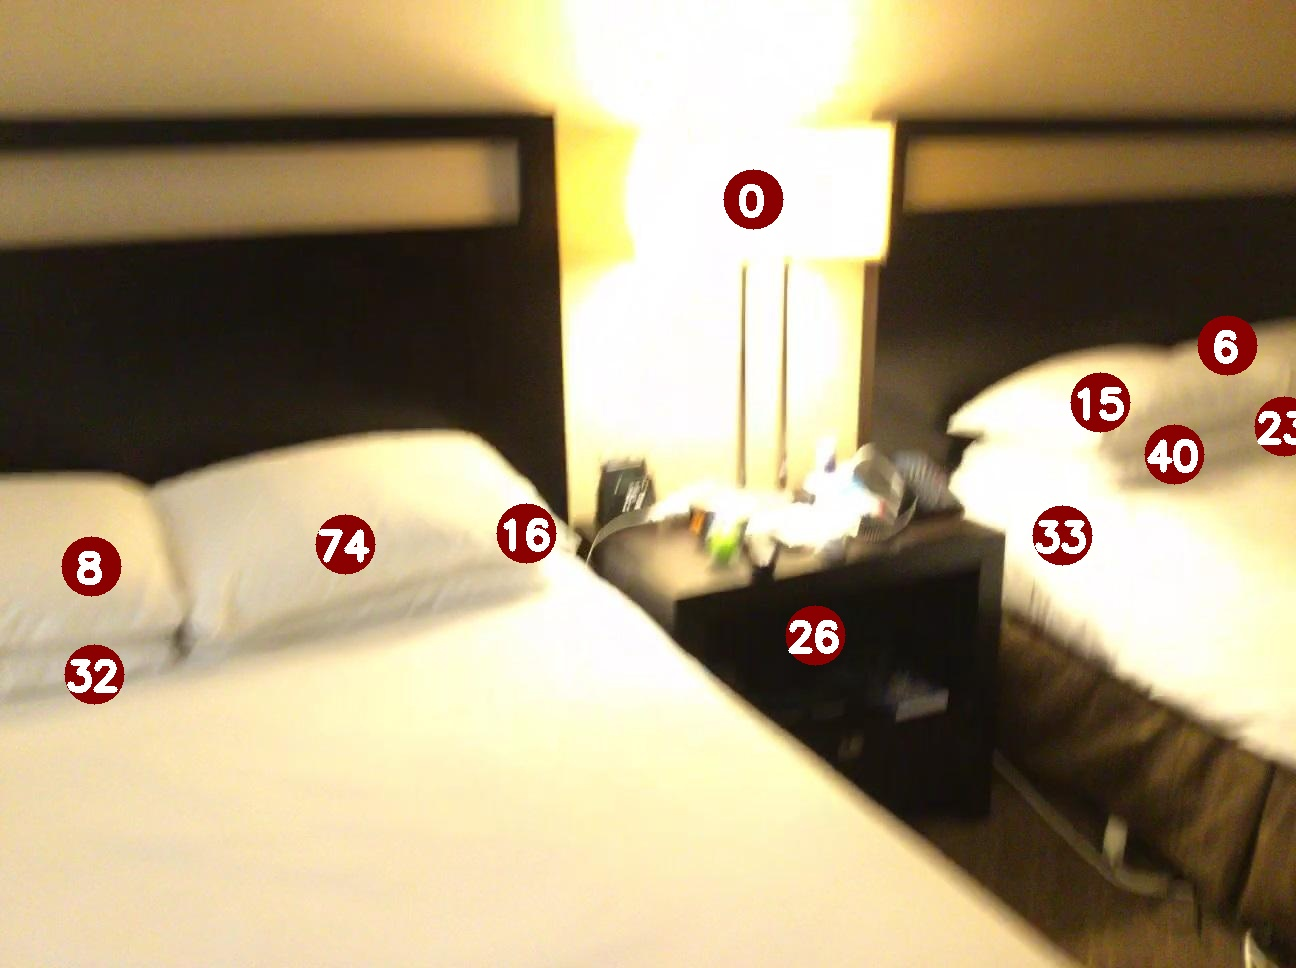} &
    \includegraphics[width=0.22\linewidth]{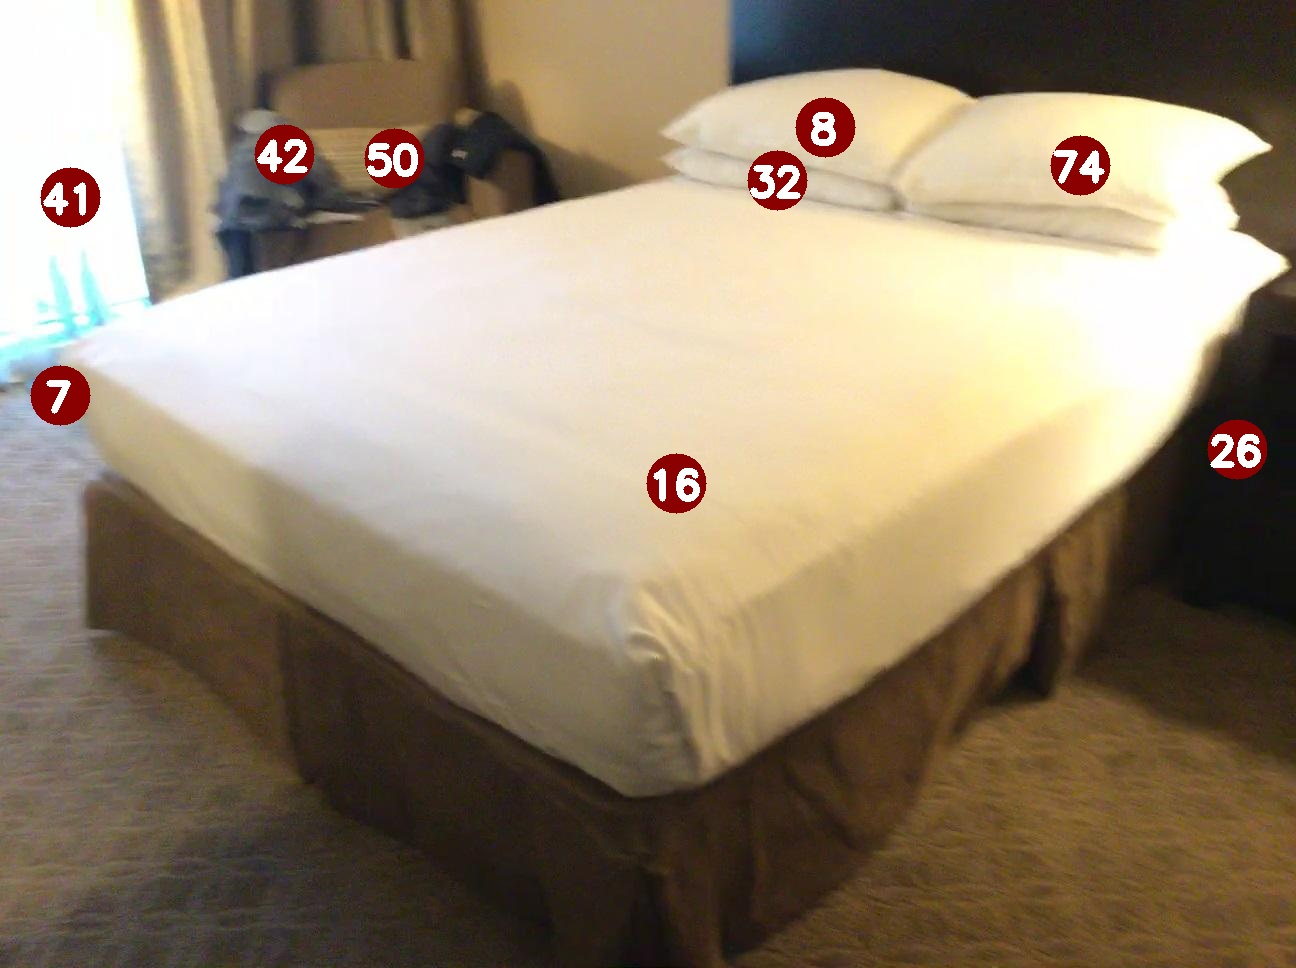} &
    \includegraphics[width=0.22\linewidth]{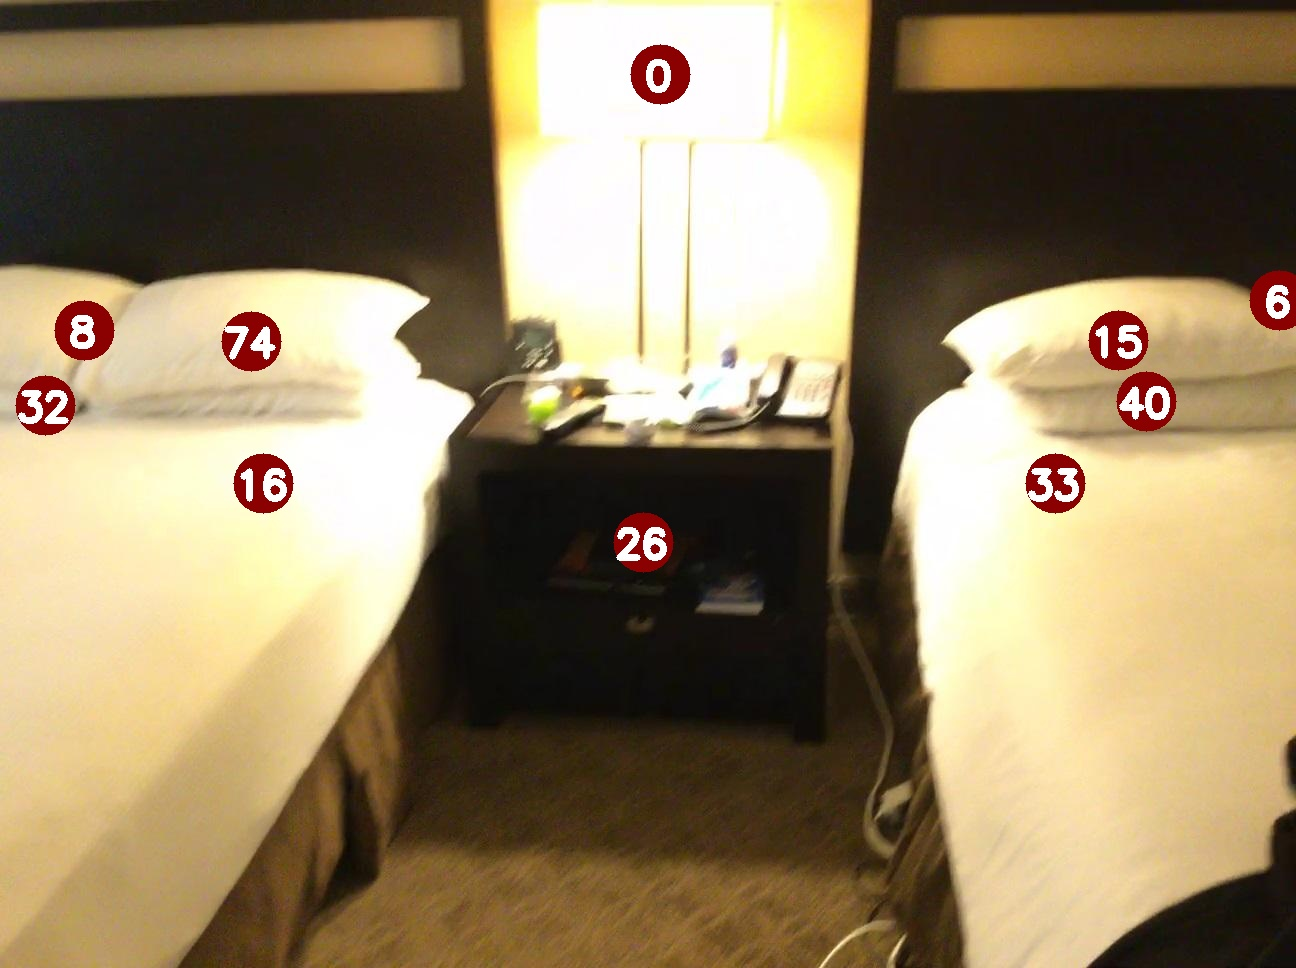} \\
    \vspace{0.1em} \\
    \includegraphics[width=0.22\linewidth]{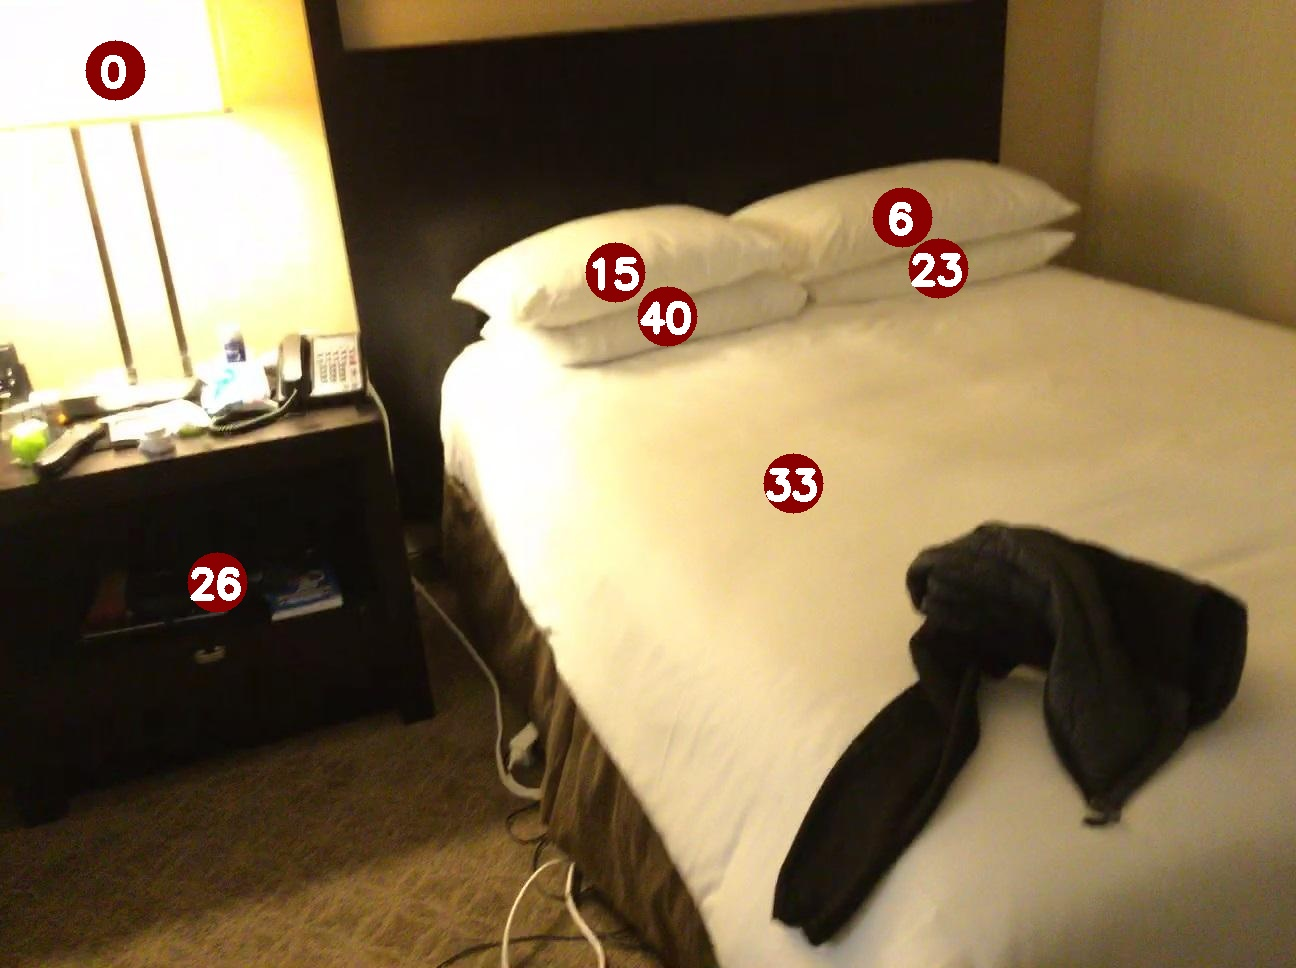} &
    \includegraphics[width=0.22\linewidth]{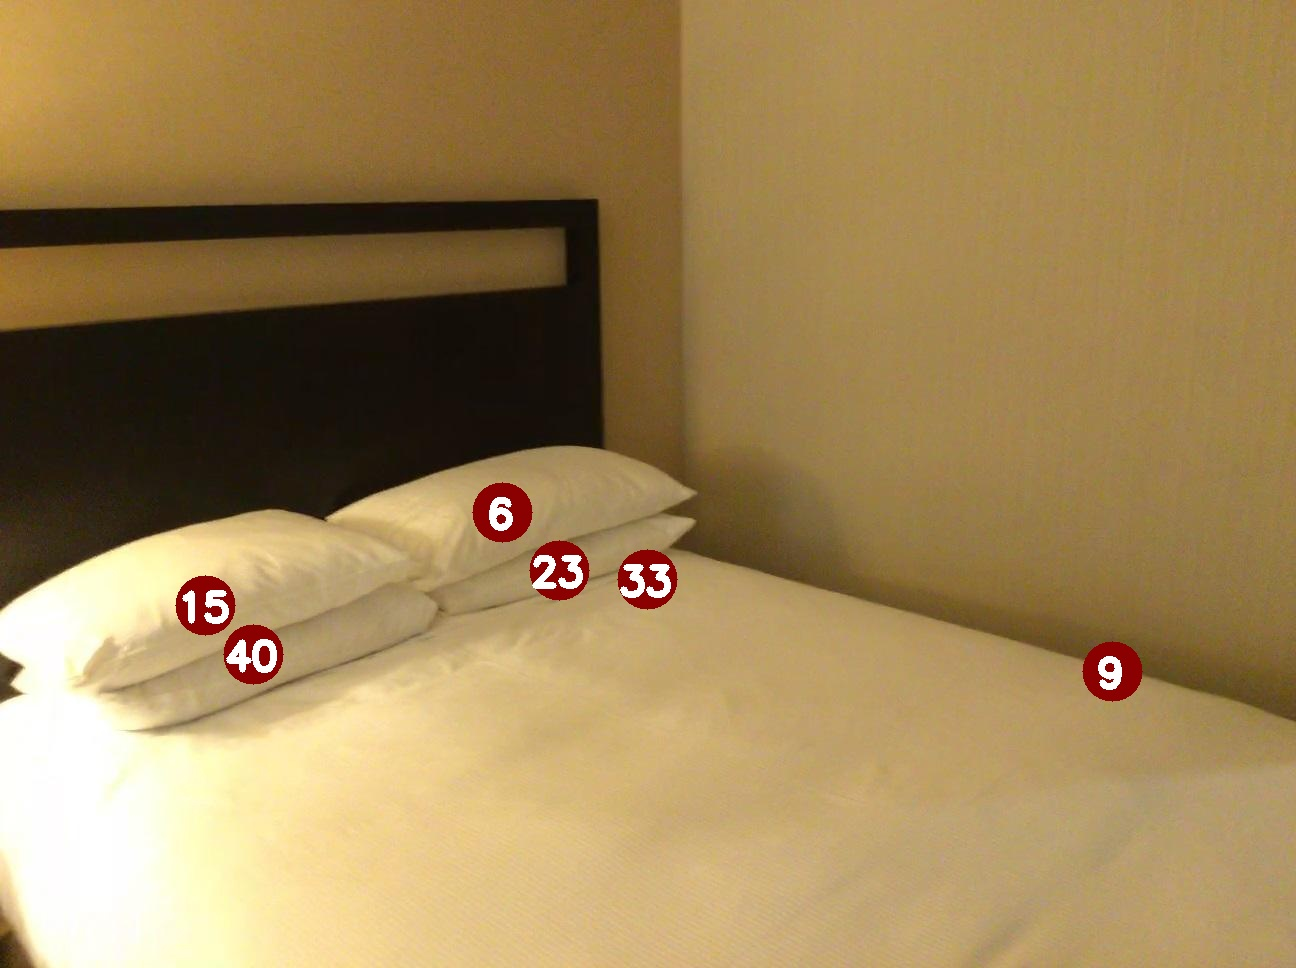} &
    \includegraphics[width=0.22\linewidth]{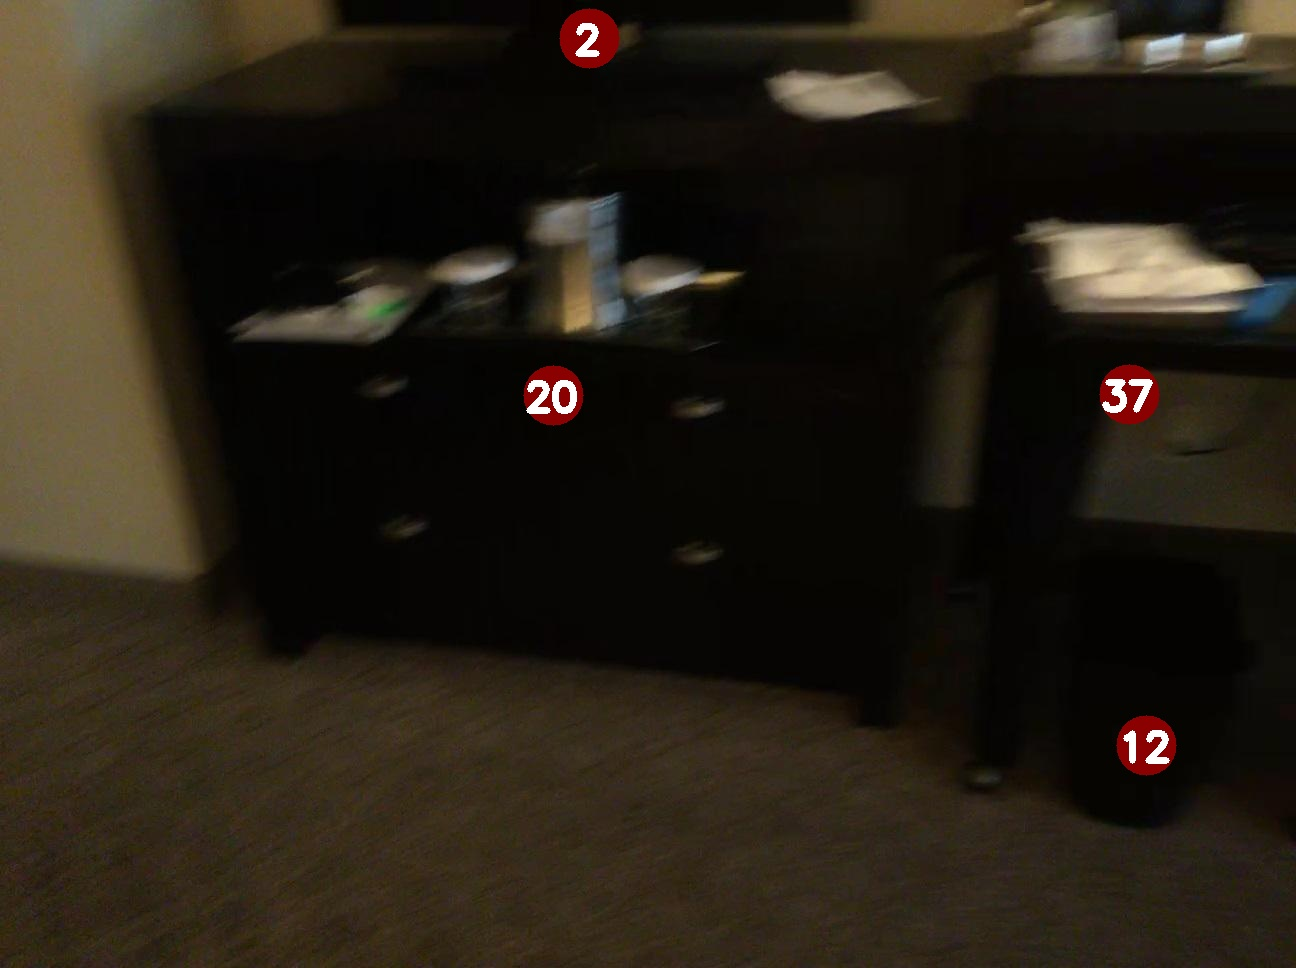} &
    \includegraphics[width=0.22\linewidth]{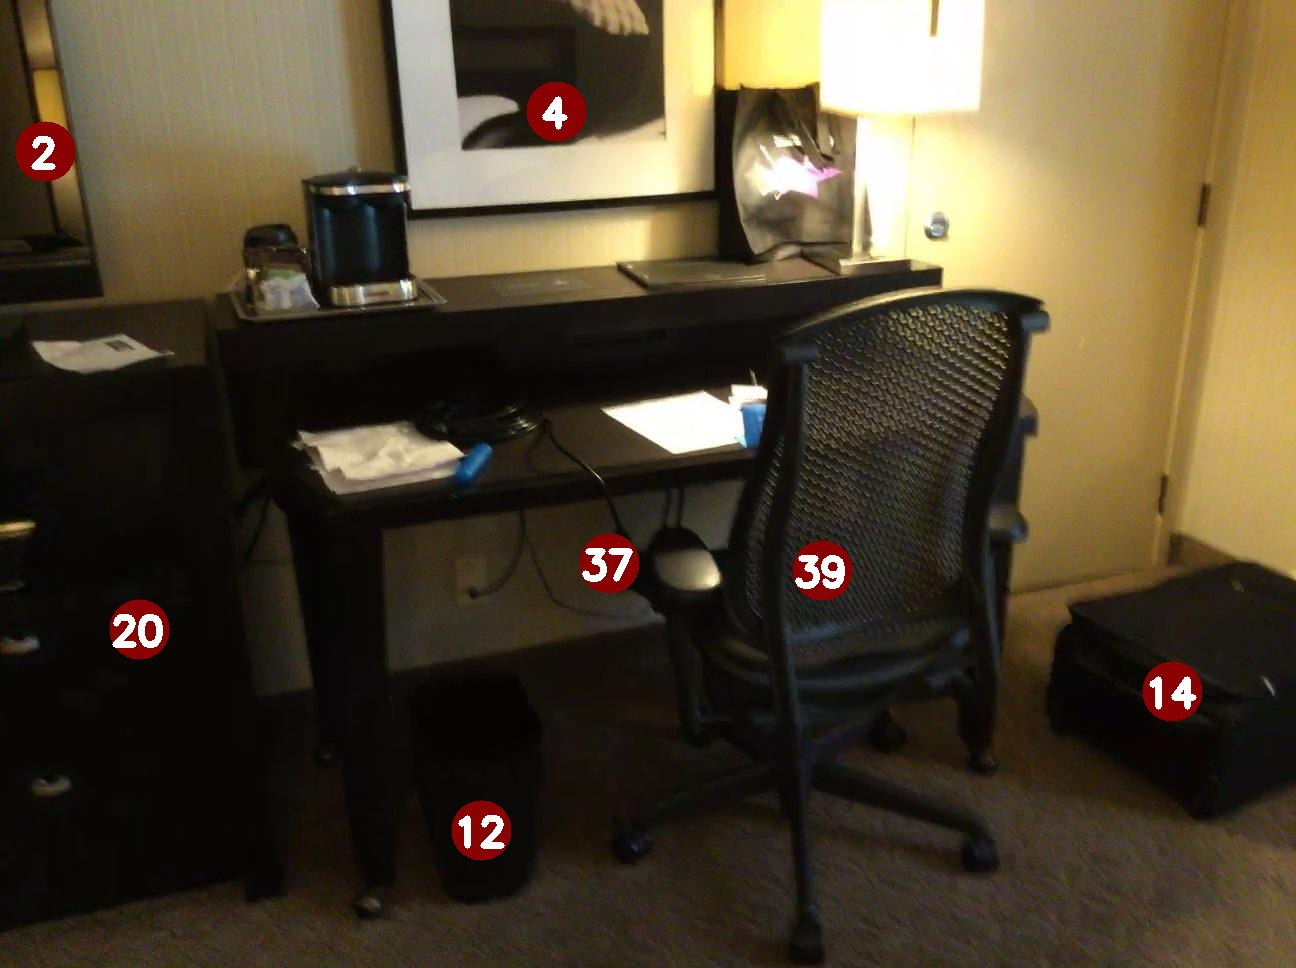} \\
    \textbf{Question}: & \multicolumn{3}{p{0.72\linewidth}}{Start by articulating the outward features of the <OBJ033>, then transition into its spatial alignment within the broader scene.} \\
    \midrule
    \textbf{Qwen2.5-VL}: & \multicolumn{3}{p{0.72\linewidth}}{The <OBJ033> is a black \colorbox{red!20}{cabinet} with a dark brown top and silver handles. It has three drawers, each with a silver handle. The cabinet is positioned against a wall, with a white door to its left and a white wall behind it. There is a black chair with a white cushion in front of the cabinet.} \\
    \midrule
    \textbf{VeBrain}: & \multicolumn{3}{p{0.72\linewidth}}{This is a \colorbox{green!20}{bed} with white sheets. It is to the right of a nightstand.} \\
    \bottomrule
    \end{tabular}
\end{table}

\begin{table}[ht]
    \centering
    \begin{tabular}{cccc}
    \toprule
    \multicolumn{4}{c}{\textbf{Spatial Reasoning: Example \#4 from ScanQA.}} \\
    \midrule
    \includegraphics[width=0.22\linewidth]{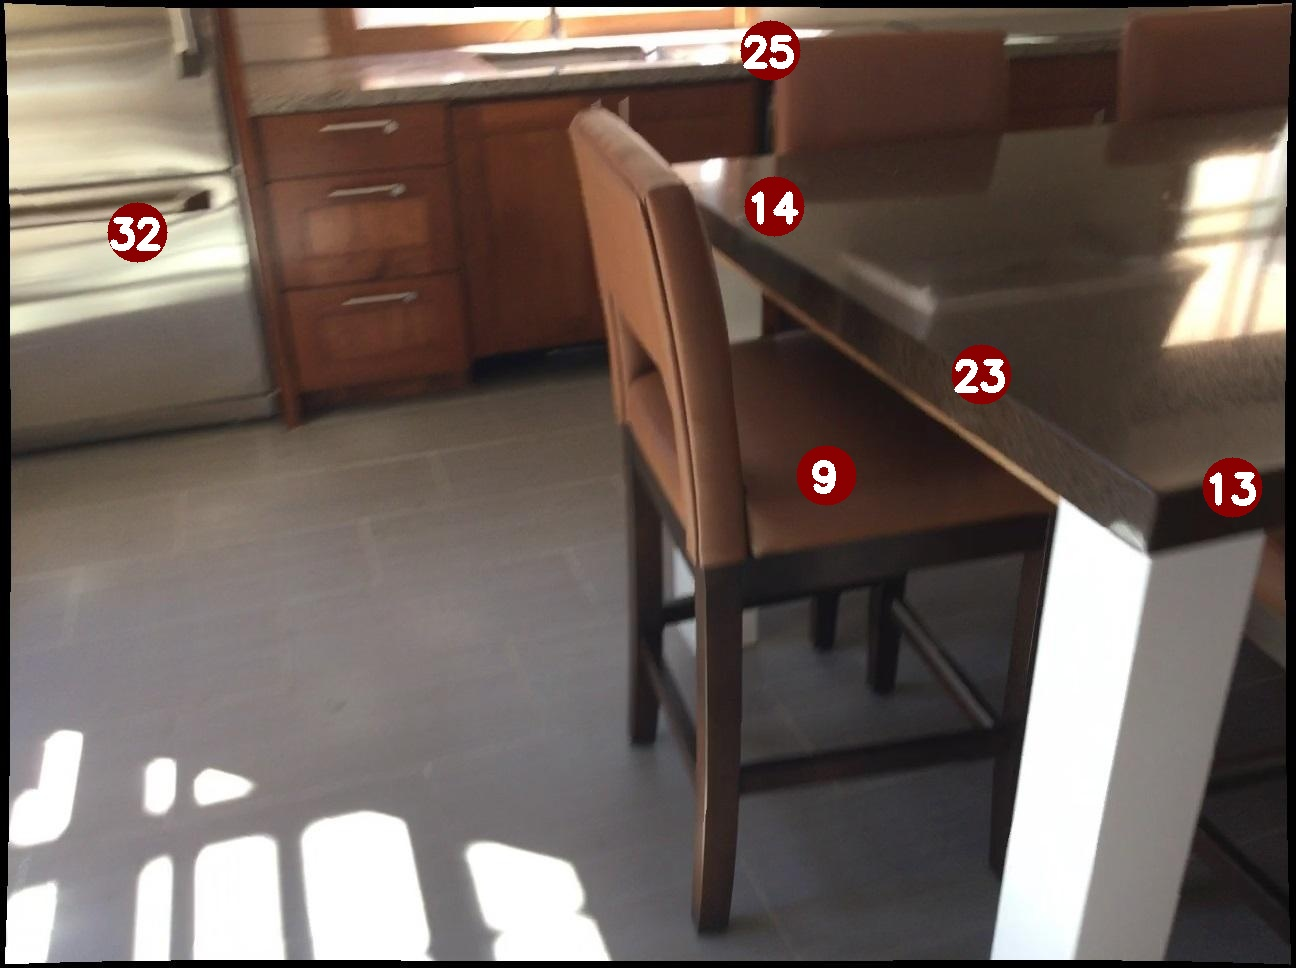} &
    \includegraphics[width=0.22\linewidth]{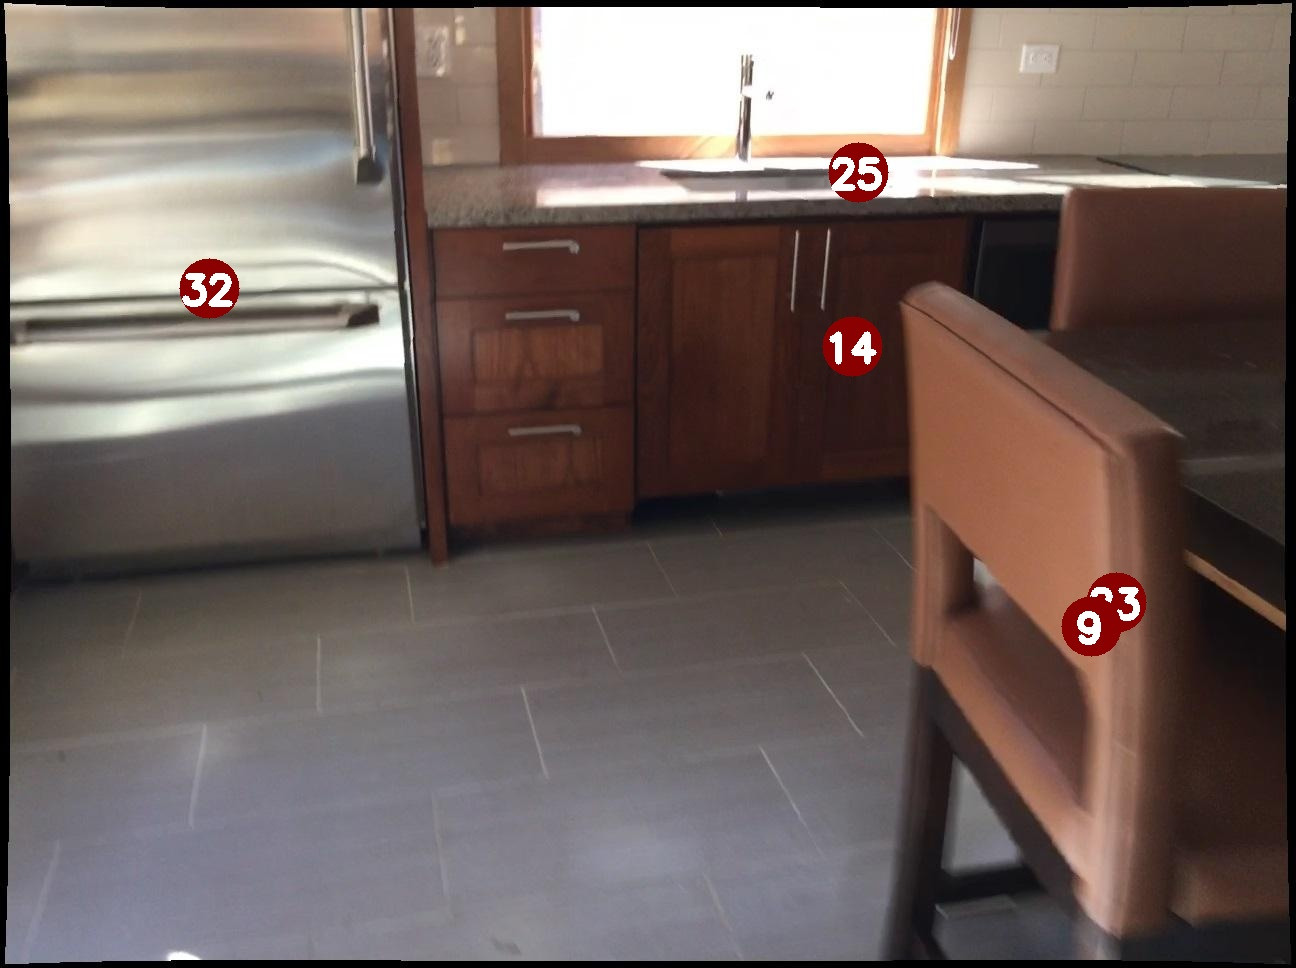} &
    \includegraphics[width=0.22\linewidth]{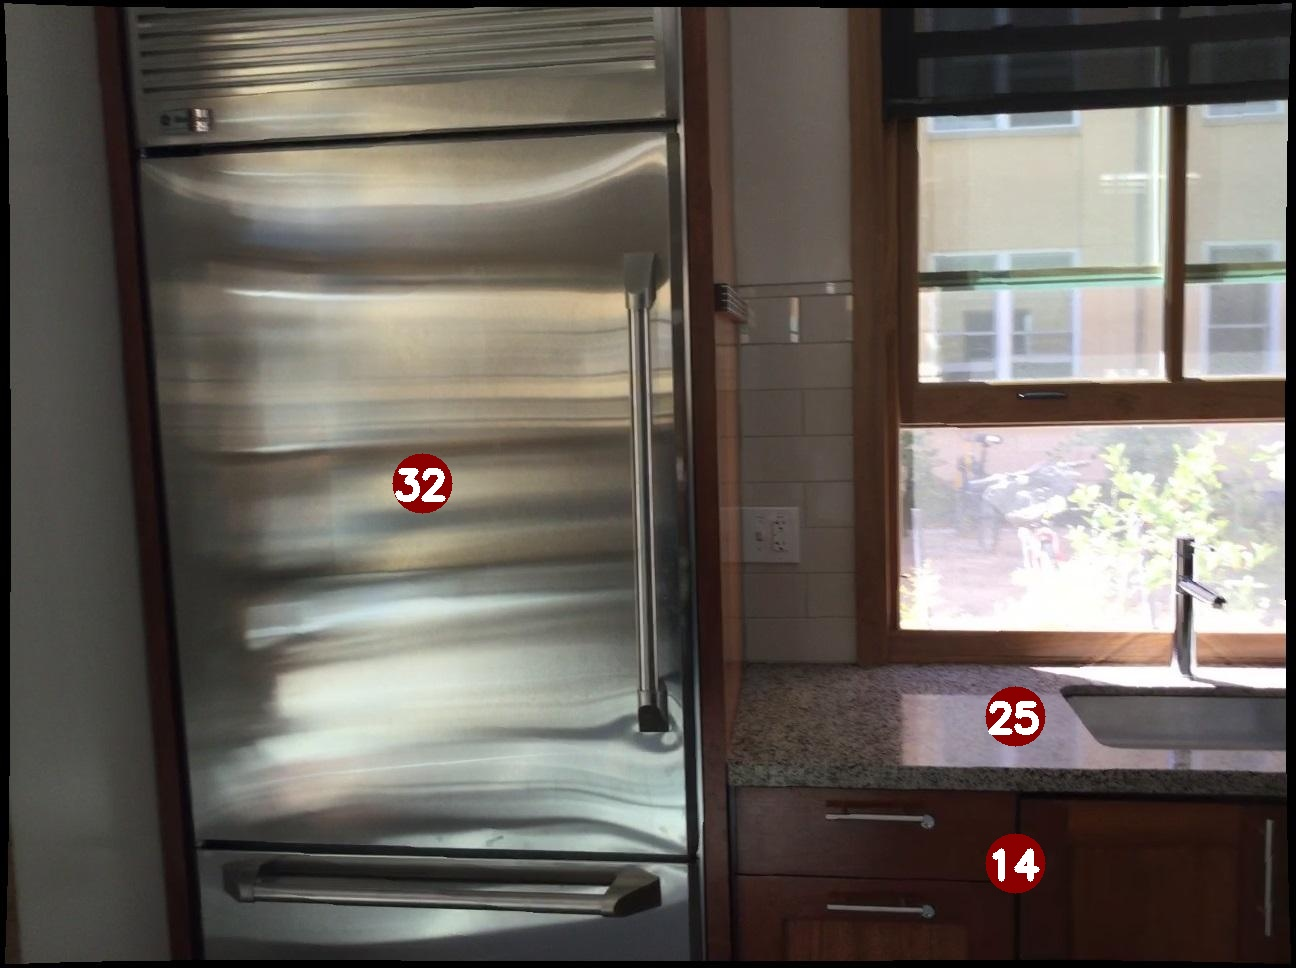} &
    \includegraphics[width=0.22\linewidth]{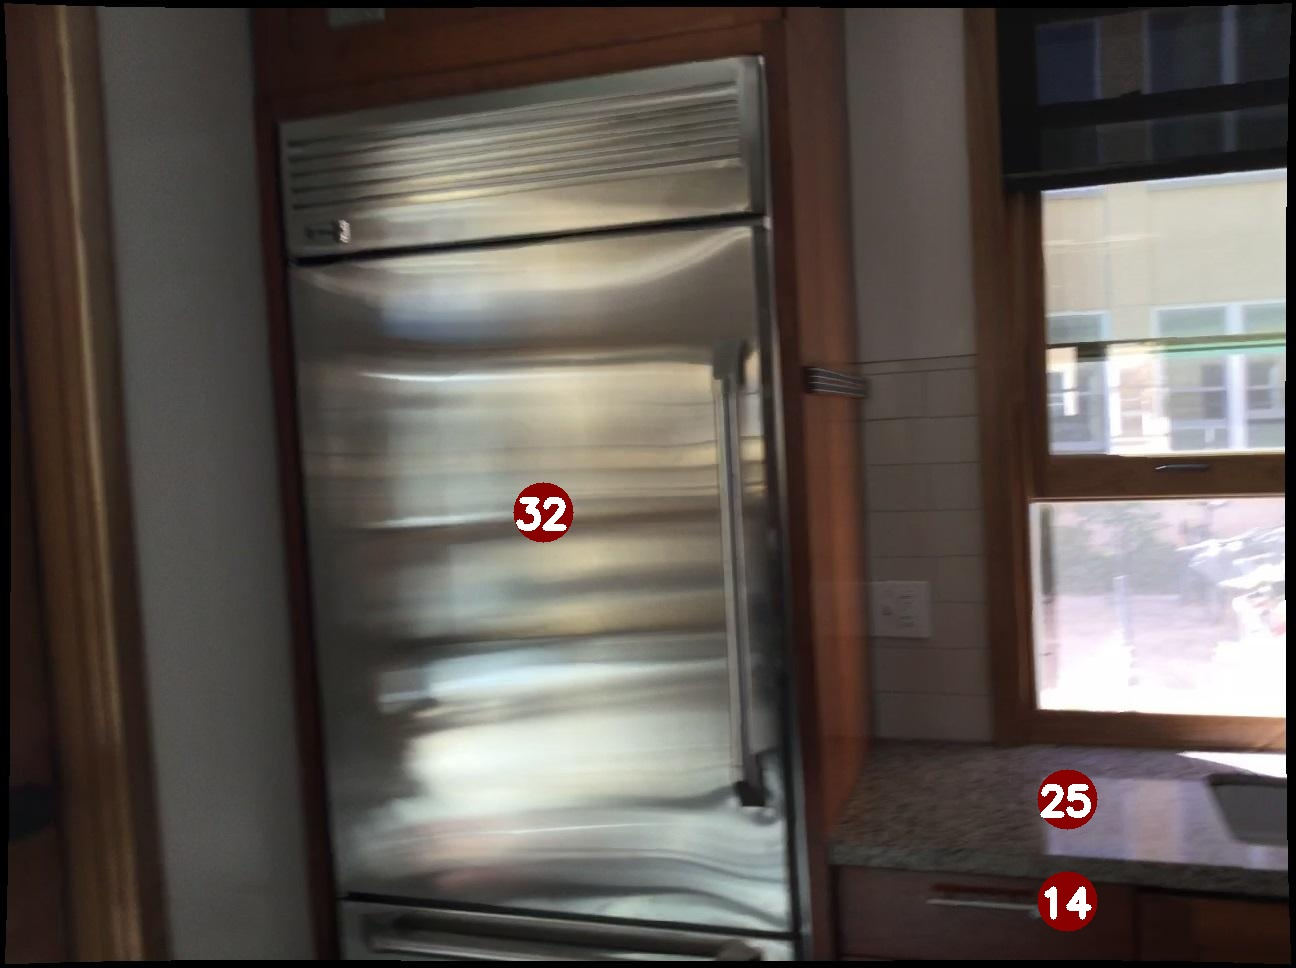} \\
    \vspace{0.1em} \\
    \includegraphics[width=0.22\linewidth]{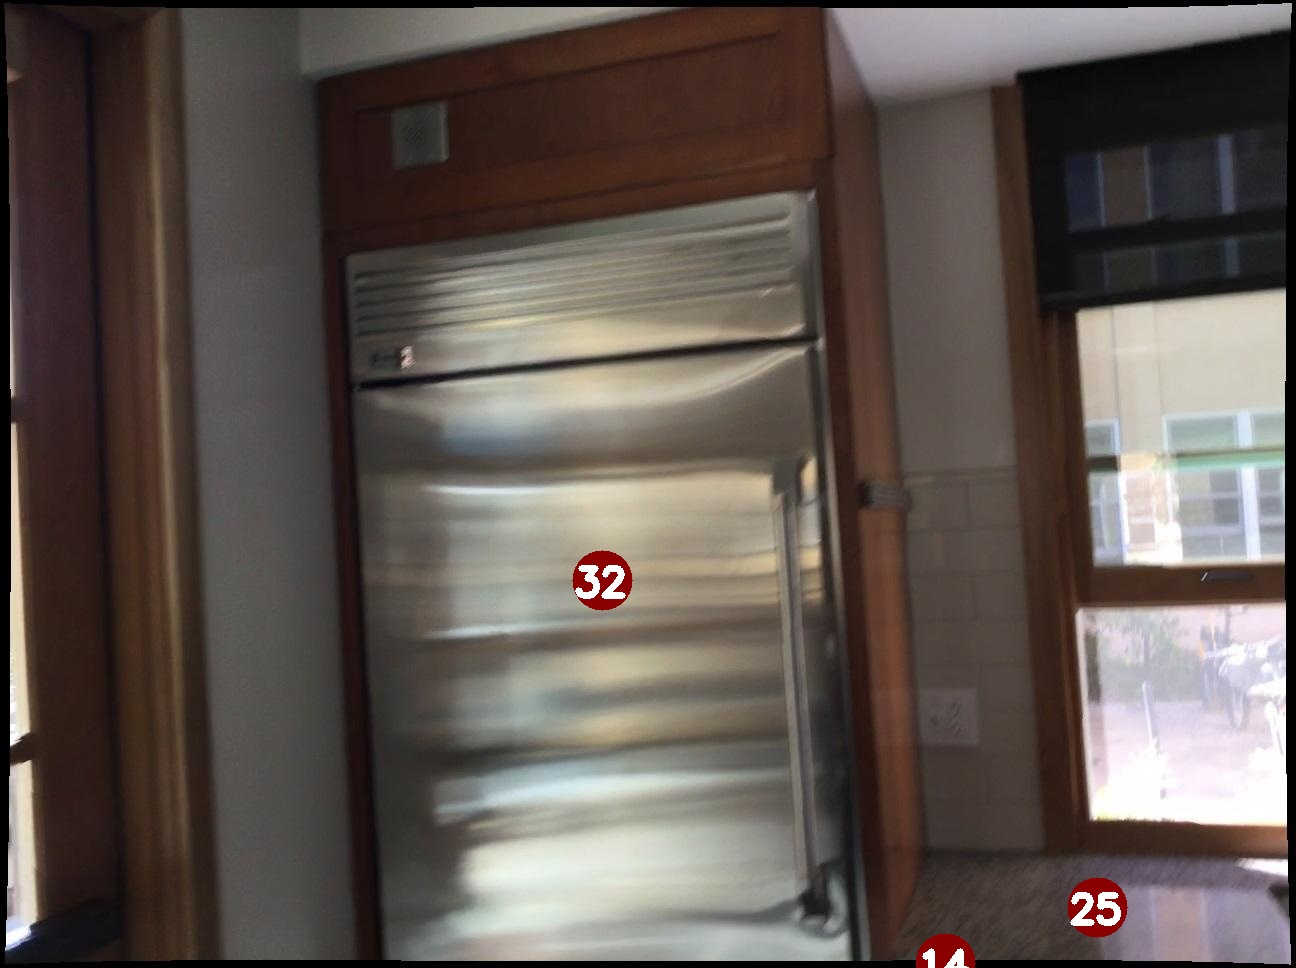} &
    \includegraphics[width=0.22\linewidth]{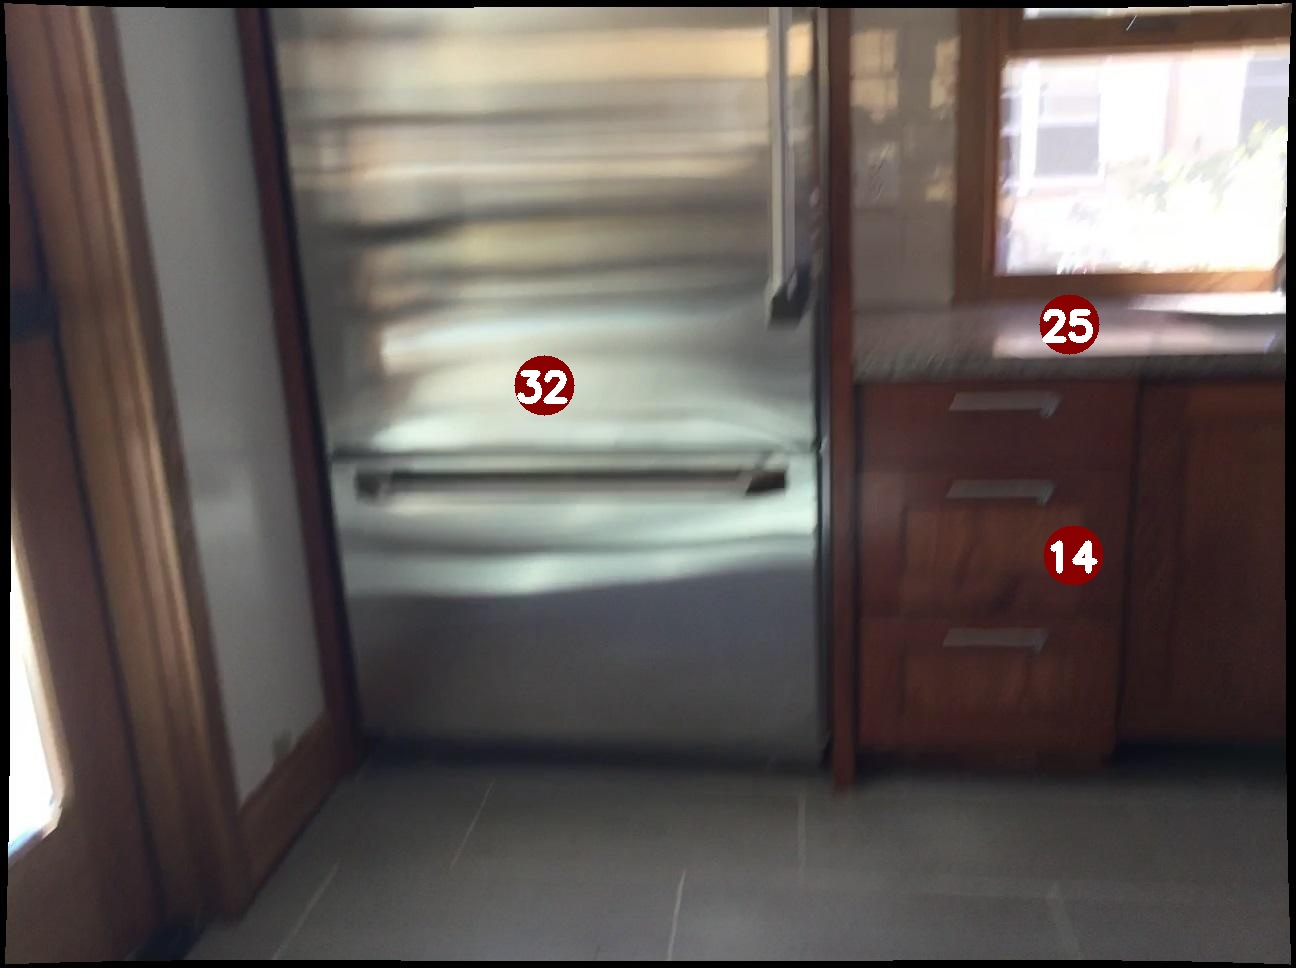} &
    \includegraphics[width=0.22\linewidth]{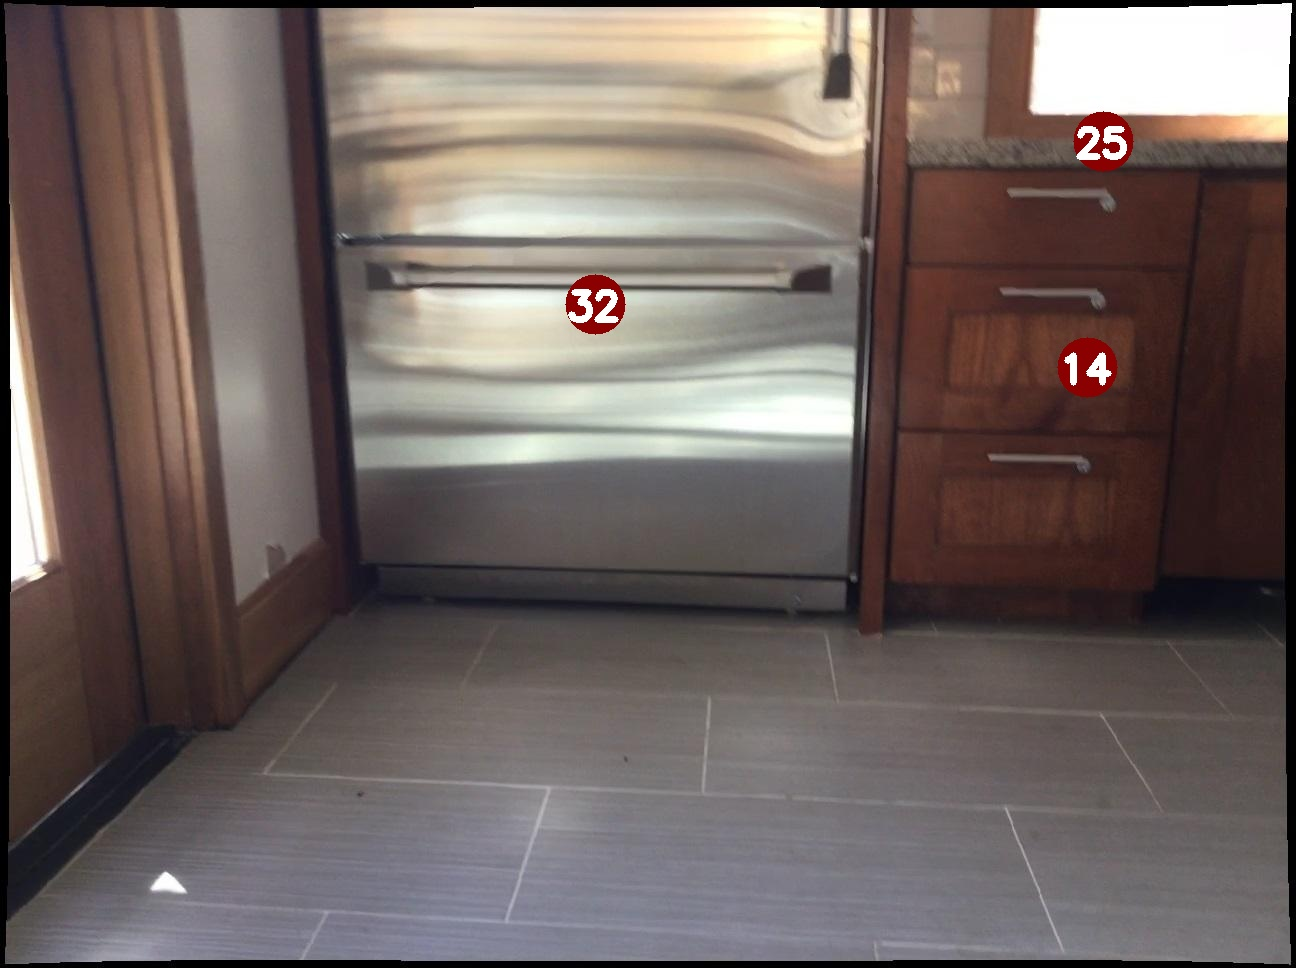} &
    \includegraphics[width=0.22\linewidth]{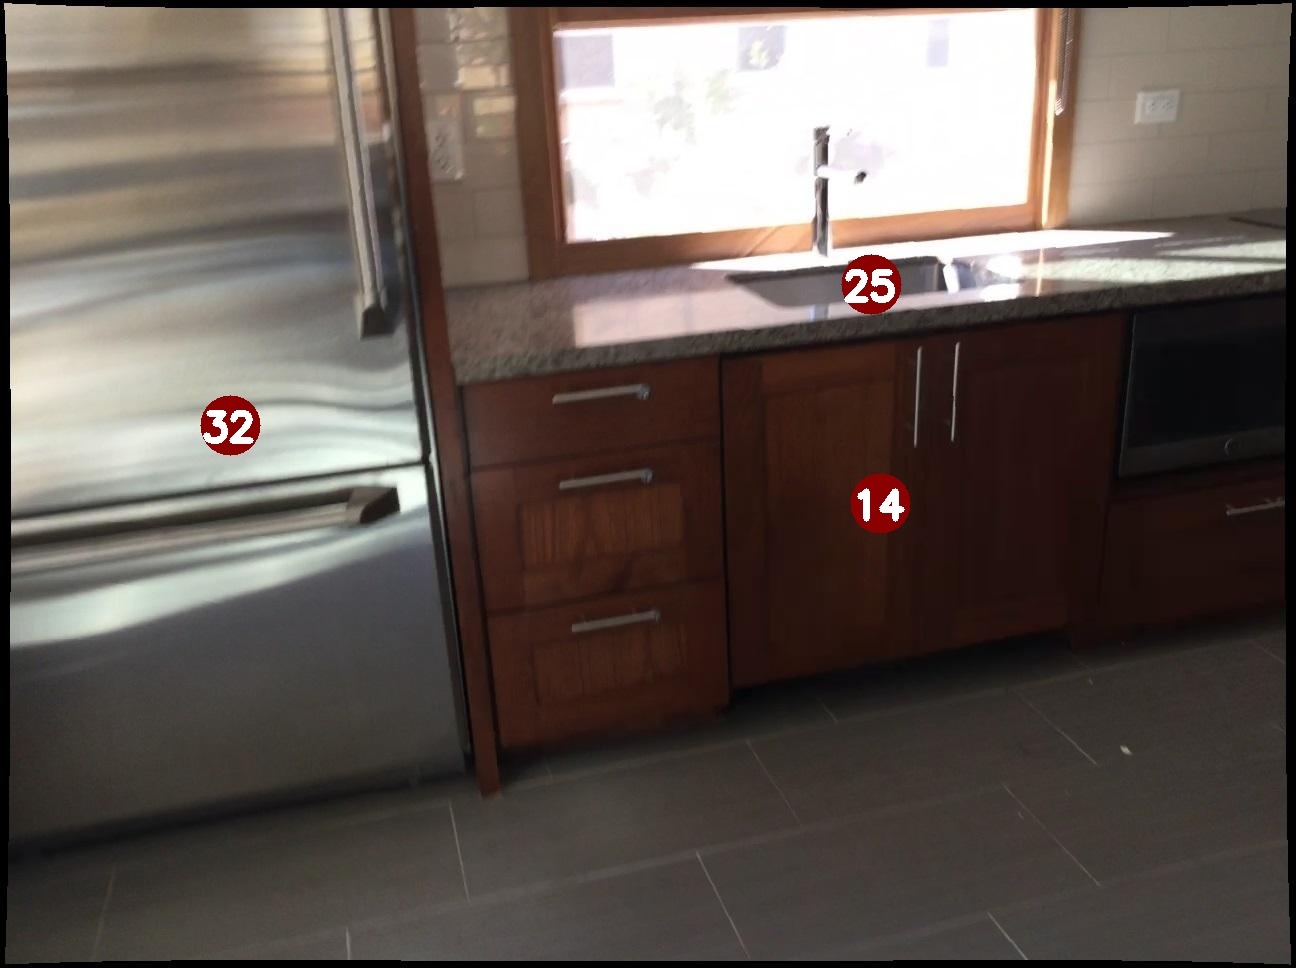} \\
    \textbf{Question}: & \multicolumn{3}{p{0.72\linewidth}}{What shape is the refrigerator on the left of a kitchen counter? Answer the question using a single word or phrase.} \\
    \midrule
    \textbf{Qwen2.5-VL}: & \multicolumn{3}{p{0.72\linewidth}}{\colorbox{red!20}{twin}} \\
    \midrule
    \textbf{VeBrain}: & \multicolumn{3}{p{0.72\linewidth}}{\colorbox{green!20}{Rectangular}} \\
    \bottomrule
    \end{tabular}
\end{table}

\begin{table}[ht]
    \centering
    \begin{tabular}{cccc}
    \toprule
    \multicolumn{4}{c}{\textbf{Spatial Reasoning: Example \#5 from ScanRefer.}} \\
    \midrule
    \includegraphics[width=0.22\linewidth]{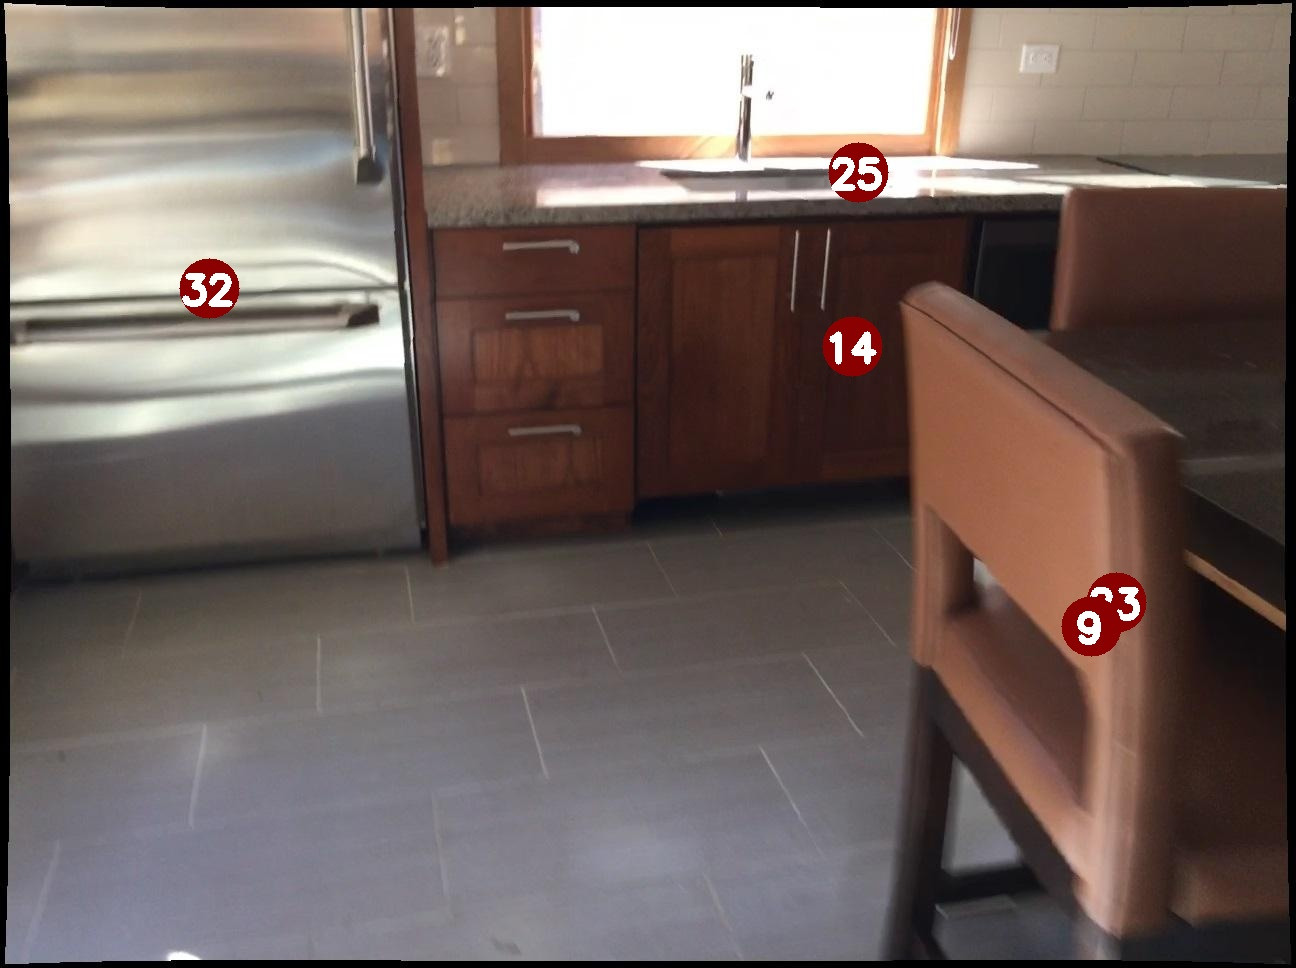} &
    \includegraphics[width=0.22\linewidth]{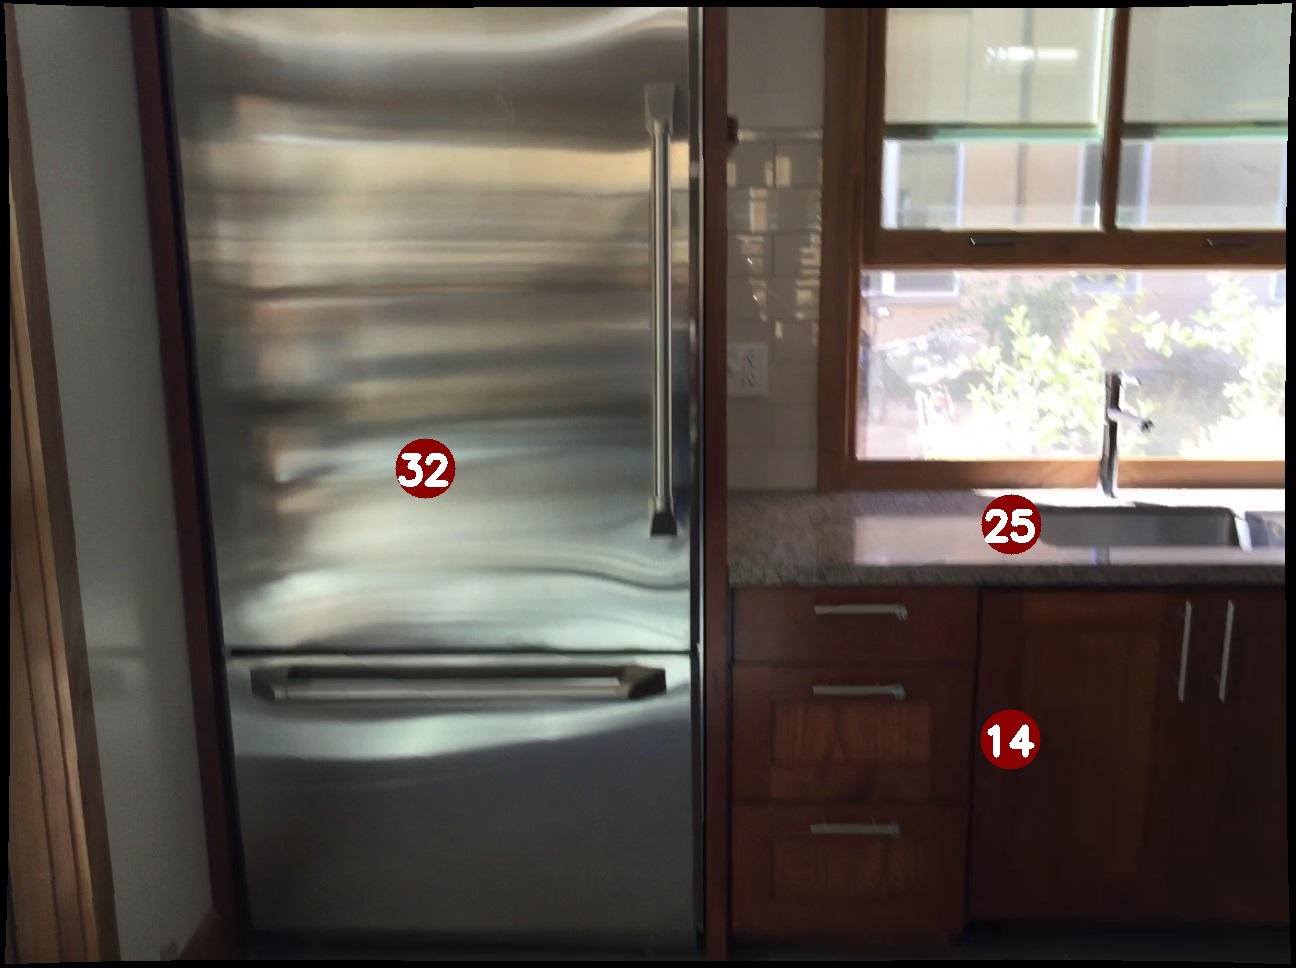} &
    \includegraphics[width=0.22\linewidth]{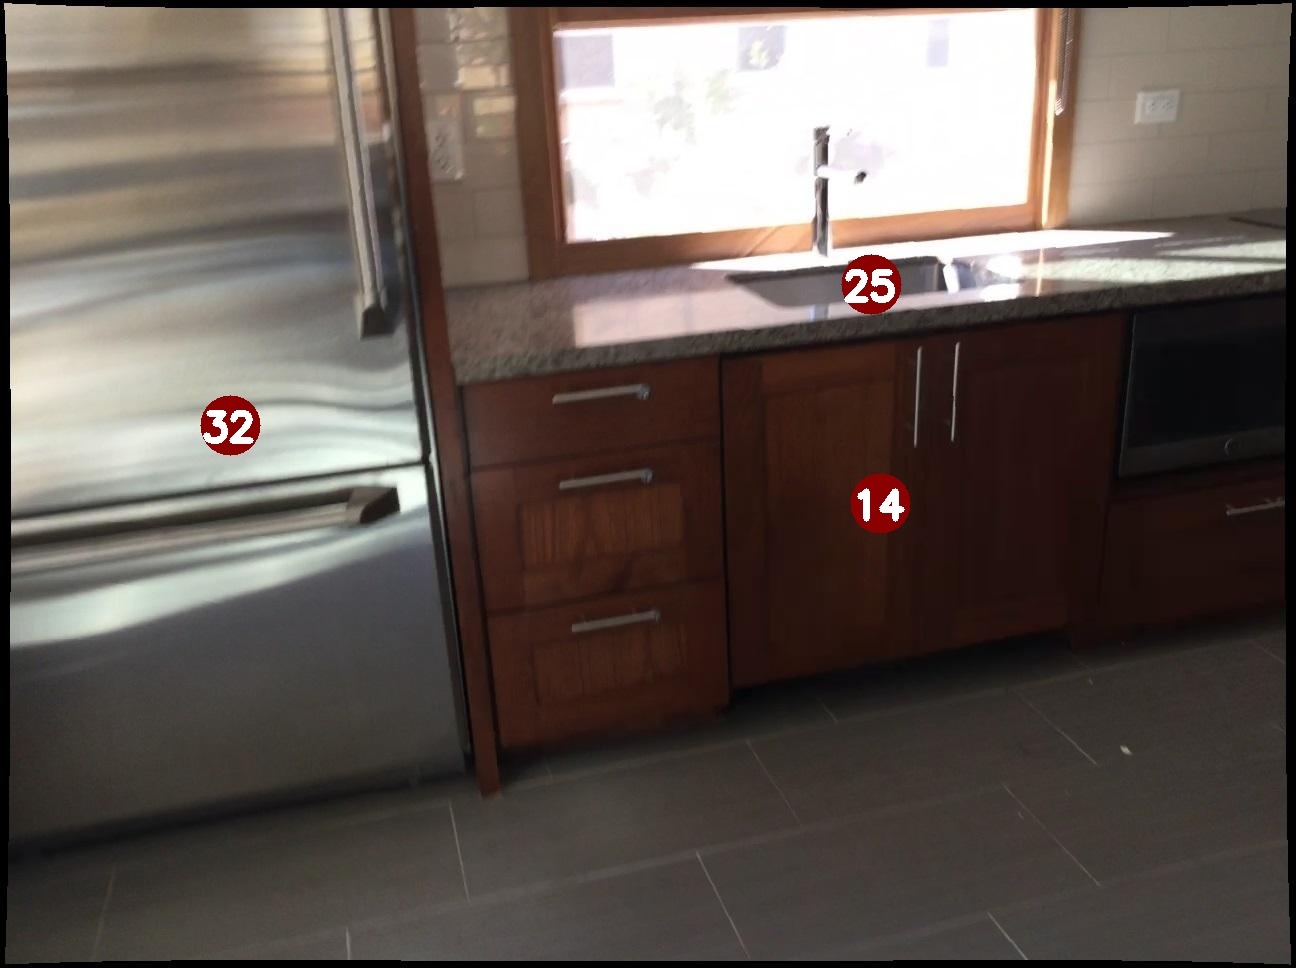} &
    \includegraphics[width=0.22\linewidth]{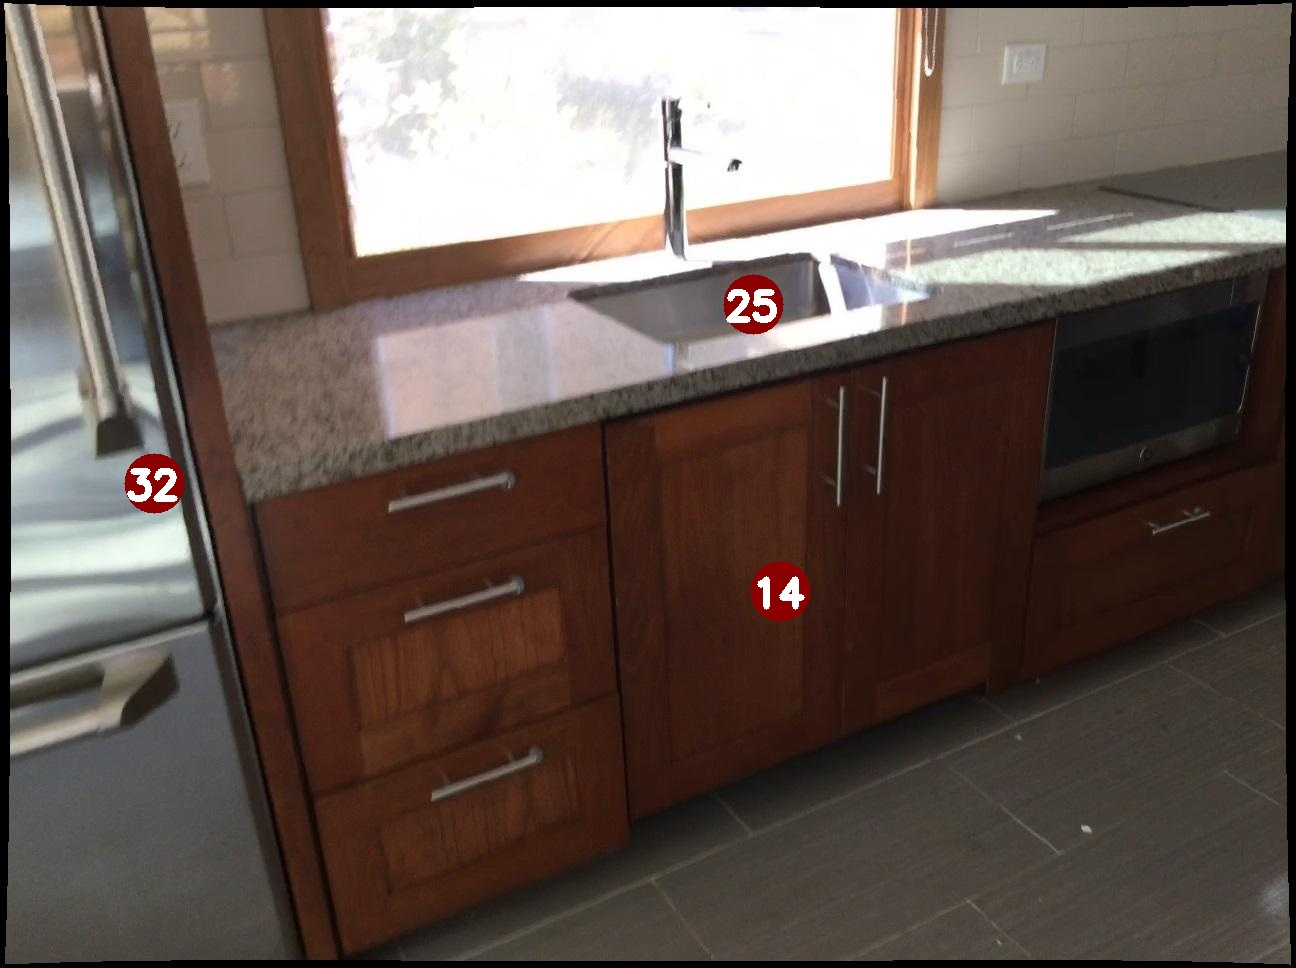} \\
    \vspace{0.1em} \\
    \includegraphics[width=0.22\linewidth]{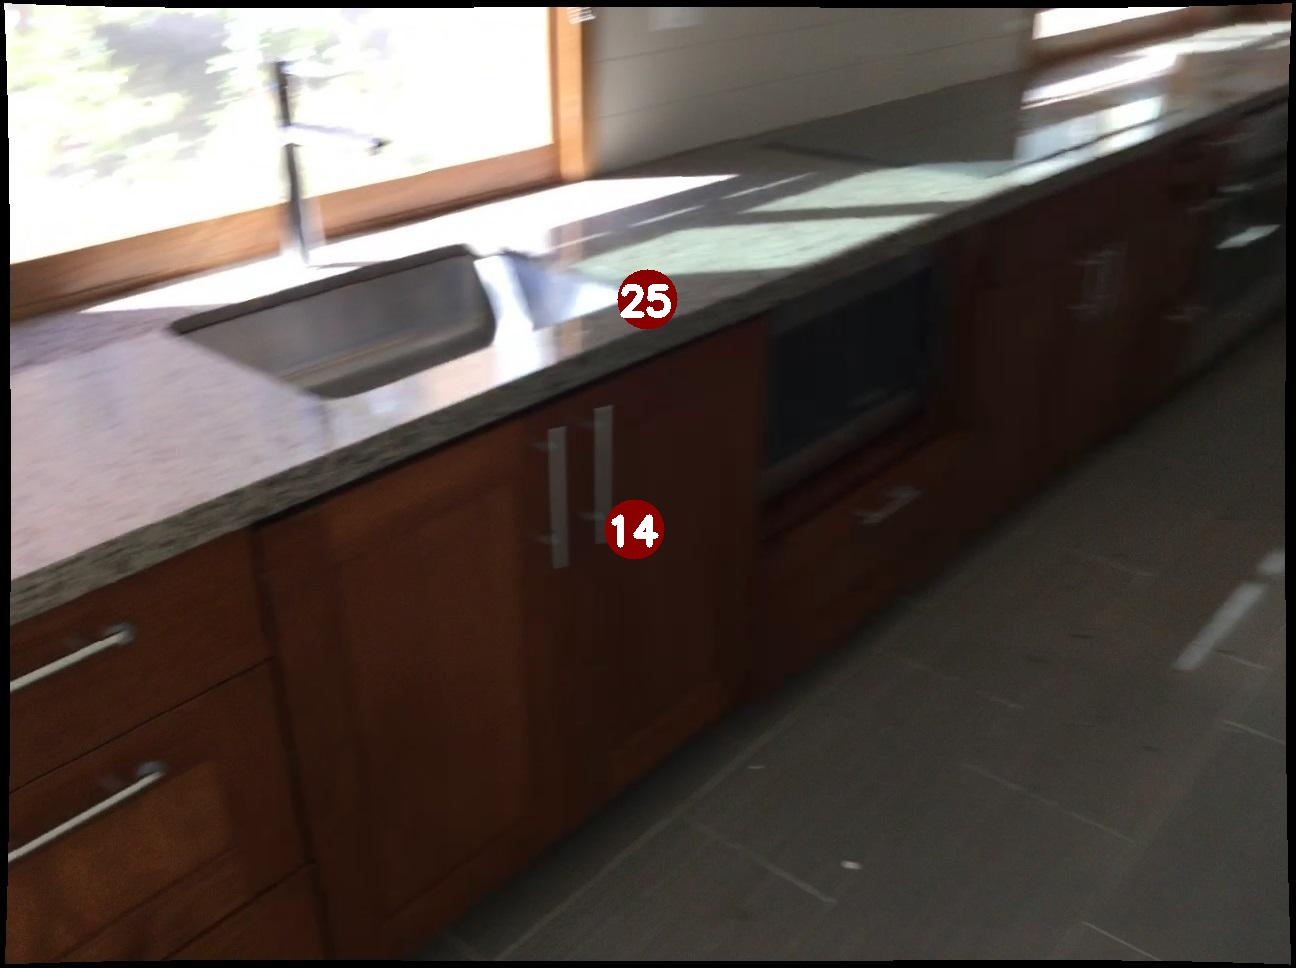} &
    \includegraphics[width=0.22\linewidth]{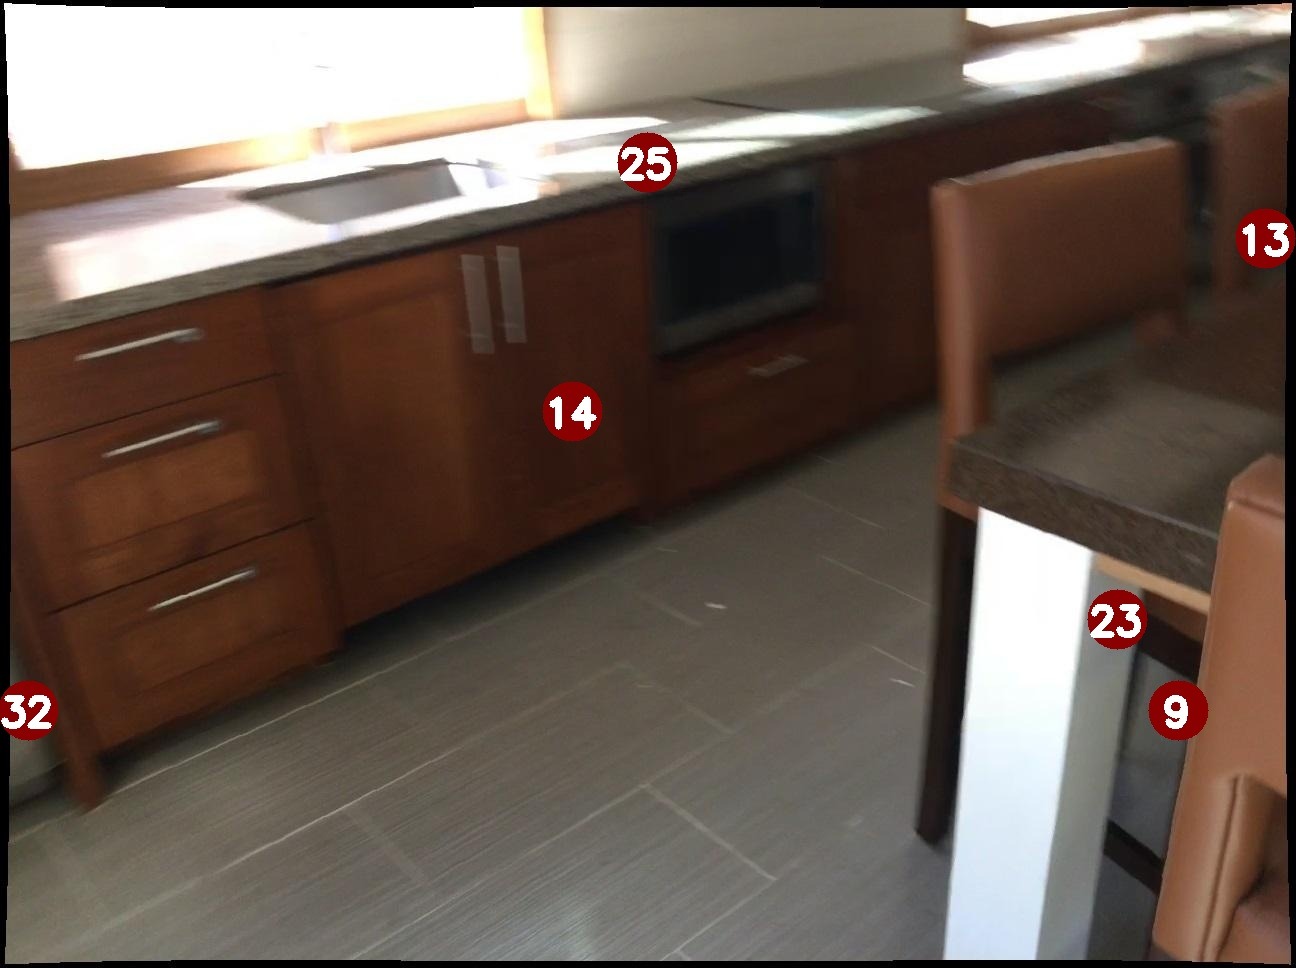} &
    \includegraphics[width=0.22\linewidth]{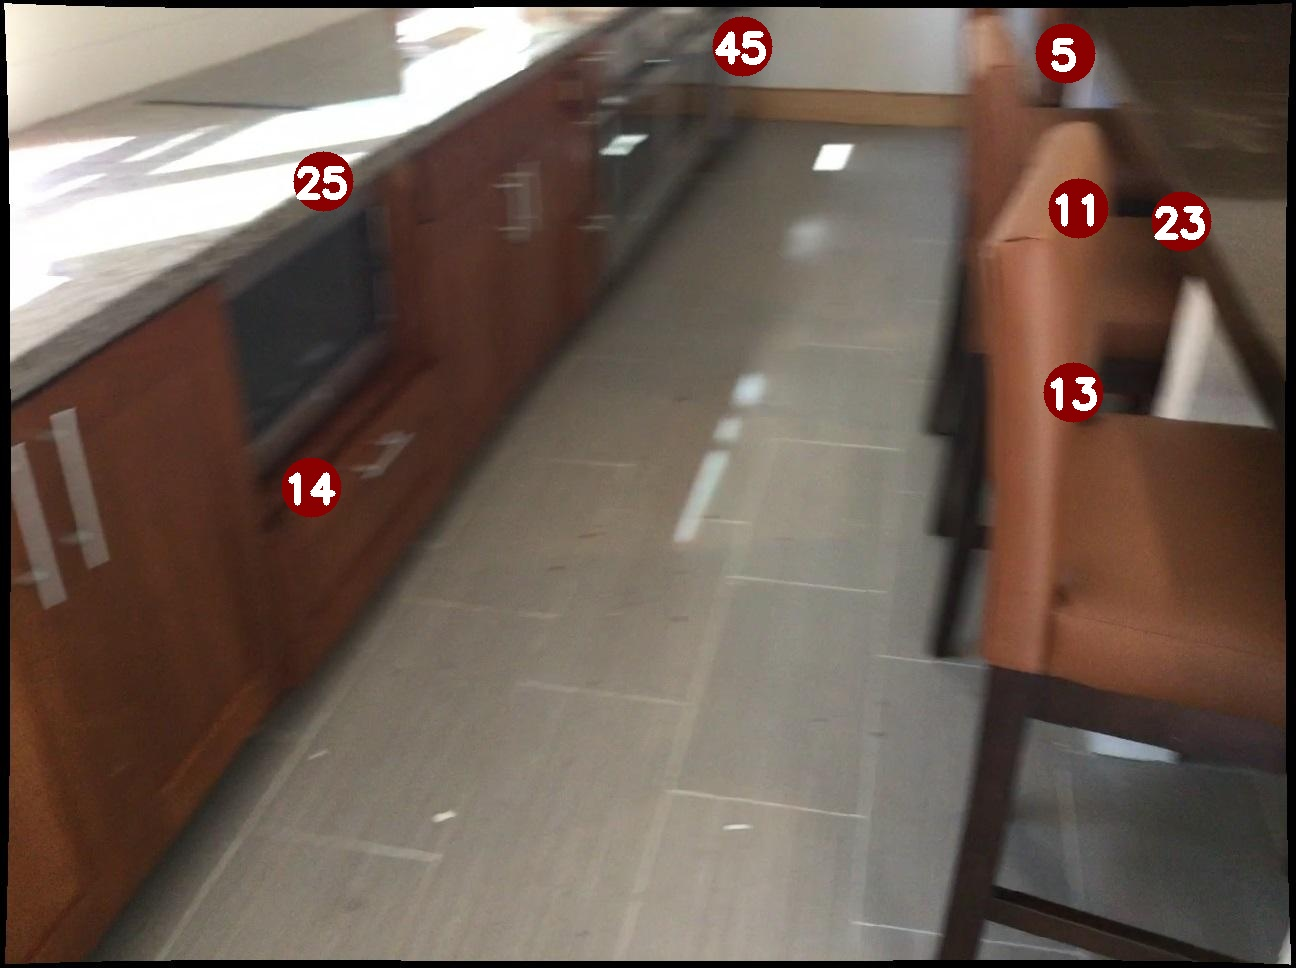} &
    \includegraphics[width=0.22\linewidth]{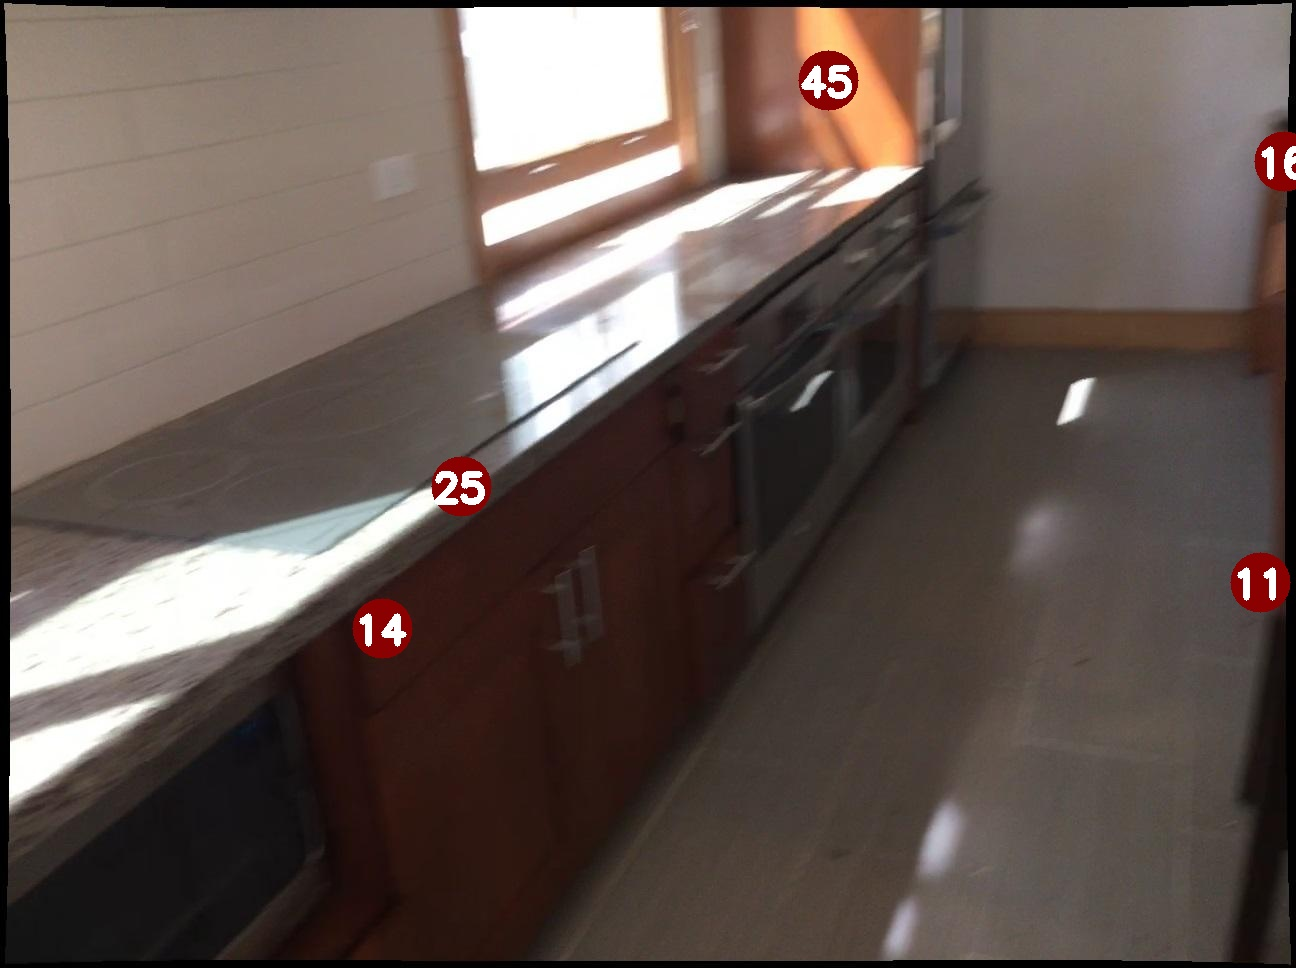} \\
    \textbf{Question}: & \multicolumn{3}{p{0.72\linewidth}}{Identify the ID of the object that closely aligns with the description "there is a set of bottom kitchen cabinets in the room. it has a microwave in the middle of it".
} \\
    \midrule
    \textbf{Qwen2.5-VL}: & \multicolumn{3}{p{0.72\linewidth}}{<points \colorbox{red!20}{x1="208" y1="369"} alt="a set of bottom kitchen cabinets in the room.} \\
    \midrule
    \textbf{VeBrain}: & \multicolumn{3}{p{0.72\linewidth}}{\colorbox{green!20}{<OBJ014>}} \\
    \bottomrule
    \end{tabular}
\end{table}

\begin{table}[ht]
    \centering
    \begin{tabular}{cccc}
    \toprule
    \multicolumn{4}{c}{\textbf{Spatial Reasoning: Example \#6 from SQA3D.}} \\
    \midrule
    \includegraphics[width=0.22\linewidth]{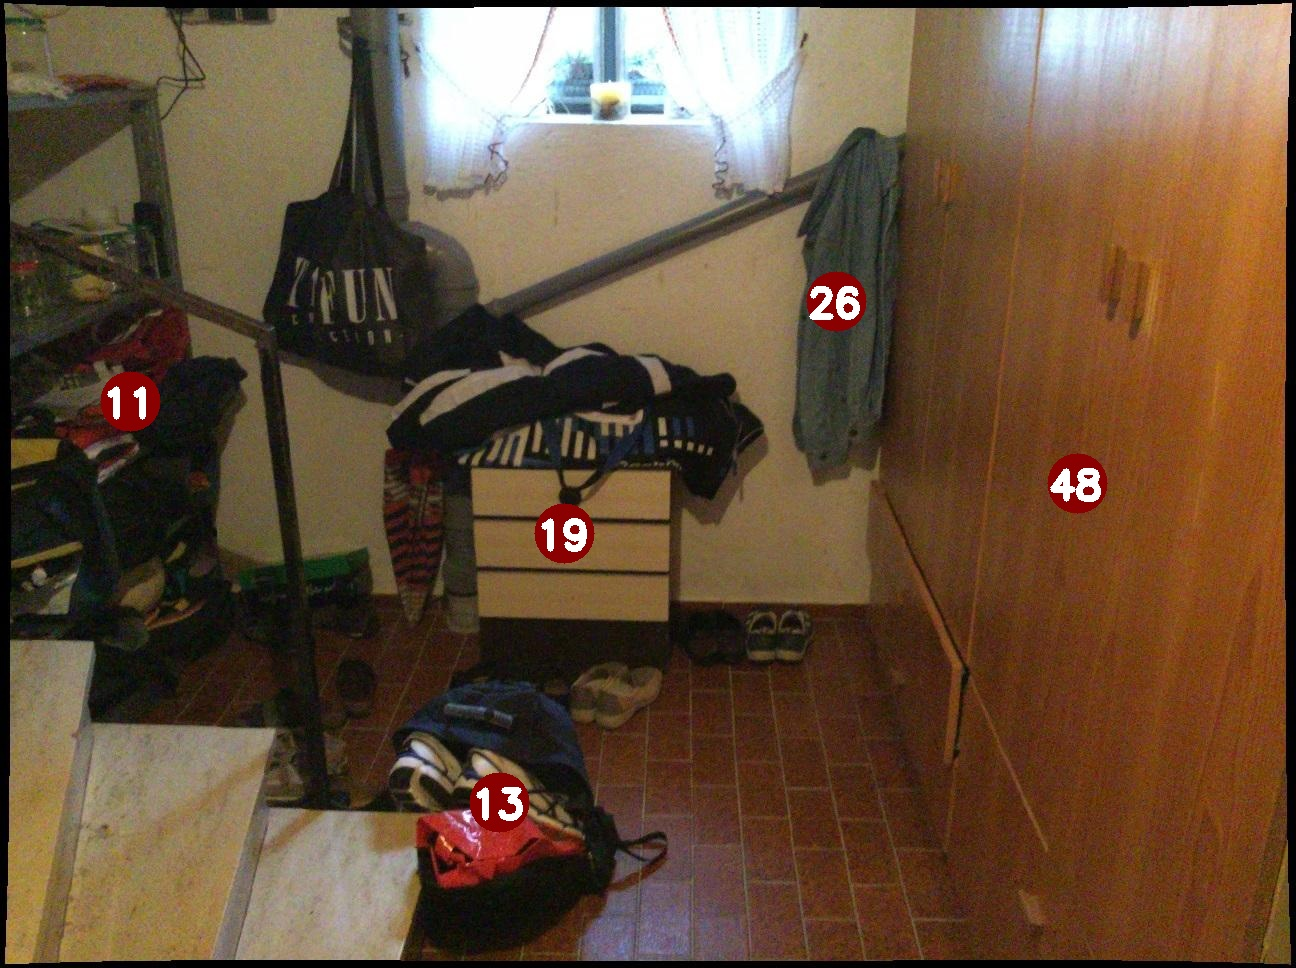} &
    \includegraphics[width=0.22\linewidth]{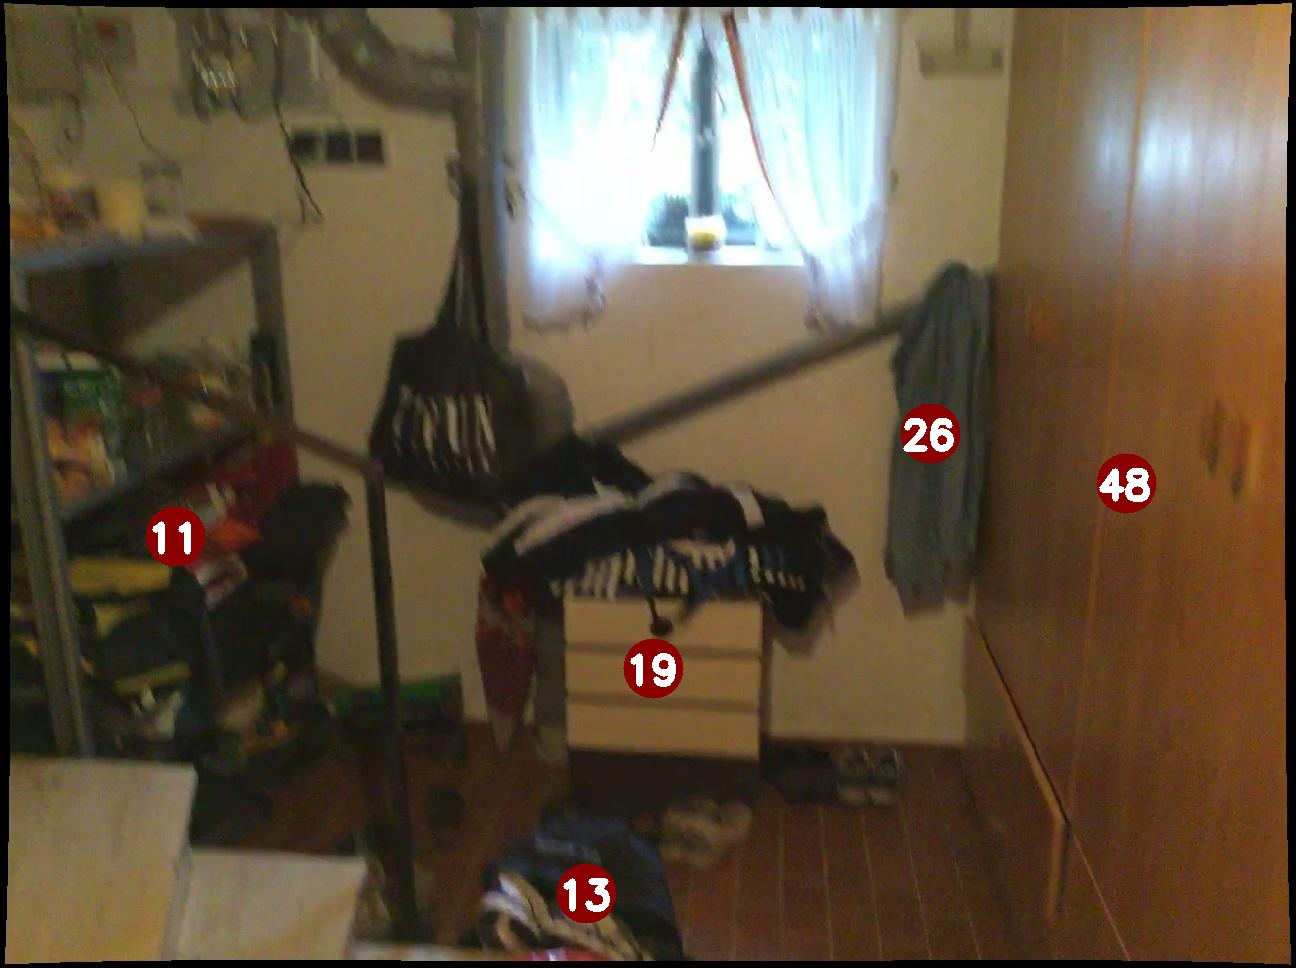} &
    \includegraphics[width=0.22\linewidth]{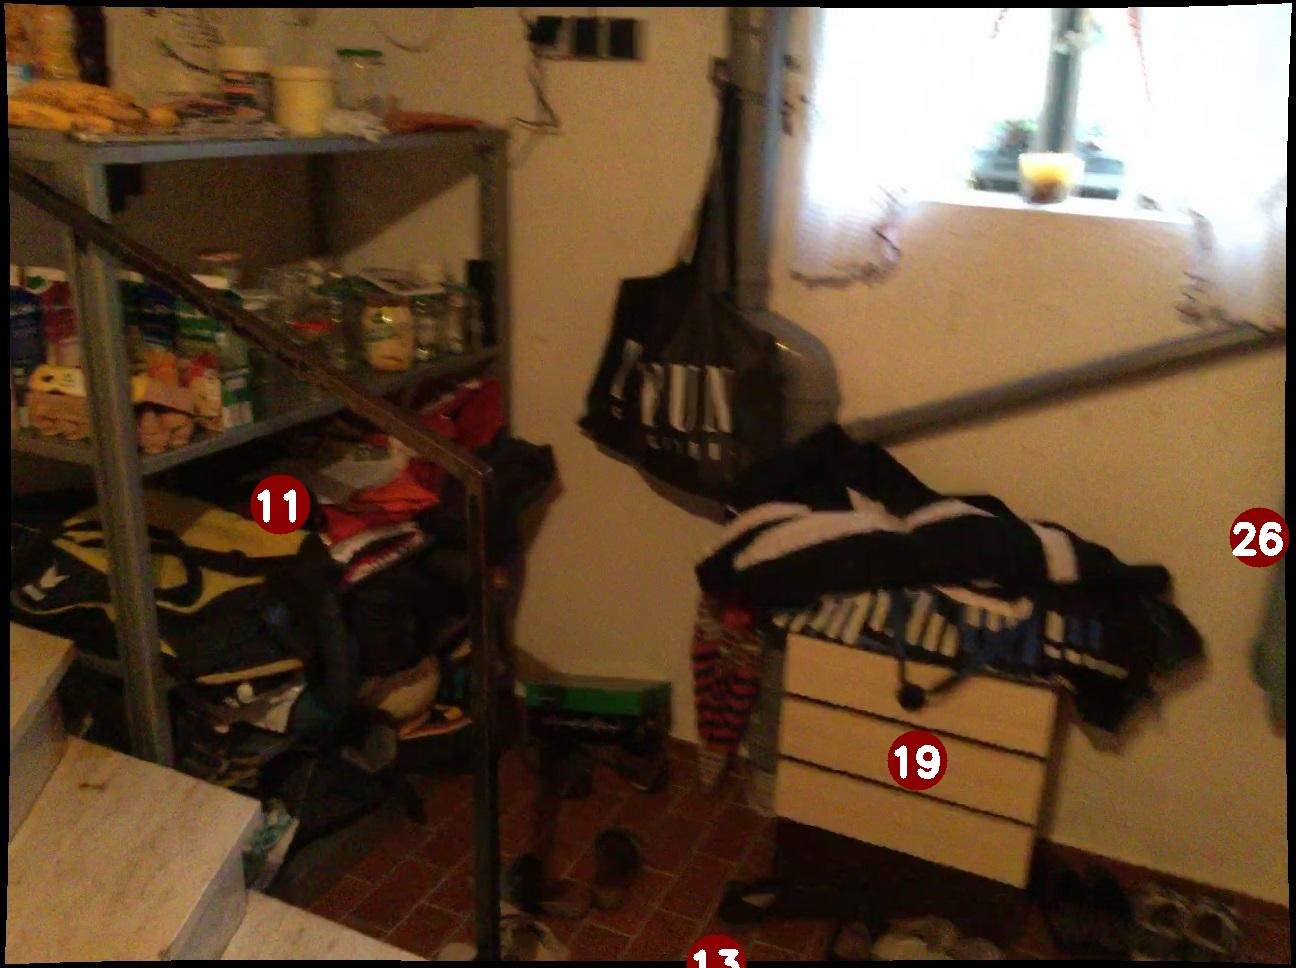} &
    \includegraphics[width=0.22\linewidth]{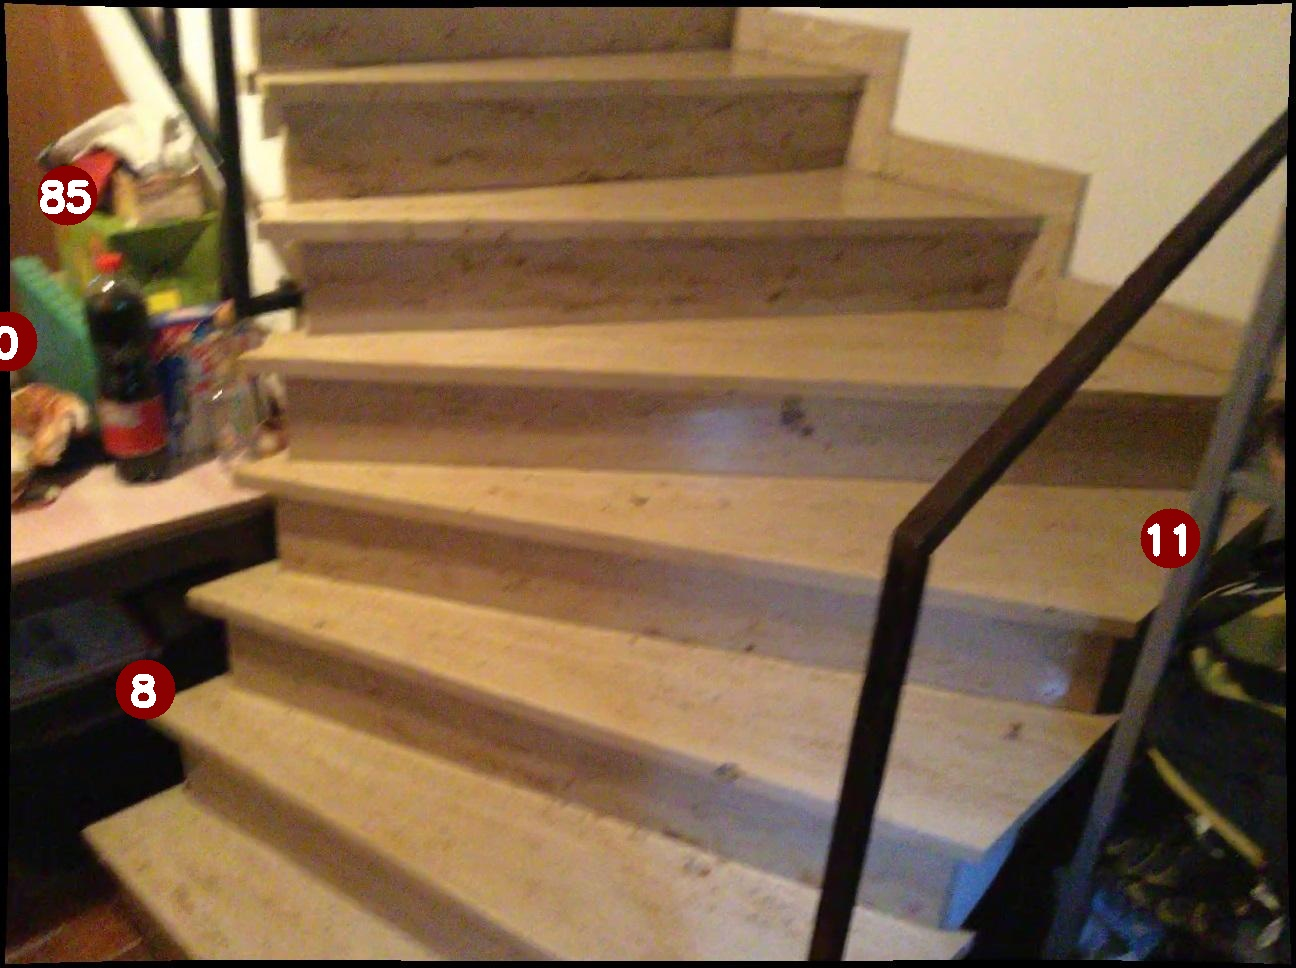} \\
    \vspace{0.1em} \\
    \includegraphics[width=0.22\linewidth]{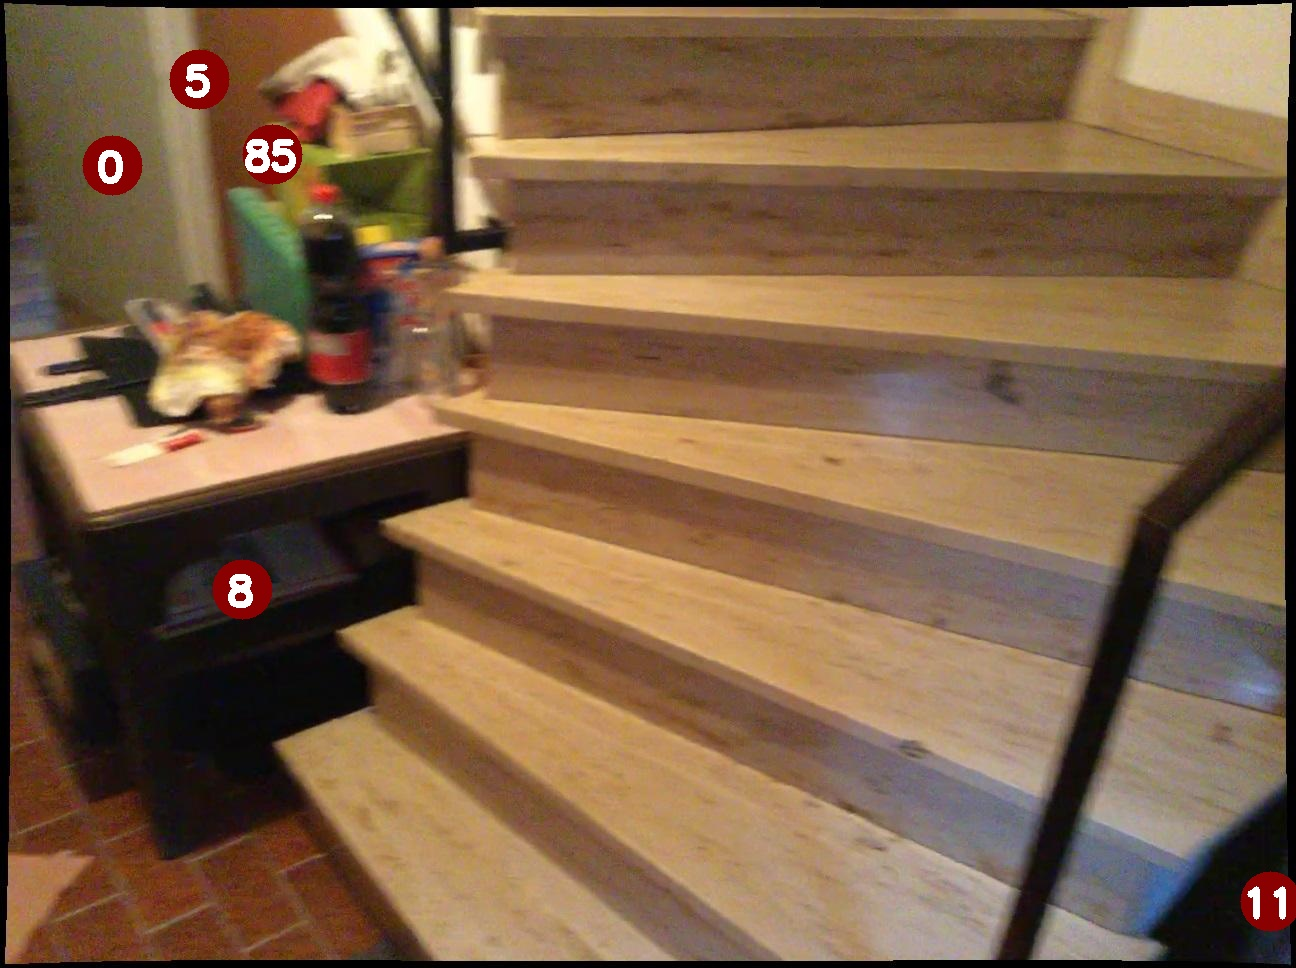} &
    \includegraphics[width=0.22\linewidth]{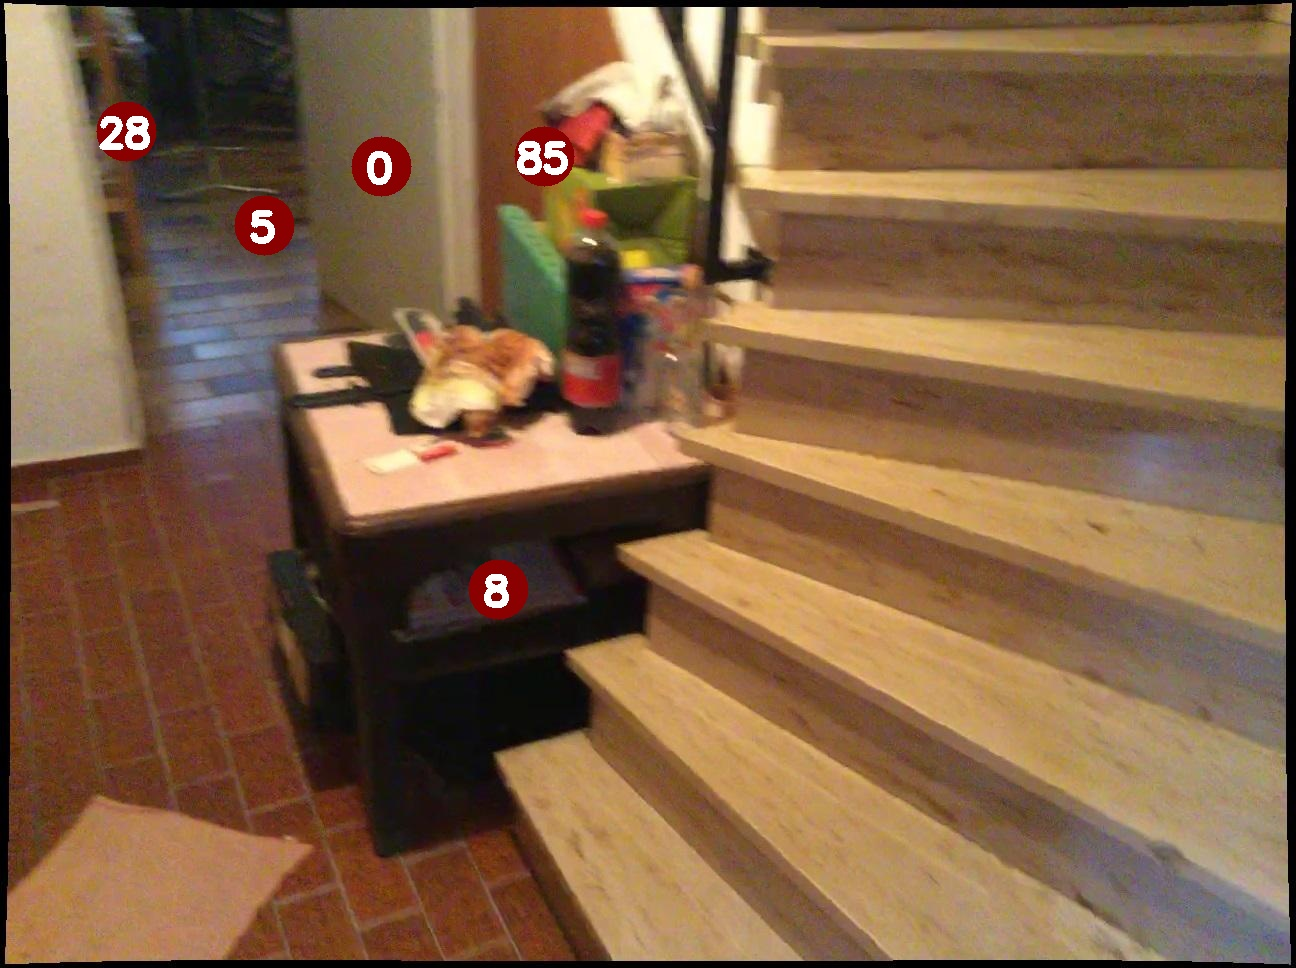} &
    \includegraphics[width=0.22\linewidth]{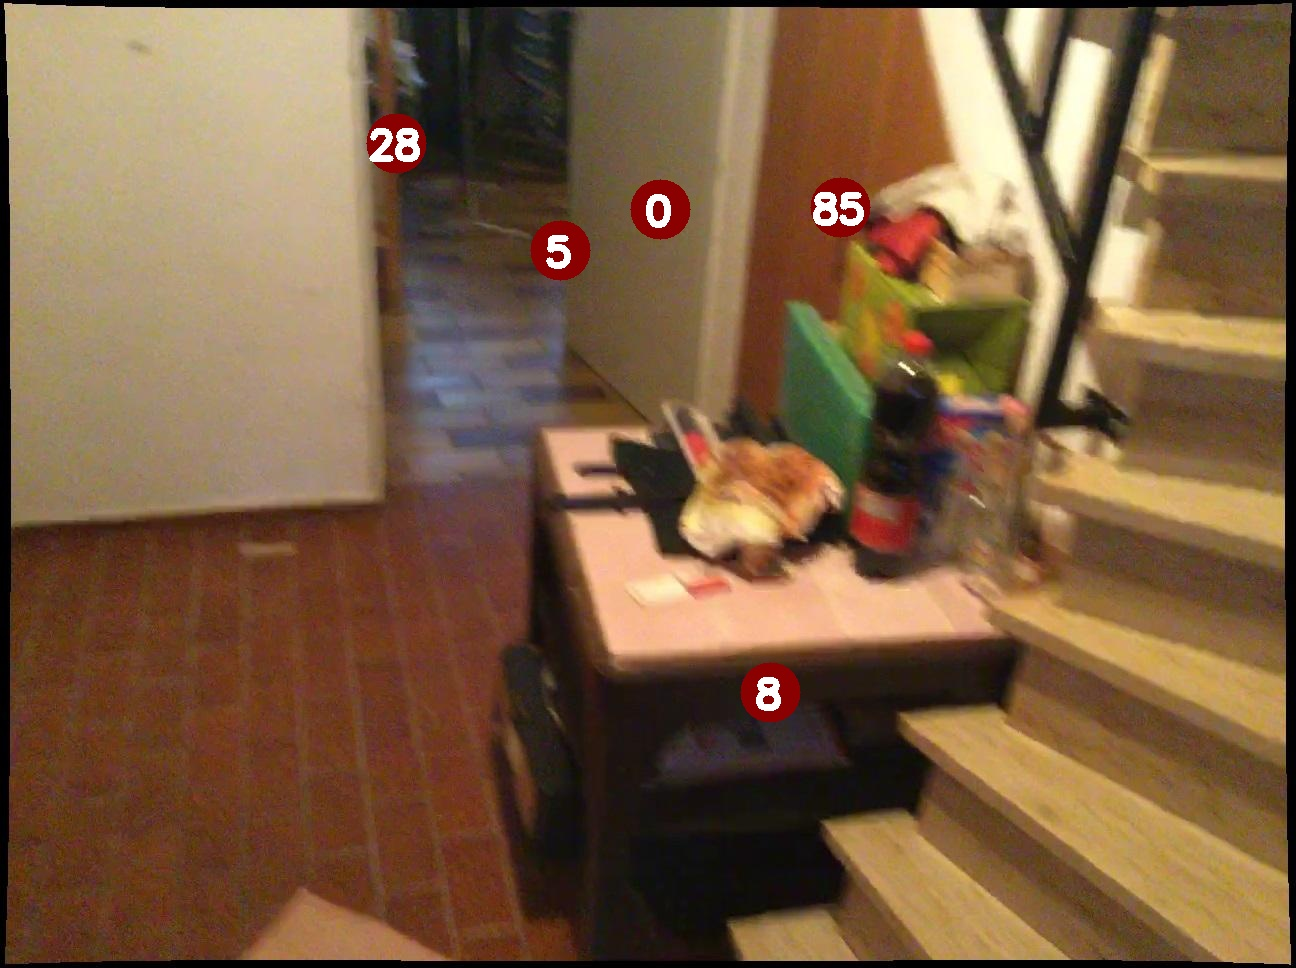} &
    \includegraphics[width=0.22\linewidth]{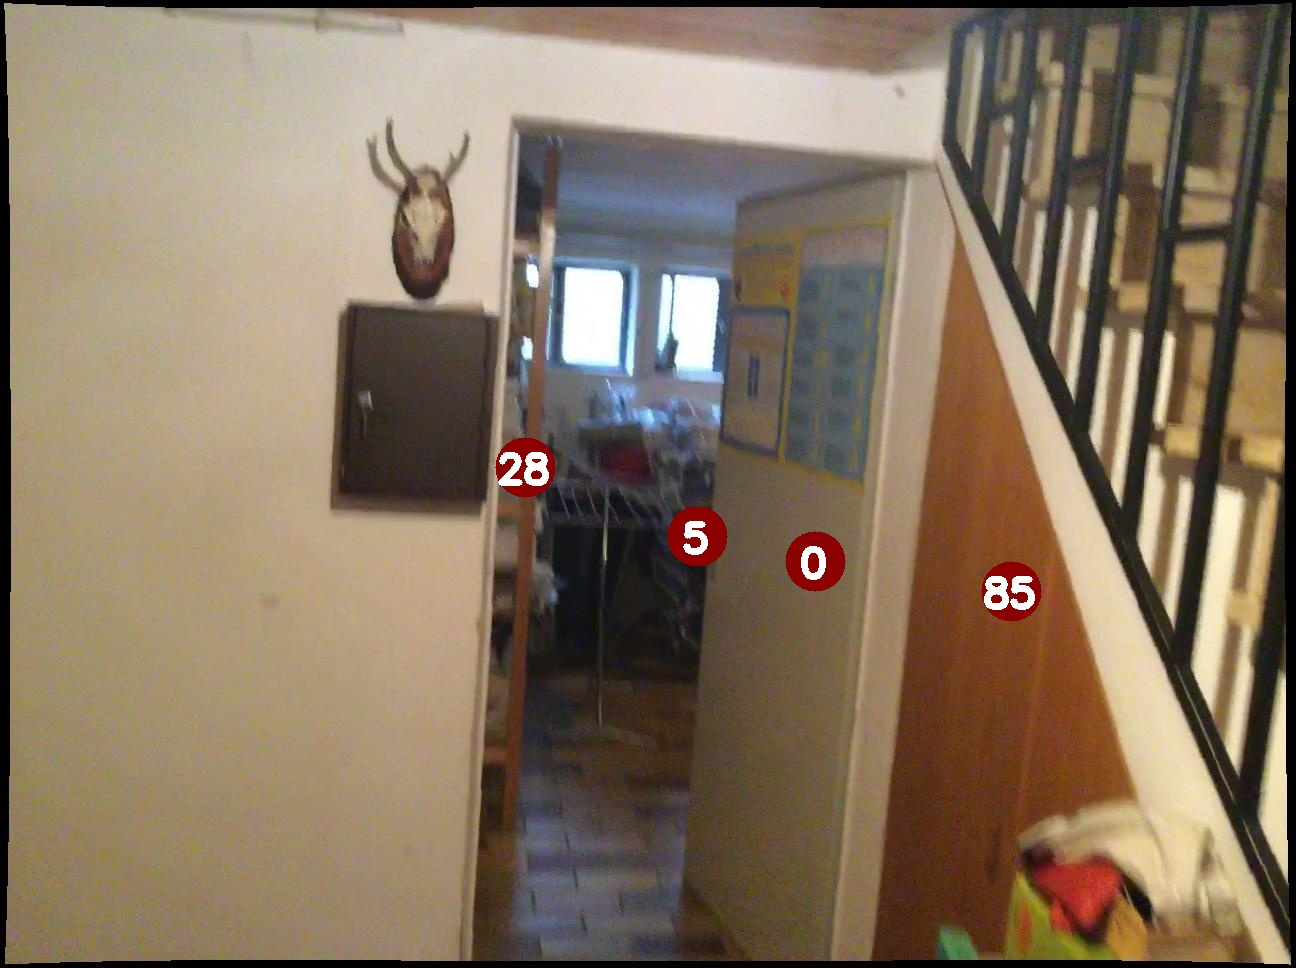} \\
    \textbf{Question}: & \multicolumn{3}{p{0.72\linewidth}}{I am standing at the second stair landing holding on to the handrails with my left hand, the wardrobe is in the face of me. Where is the closest door to me? Answer the question using a single word or phrase.
} \\
    \midrule
    \textbf{Qwen2.5-VL}: & \multicolumn{3}{p{0.72\linewidth}}{\colorbox{red!20}{Left}} \\
    \midrule
    \textbf{VeBrain}: & \multicolumn{3}{p{0.72\linewidth}}{\colorbox{green!20}{Right}} \\
    \bottomrule
    \end{tabular}
\end{table}

\begin{table}[ht]
    \centering
    \begin{tabular}{cccc}
    \toprule
    \multicolumn{4}{c}{\textbf{Spatial Reasoning: Example \#7 from VSI-Bench.}} \\
    \midrule
    \includegraphics[width=0.22\linewidth]{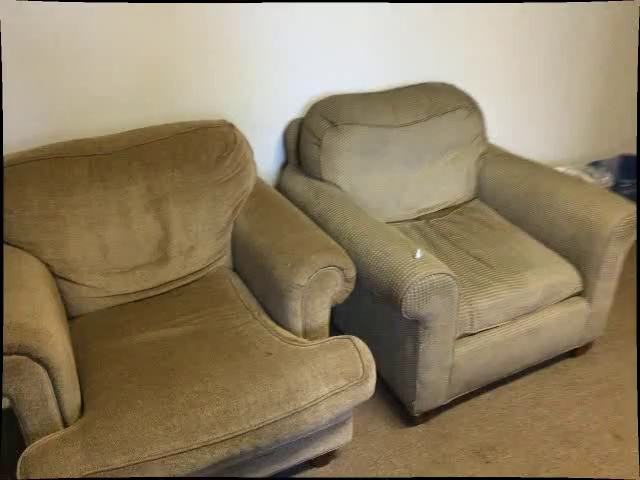} &
    \includegraphics[width=0.22\linewidth]{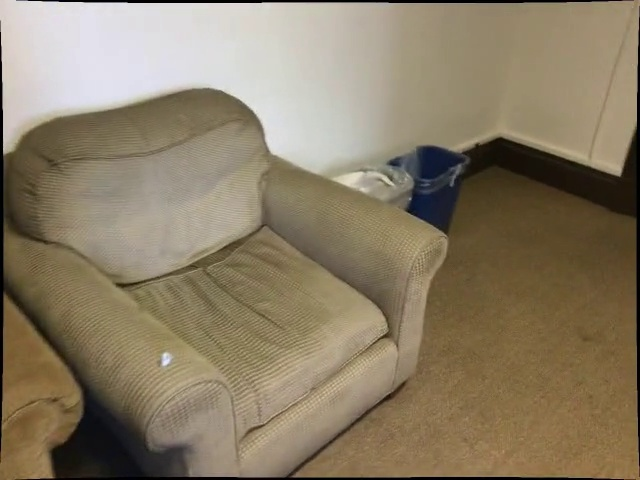} &
    \includegraphics[width=0.22\linewidth]{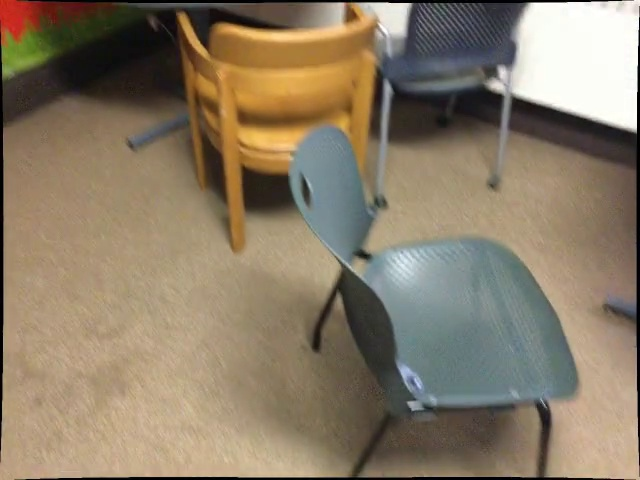} &
    \includegraphics[width=0.22\linewidth]{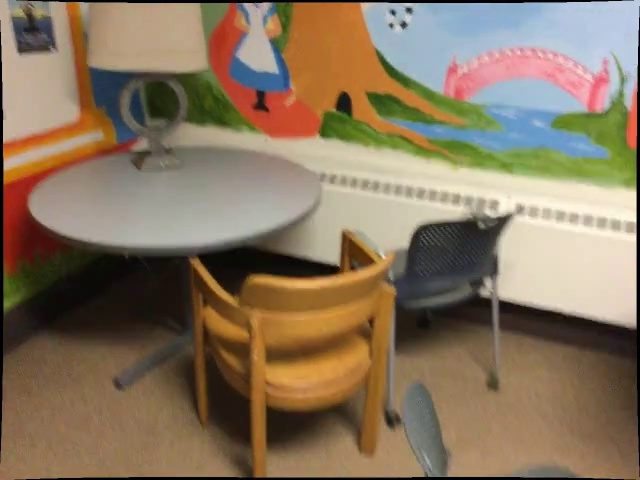} \\
    \vspace{0.1em} \\
    \includegraphics[width=0.22\linewidth]{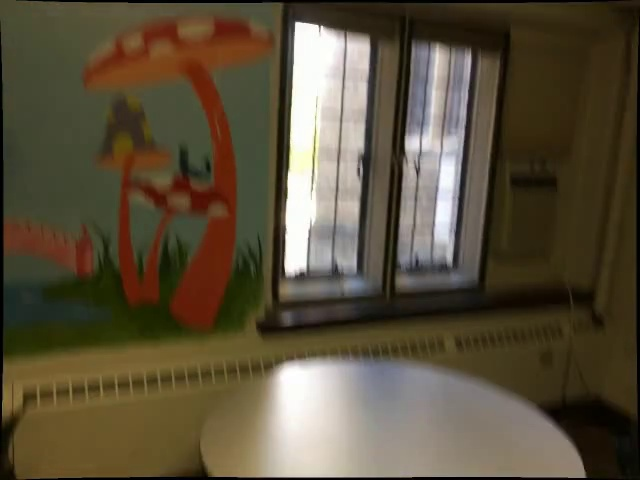} &
    \includegraphics[width=0.22\linewidth]{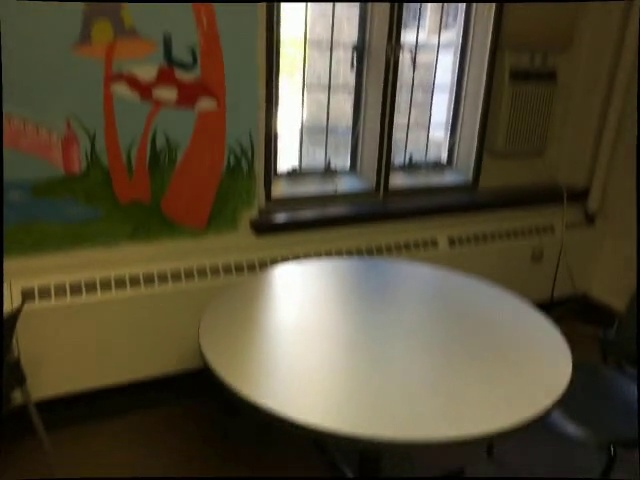} &
    \includegraphics[width=0.22\linewidth]{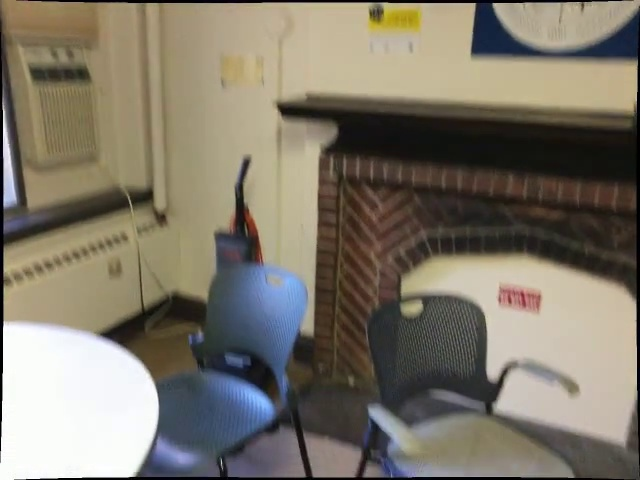} &
    \includegraphics[width=0.22\linewidth]{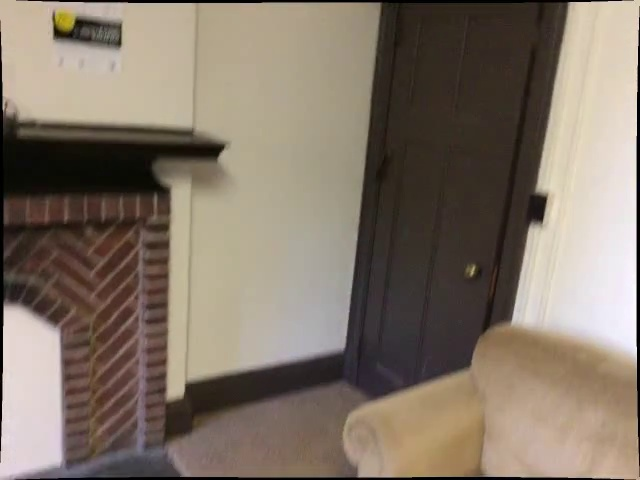} \\
    \textbf{Question}: & \multicolumn{3}{p{0.72\linewidth}}{How many chair(s) are in this room?\newline
    Please answer the question using a single word or phrase.} \\
    \midrule
    \textbf{Qwen2.5-VL}: & \multicolumn{3}{p{0.72\linewidth}}{\colorbox{red!20}{6}} \\
    \midrule
    \textbf{VeBrain}: & \multicolumn{3}{p{0.72\linewidth}}{\colorbox{green!20}{7}} \\
    \bottomrule
    \end{tabular}
\end{table}

\begin{table}[ht]
    \centering
    \begin{tabular}{cccc}
    \toprule
    \multicolumn{4}{c}{\textbf{Spatial Reasoning: Example \#8 from VSI-Bench.}} \\
    \midrule
    \includegraphics[width=0.22\linewidth]{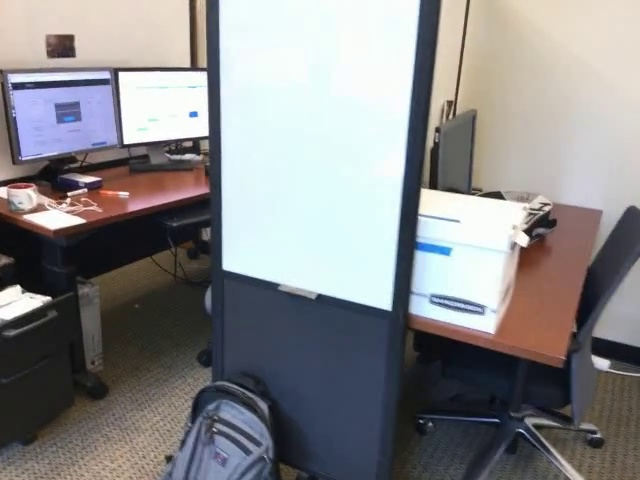} &
    \includegraphics[width=0.22\linewidth]{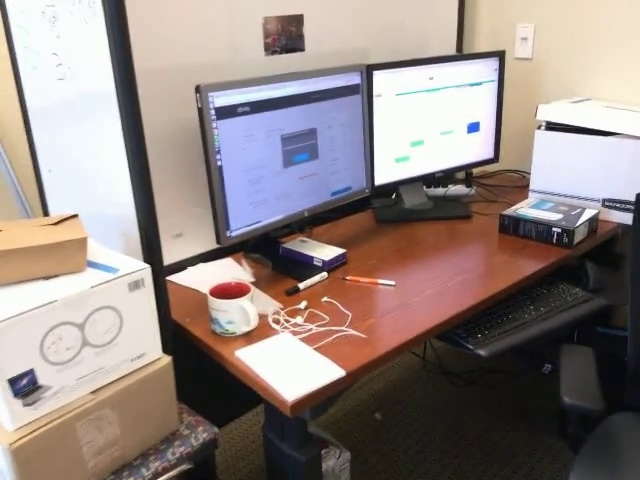} &
    \includegraphics[width=0.22\linewidth]{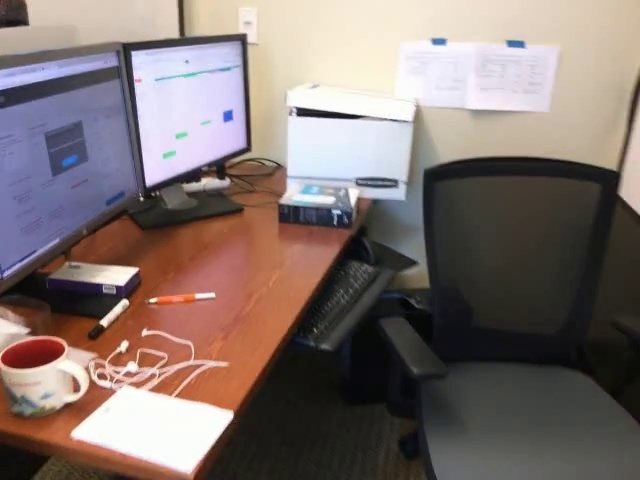} &
    \includegraphics[width=0.22\linewidth]{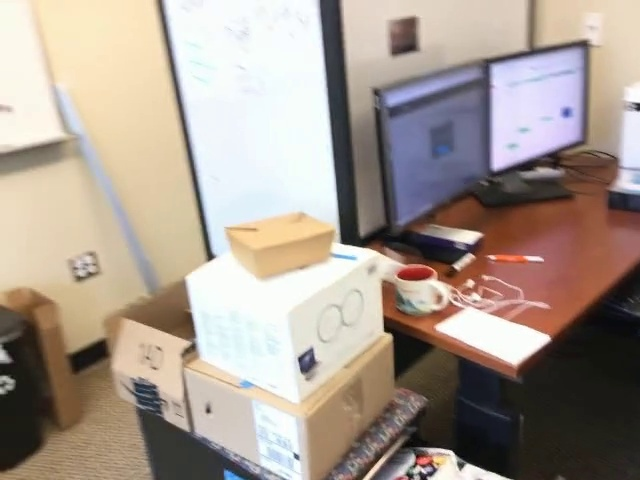} \\
    \vspace{0.1em} \\
    \includegraphics[width=0.22\linewidth]{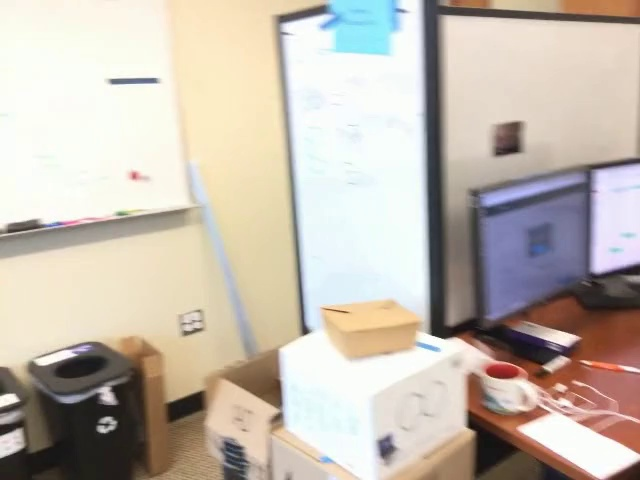} &
    \includegraphics[width=0.22\linewidth]{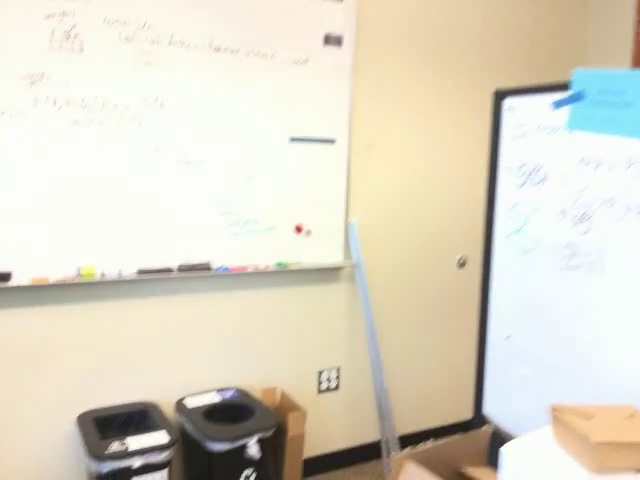} &
    \includegraphics[width=0.22\linewidth]{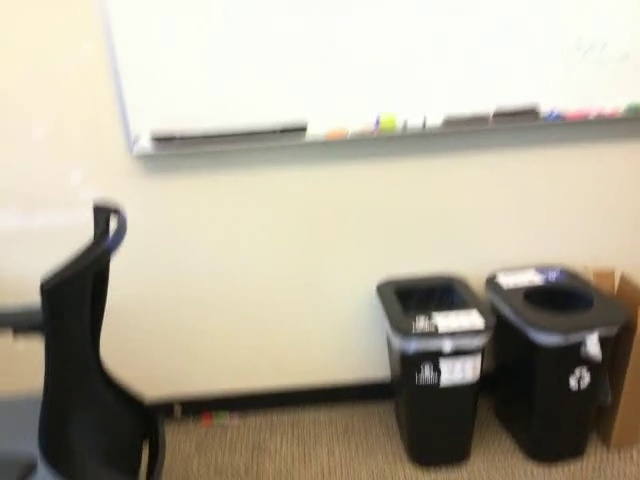} &
    \includegraphics[width=0.22\linewidth]{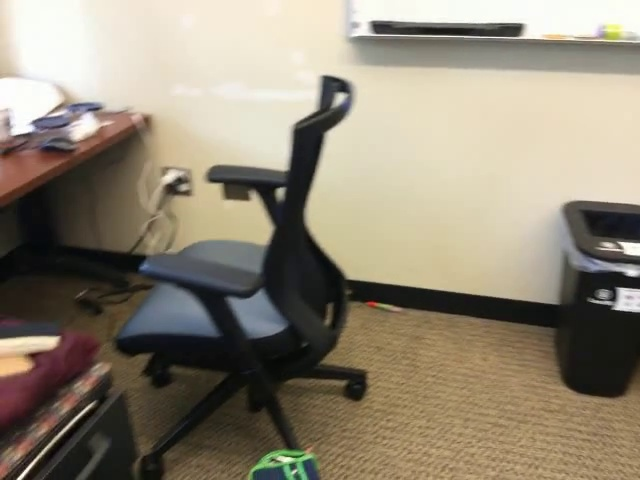} \\
    \textbf{Question}: & \multicolumn{3}{p{0.72\linewidth}}{Measuring from the closest point of each object, which of these objects (chair, table, trash bin, monitor) is the closest to the whiteboard?\newline
    A. chair\newline
    B. table\newline
    C. trash bin\newline
    D. monitor\newline
    Answer with the option's letter from the given choices directly.} \\
    \midrule
    \textbf{Qwen2.5-VL}: & \multicolumn{3}{p{0.72\linewidth}}{\colorbox{red!20}{D}} \\
    \midrule
    \textbf{VeBrain}: & \multicolumn{3}{p{0.72\linewidth}}{\colorbox{green!20}{C}} \\
    \bottomrule
    \end{tabular}
\end{table}
