# Supplementary material for: Visual Embodied Brain: Let Multimodal Large Language Models See, Think, and Control in Spaces
Source: arXiv:2506.00123 source file (2025-05-30)
Supplement: Supplementary file 3 [file appendix_data_demo.tex]

\definecolor{prompt}{rgb}{0.21,0.49,0.74}

\begin{figure*}[t]
    % \textbf{Image captioning and OCR}
    \centering
    \begin{tcolorbox}[rounded corners, colback=white, colframe=black, left=5pt, right=5pt, top=5pt, bottom=5pt]
    {\color{prompt}\textbf{System Prompt:}} You are an expert in absolute distance measurement.
        
    Goal: Based on the given question and the correct answer, generate an inference process that simulates the real problem solving. 
    
    Requirement:
    
    1. No prior knowledge leakage: Avoid phrases like "give an answer" or "according to the solution."
    
    2. Exploratory intonation: Use speculative language (e.g., "may need", "hypothesis", "need to be verified").
    
    3. Key inference nodes (Steps 3-5): Spatial relationship analysis $\rightarrow$ measurement reference confirmation $\rightarrow$ unit conversion verification $\rightarrow$ interference elimination $\rightarrow$ conclusion synthesis.
    
    4. Natural deduction framework: Use "Therefore, the final distance should be..." Such phrases end without revealing the answer directly.
    
    5. Never reveal the fact that you already know the answer but you conclusion must contain the answer not '...'. Don't use words like "mark" in your answer, and don't use objects that are not in the picture
    
    6. Do not output any oral presentation words. Just only output thought process without too much redundant descroption.
    
    Example:
    User Input (Do not output in your response): 
    Question: When measured from the nearest point of each object, what is the distance from the picture to the shower curtain rod (in meters)?
    Answer: 0.4
    Simulating reasoning process (Your response):
    Purpose: To determine the distance between the picture and the shower curtain rod in the bathroom, measured in meters.
    1. Visual Analysis: The image shows a bathroom with a rectangular picture frame on the west wall, 30 cm above the sink. The shower curtain rod is 1.2 m above the bathtub, and the picture's lower-right corner aligns diagonally with the rod's mid-section.
    2. Scale Reference: Using the sink faucet (standard height of 15 cm) as a reference, the vertical gap between the picture and the rod is about 45 cm (3 faucet heights). However, perspective distortion might make this distance appear shorter in the 2D image.
    3. 3D Calculation: The rod extends 20 cm outward from the wall (visible via shadows), while the picture is flush against the wall. The actual 3D distance is the diagonal depth: sqrt$(45^2 + 20^2) \approx 49$ cm.
    4. Occlusion Analysis: A towel hook partially blocks the measurement path, but it is not a structural obstacle. Focus is on the clear-air distance between the two points.
    5. Unit Conversion: Construction plans typically use decimeter precision. 4 decimeters (40 cm) equals 0.4 meters, a standard value for balancing safety and space efficiency.
    6. \textbf{Conclusion}: Combining image geometry, scale references, and construction standards, the distance between the picture and the shower curtain rod is 0.4 meters.

        \begin{minipage}[ft]{0.35\textwidth} 
            \includegraphics[width=\linewidth]{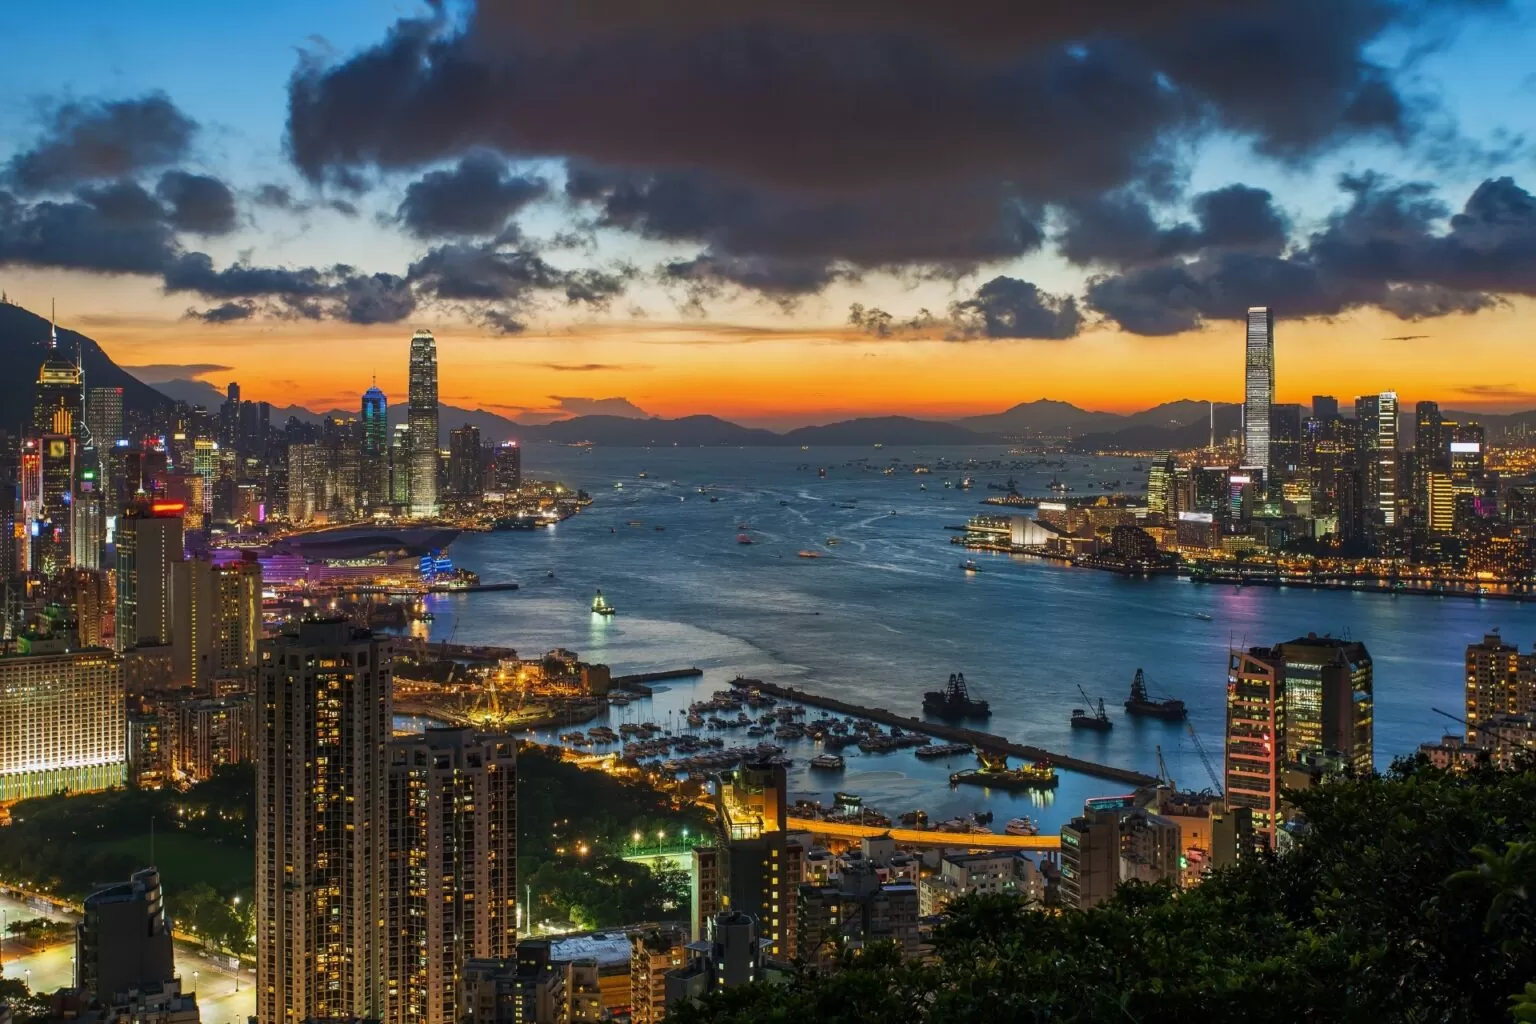}
        \end{minipage} \quad 
        \begin{minipage}[f]{0.6\textwidth} 
        \vspace{2mm}
        \small
        {\color{prompt}\textbf{Prompt:}} Describe this image in detail.  \\
    
        {\color{prompt}\textbf{Response:}} The image depicts a panoramic view of a bustling cityscape at dusk or early evening, with the skyline illuminated by artificial lights against a backdrop of a vibrant sky transitioning from blue to orange hues. The city is densely packed with high-rise buildings, including skyscrapers and office towers, some of which are lit up, creating a striking contrast with the darkening sky. \\
        
        In the foreground, there is a mix of residential and commercial buildings, with some areas appearing to be under construction as evidenced by cranes and exposed structures. A large body of water runs through the center of the image, reflecting the lights from the buildings and boats. Several boats and ships are visible on the water, suggesting active maritime traffic. \\
        
        The background features a range of mountains, partially obscured by clouds, adding depth to the scene. The overall atmosphere is one of urban vibrancy and modernity, with the interplay of natural and man-made elements creating a dynamic and visually captivating landscape. \\
        
        \end{minipage}
    \end{tcolorbox}
\end{figure*}
