# Supplementary material for: Visual Embodied Brain: Let Multimodal Large Language Models See, Think, and Control in Spaces
Source: arXiv:2506.00123 source file (2025-05-30)
Supplement: Supplementary file 4 [file appendix_dog_demo.tex]

\begin{table}[ht]
    \centering
    \caption{\textbf{More Demonstrations of VeBrain on Locomotion Tasks.}}
    \label{tab:dog_demo}
    \resizebox{\linewidth}{!}{
    \begin{tabular}{cp{0.2\linewidth}p{0.2\linewidth}p{0.2\linewidth}p{0.2\linewidth}p{0.2\linewidth}}
    \toprule
    \textbf{Task} & \textbf{Initial Frame} & \multicolumn{4}{l}{\textbf{Subsequent Frames}} \\
    \midrule
    \multirow{6}{*}{\makecell{Find}} & & & & & \\
    &
    \includegraphics[width=\linewidth]{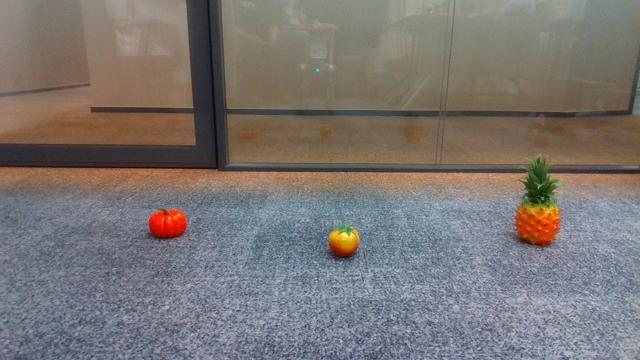} &
    \includegraphics[width=\linewidth]{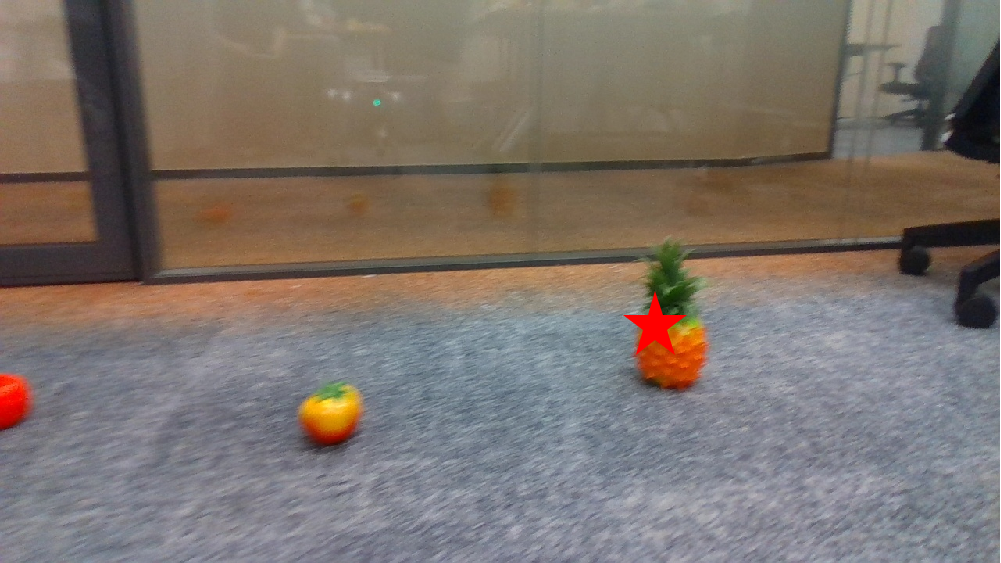} &
    \includegraphics[width=\linewidth]{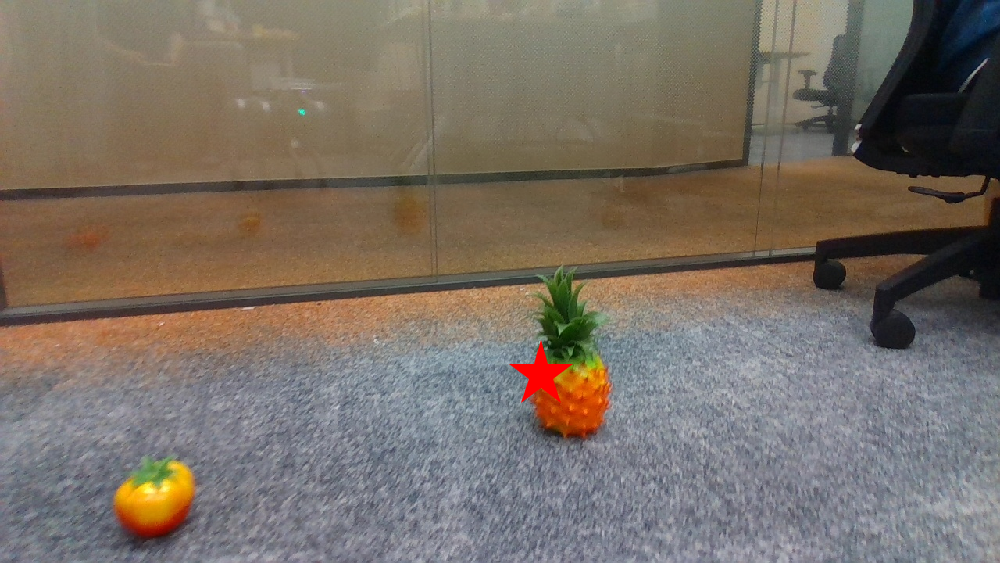} &
    \includegraphics[width=\linewidth]{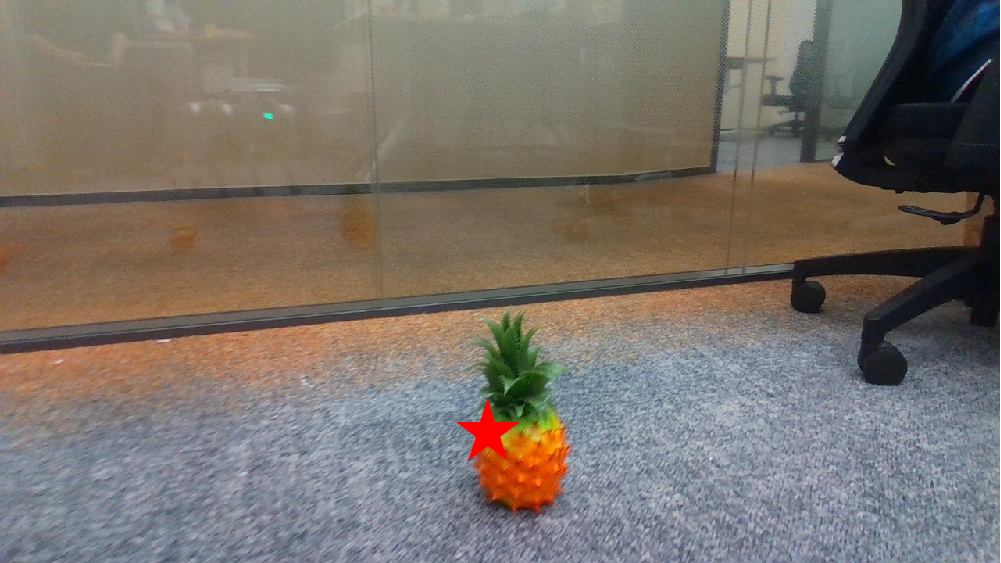} &
    \includegraphics[width=\linewidth]{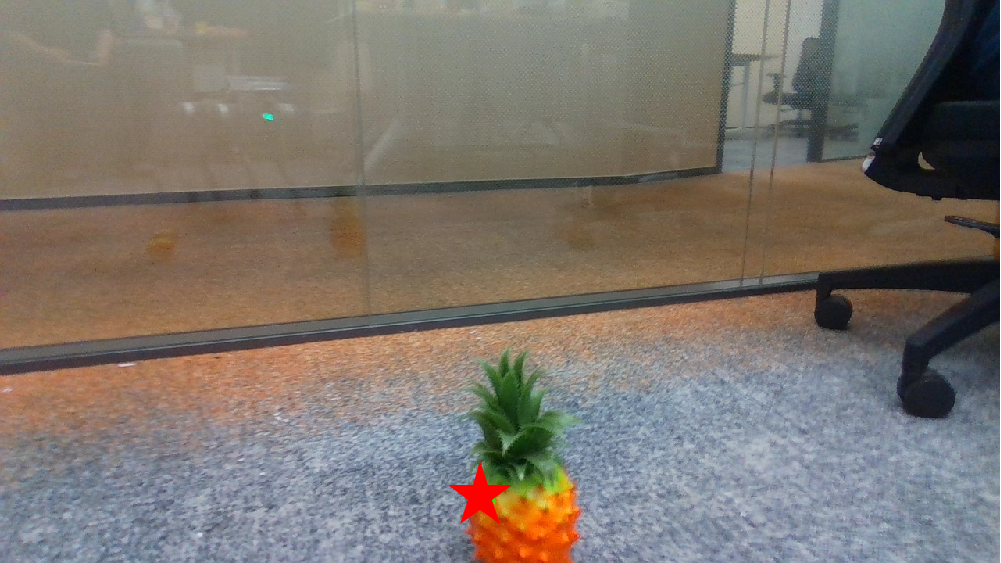} \\
    \multirow{6}{*}{\makecell{Interaction}} & & & & & \\
    &
    \includegraphics[width=\linewidth]{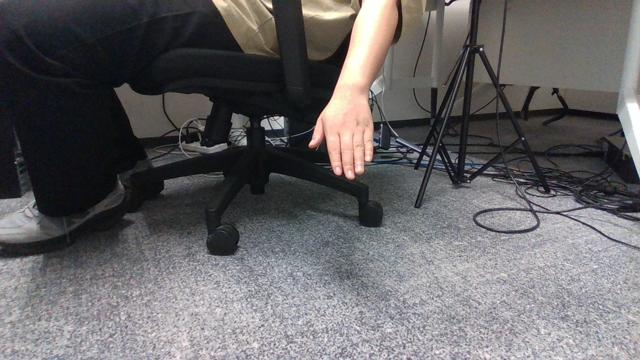} &
    \includegraphics[width=\linewidth]{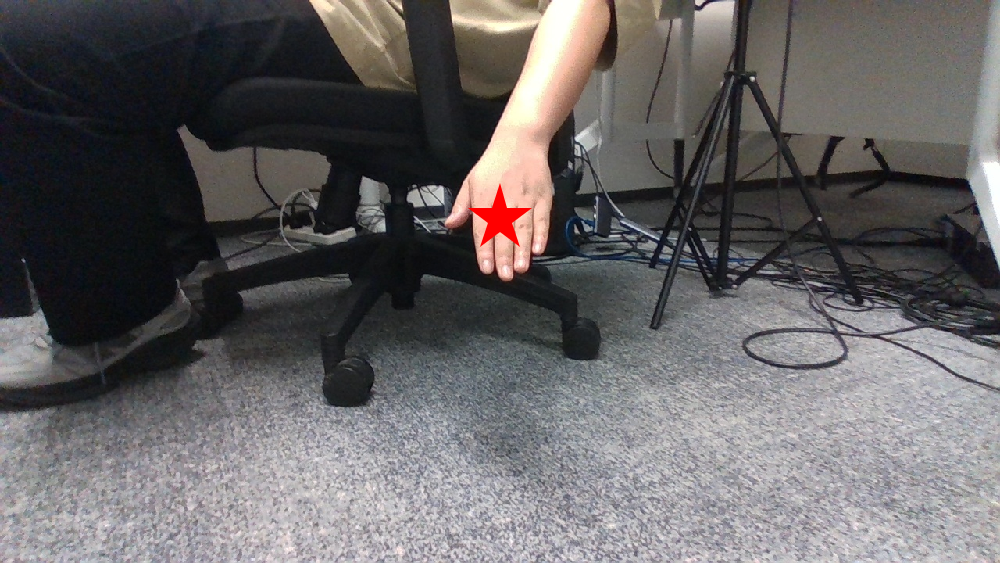} &
    \includegraphics[width=\linewidth]{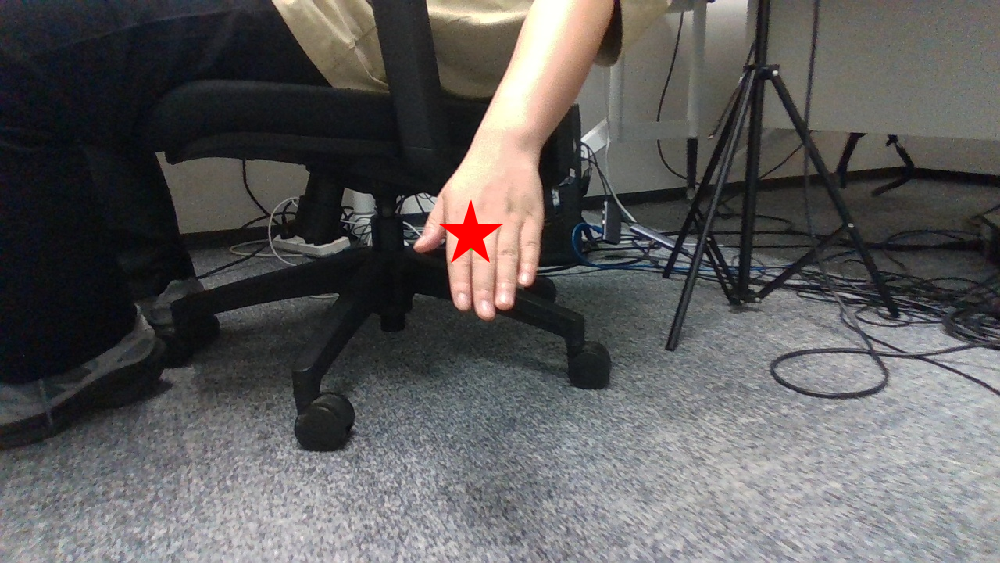} &
    \includegraphics[width=\linewidth]{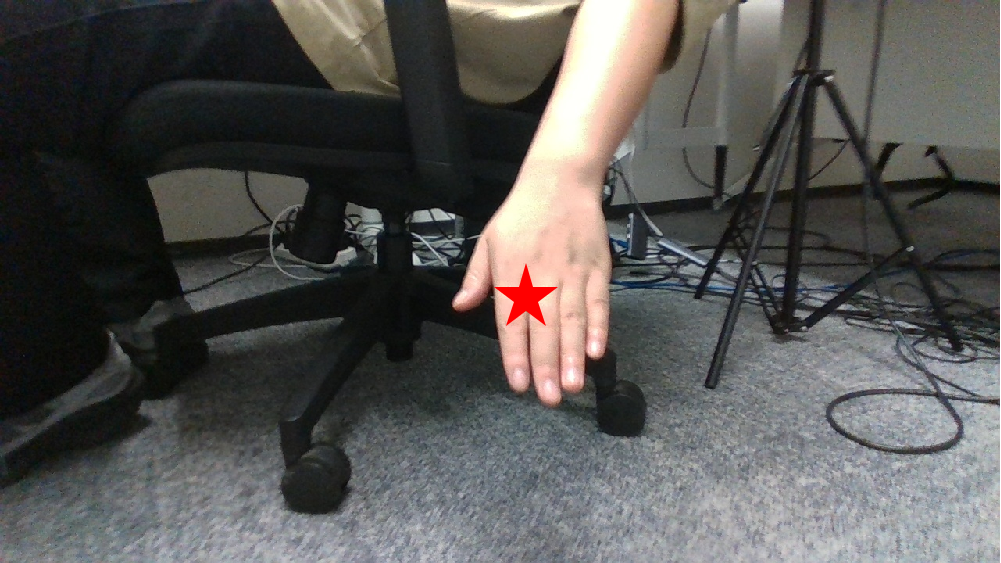} &
    \includegraphics[width=\linewidth]{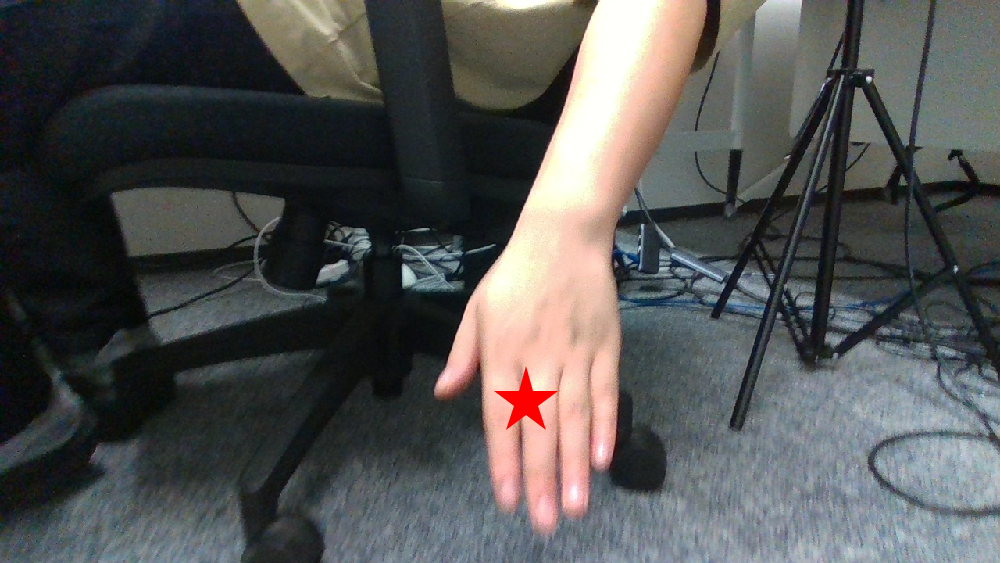} \\
    % \vspace{0.1cm} \\
    \multirow{6}{*}{\makecell{Complex\\Find}} & & & & & \\
    &
    \includegraphics[width=\linewidth]{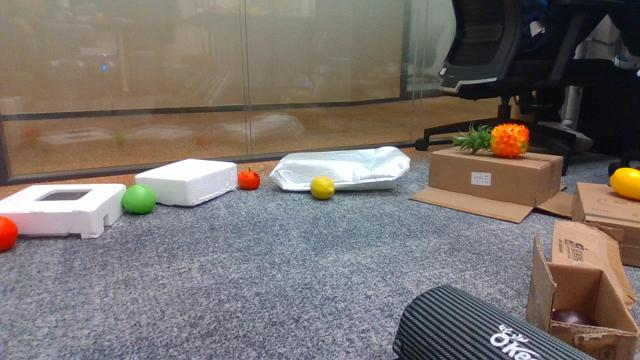} &
    \includegraphics[width=\linewidth]{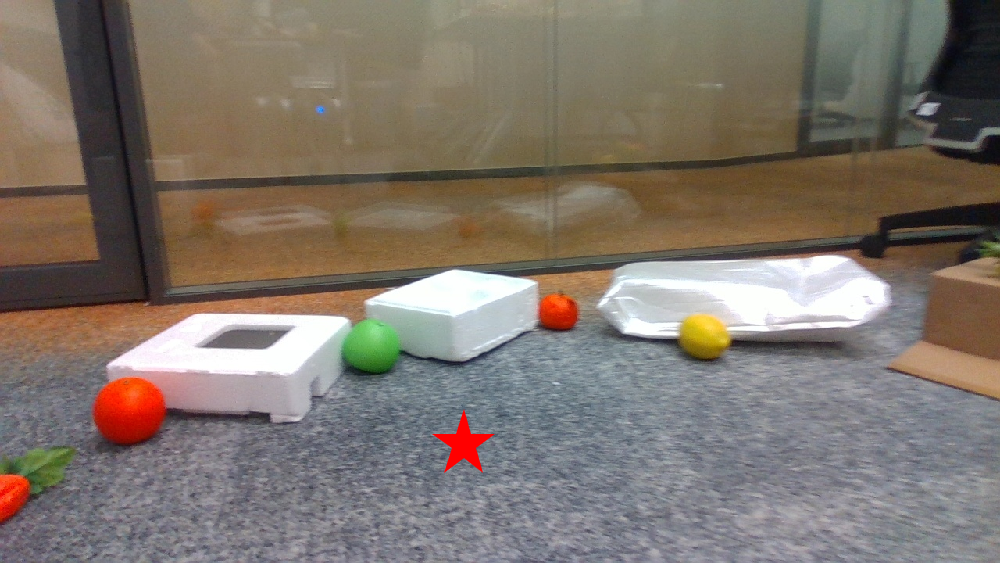} &
    \includegraphics[width=\linewidth]{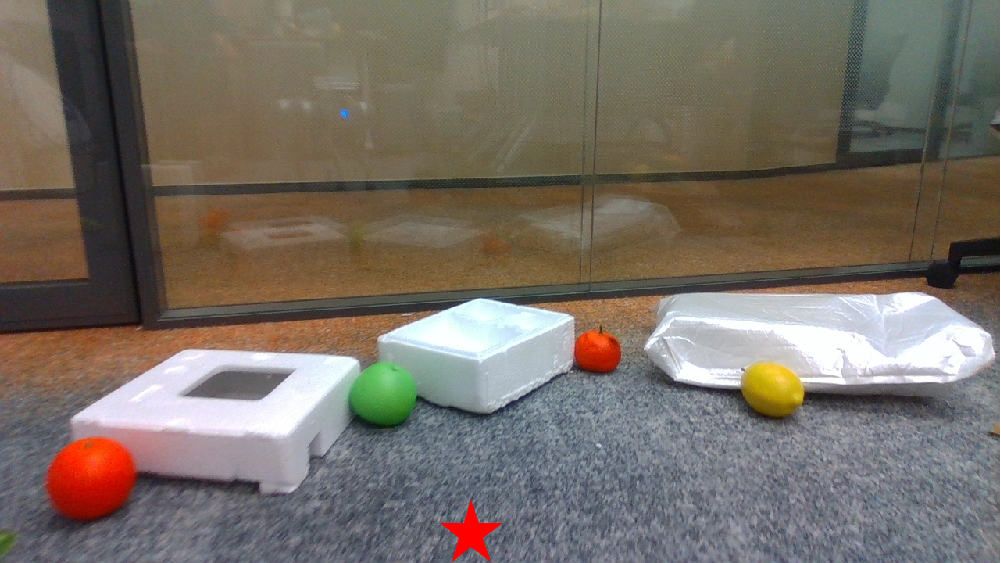} &
    \includegraphics[width=\linewidth]{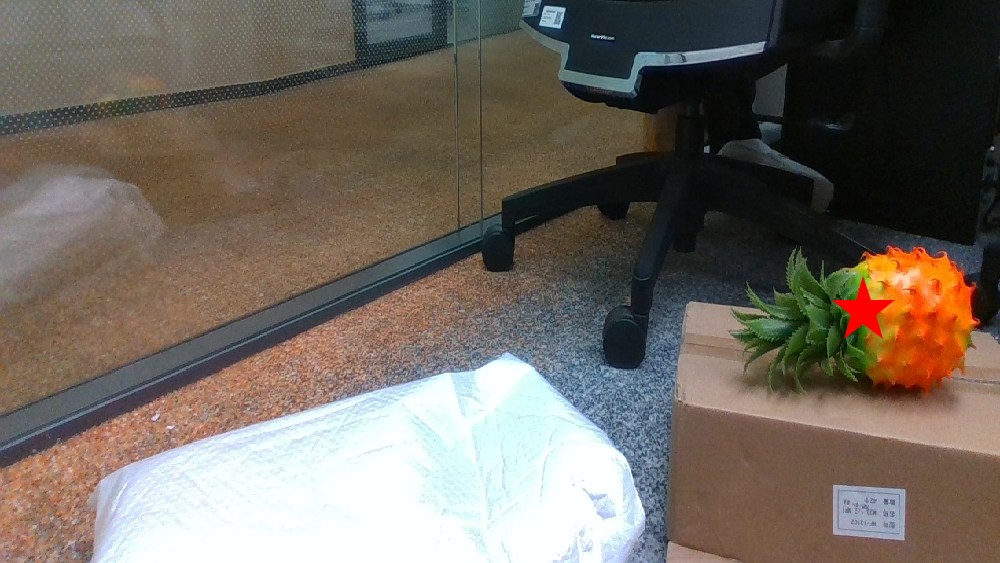} &
    \includegraphics[width=\linewidth]{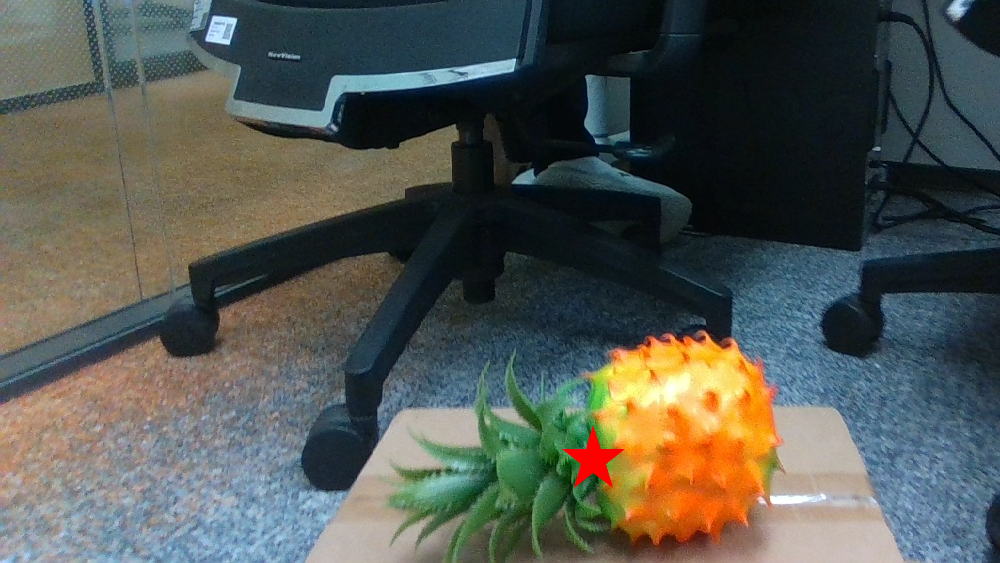} \\
    \multirow{6}{*}{\makecell{Complex\\Interaction}} & & & & & \\
    &
    \includegraphics[width=\linewidth]{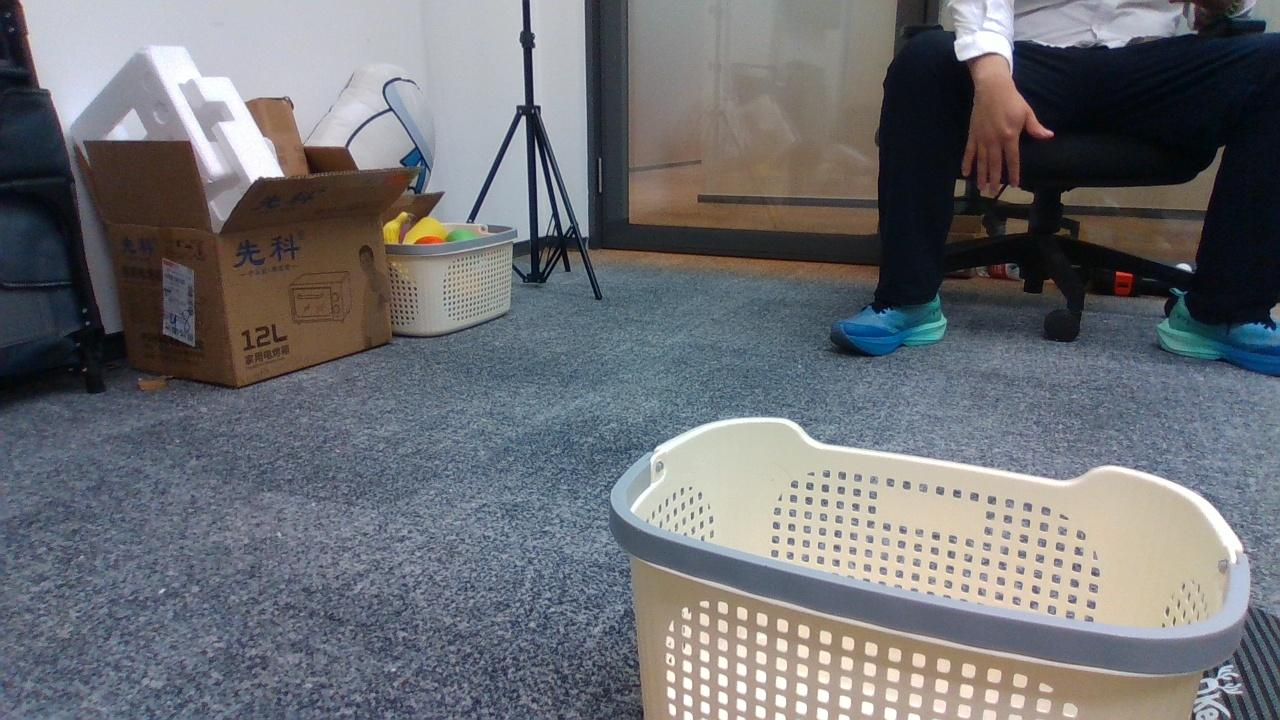} &
    \includegraphics[width=\linewidth]{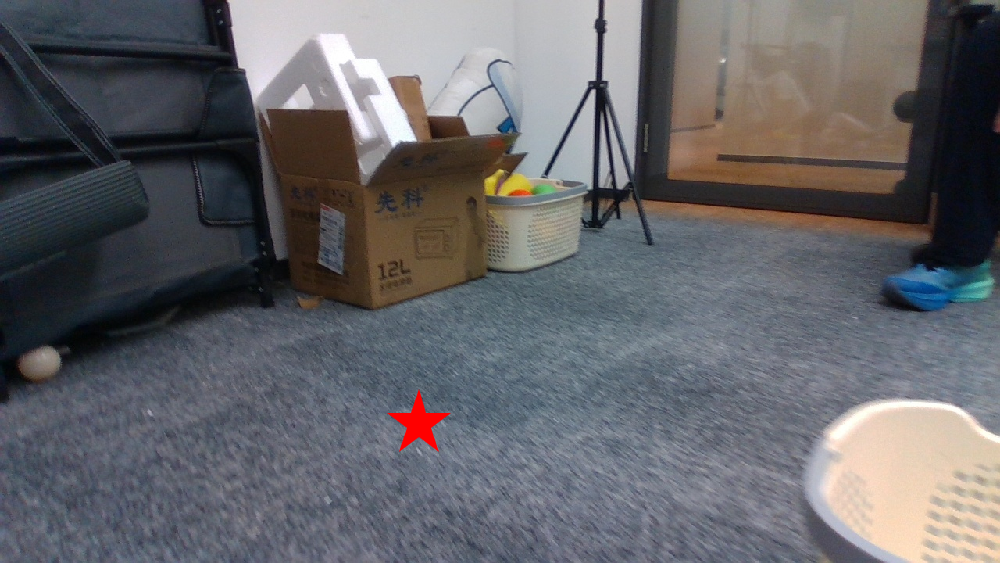} &
    \includegraphics[width=\linewidth]{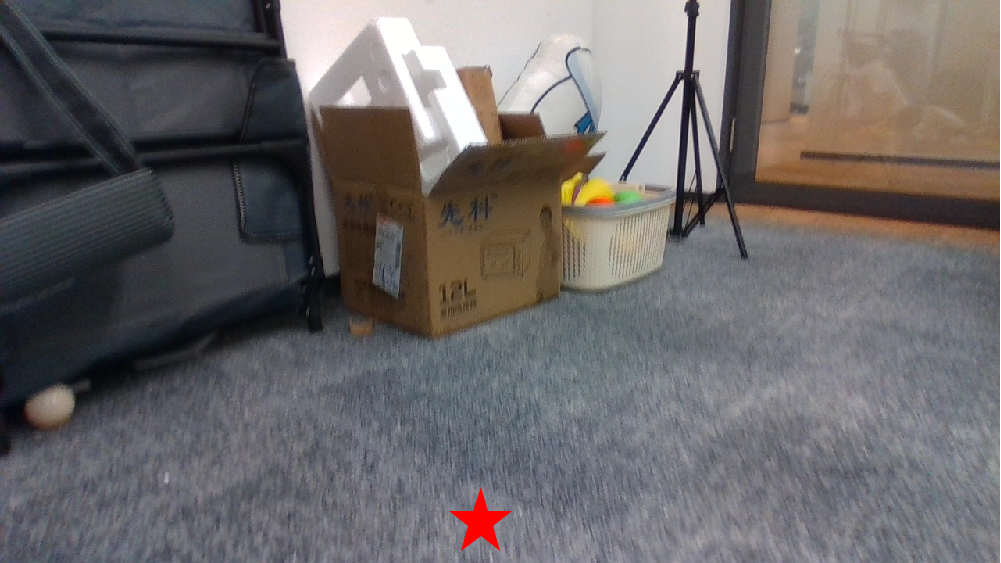} &
    \includegraphics[width=\linewidth]{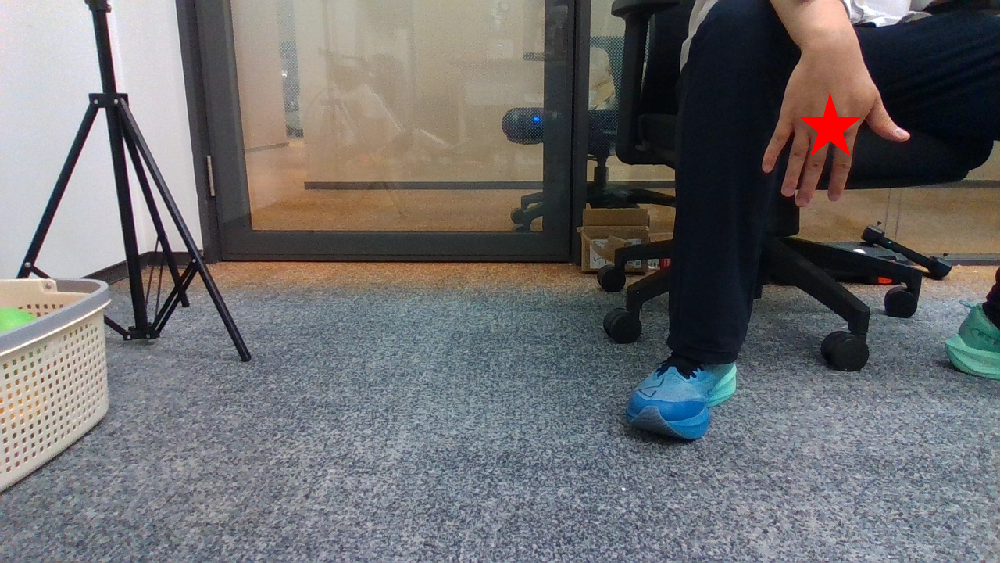} &
    \includegraphics[width=\linewidth]{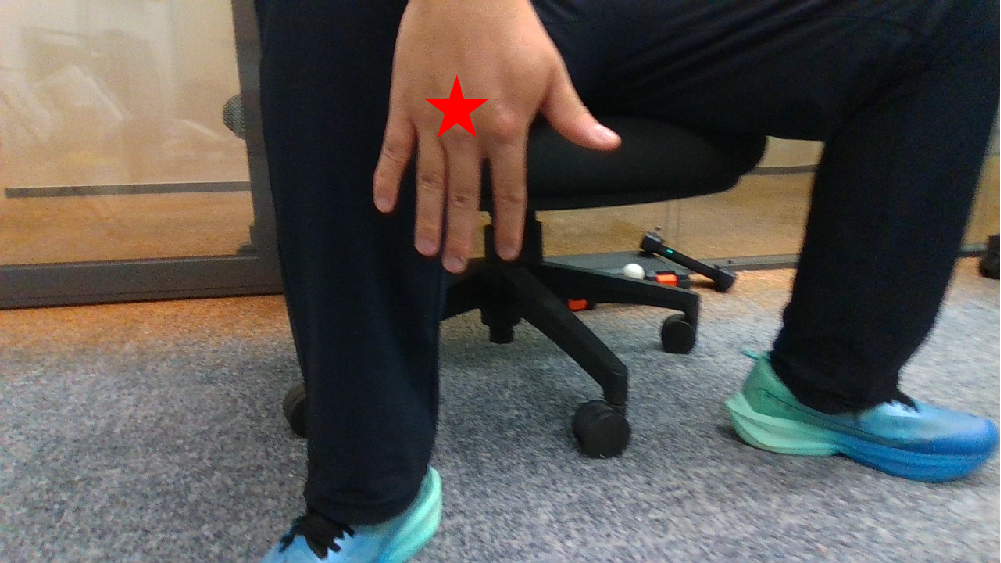} \\
    \multirow{6}{*}{\makecell{Complex\\Transport}} & & & & & \\
    &
    \includegraphics[width=\linewidth]{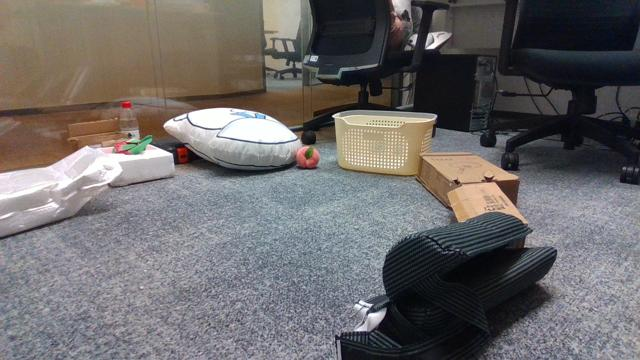} &
    \includegraphics[width=\linewidth]{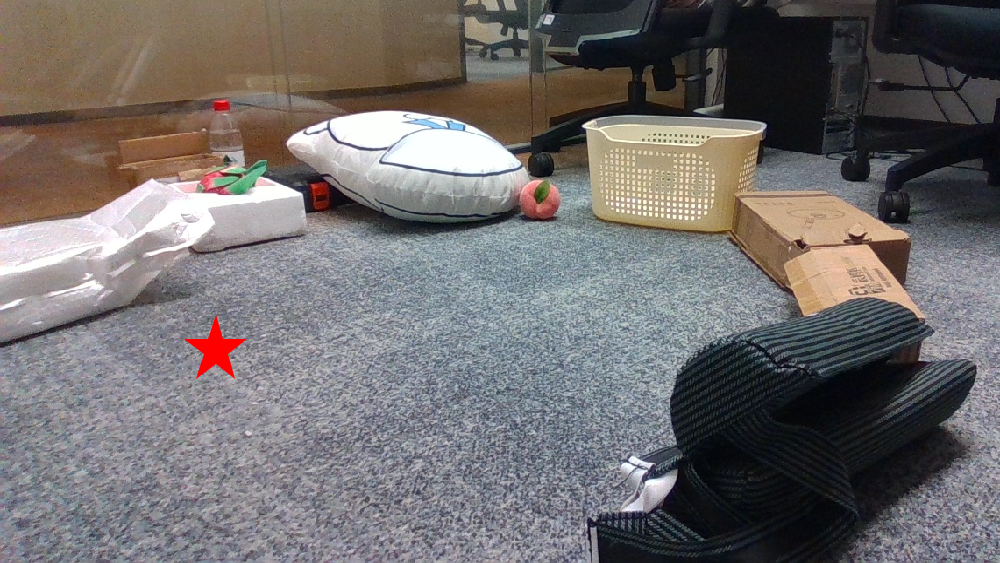} &
    \includegraphics[width=\linewidth]{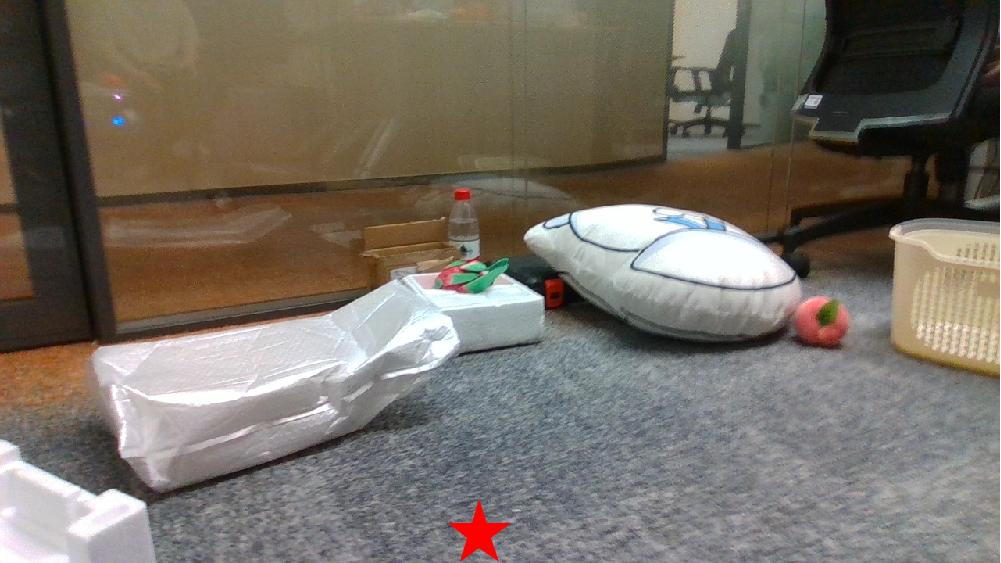} &
    \includegraphics[width=\linewidth]{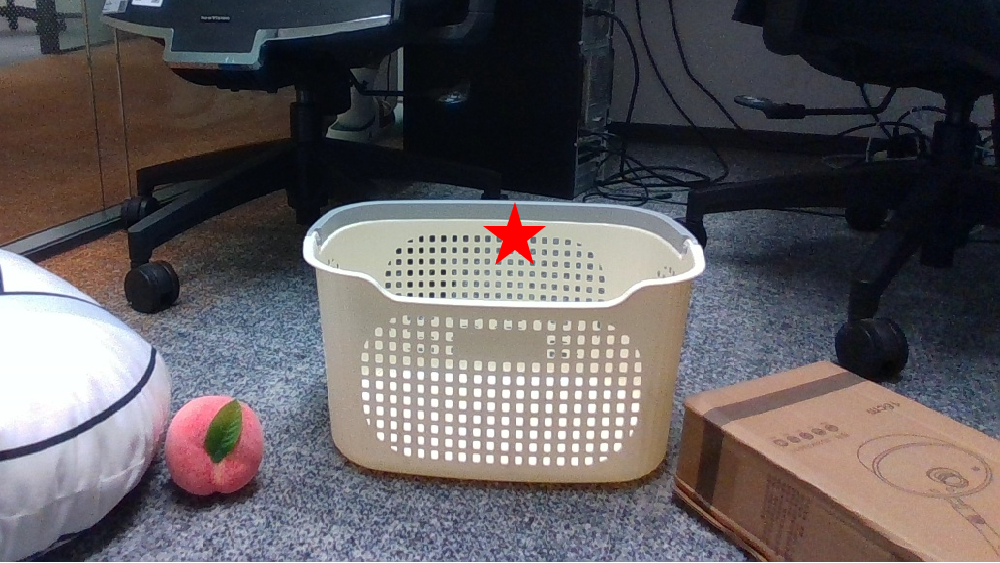} &
    \includegraphics[width=\linewidth]{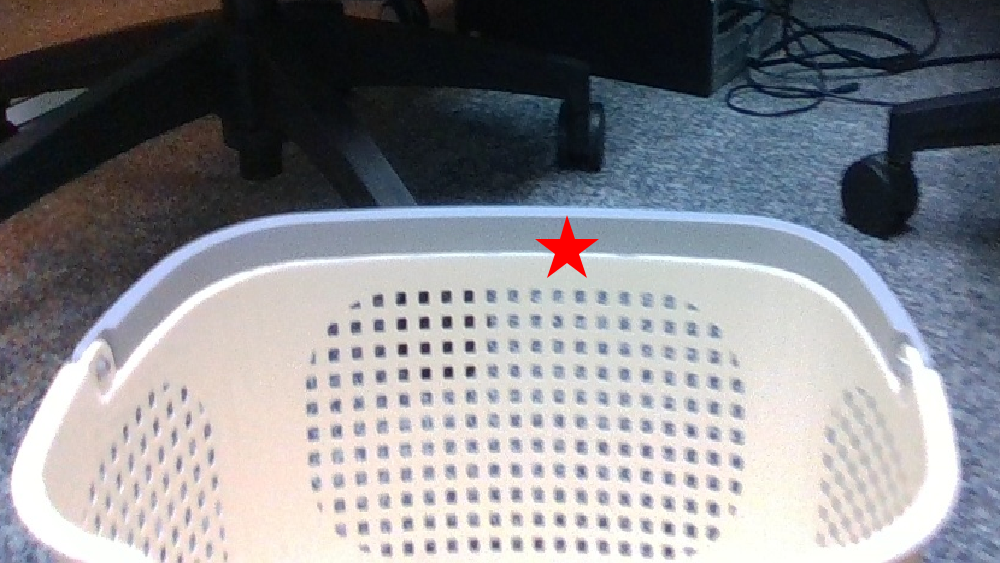} \\
    \bottomrule
    \end{tabular}}
\end{table}
