# Supplementary material for: Visual Embodied Brain: Let Multimodal Large Language Models See, Think, and Control in Spaces
Source: arXiv:2506.00123 source file (2025-05-30)
Supplement: Supplementary file 5 [file appendix_multimodal_demo.tex]

\definecolor{prompt}{rgb}{0.21,0.49,0.74}

\begin{figure*}[t]
    % \textbf{Image captioning and OCR}
    \centering
    \begin{tcolorbox}[rounded corners, colback=white, colframe=black, left=5pt, right=5pt, top=5pt, bottom=5pt]
        \begin{minipage}[ft]{0.35\textwidth} 
            \includegraphics[width=\linewidth]{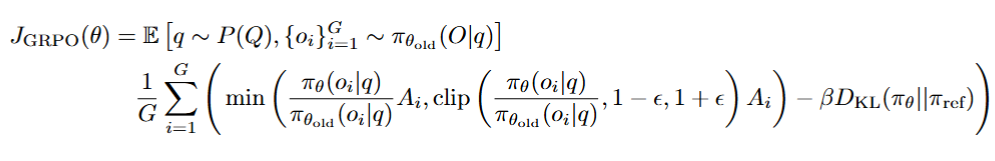}
        \end{minipage} \quad 
        \begin{minipage}[f]{0.6\textwidth} 
        \vspace{2mm}
        \small
        {\color{prompt}\textbf{Prompt:}} Convert the formula in the figure to latex format.  \\
    
        {\color{prompt}\textbf{Response:}} Sure, I'll convert the formula in the figure to LaTeX format for you. \\

        \begin{lstlisting}[breaklines=true]
```latex\n\
\begin{align}
J_{\text{GRPO}}(\theta) &= \mathbb{E}\left[q \sim P(Q), \{o_i\}_{i=1}^G \sim \pi_{\theta_{\text{old}}}(O|q)\right] \nonumber \\
&\quad \frac{1}{G} \sum_{i=1}^G \Bigg( \min\left(\frac{\pi_\theta(o_i|q)}{\pi_{\theta_{\text{old}}}(o_i|q)} A_i, \text{clip}\left(\frac{\pi_\theta(o_i|q)}{\pi_{\theta_{\text{old}}}(o_i|q)}, 1 - \epsilon, 1 + \epsilon\right) A_i \right) - \beta D_{\text{KL}} (\pi_\theta||\pi_{\text{ref}}) \Bigg),
\end{align}\n```
        \end{lstlisting}
        \end{minipage}
    \end{tcolorbox}
\end{figure*} \\

\begin{figure*}[t]
    % \textbf{Image captioning and OCR}
    \centering
    \begin{tcolorbox}[rounded corners, colback=white, colframe=black, left=5pt, right=5pt, top=5pt, bottom=5pt]
        \begin{minipage}[ft]{0.35\textwidth} 
            \includegraphics[width=\linewidth]{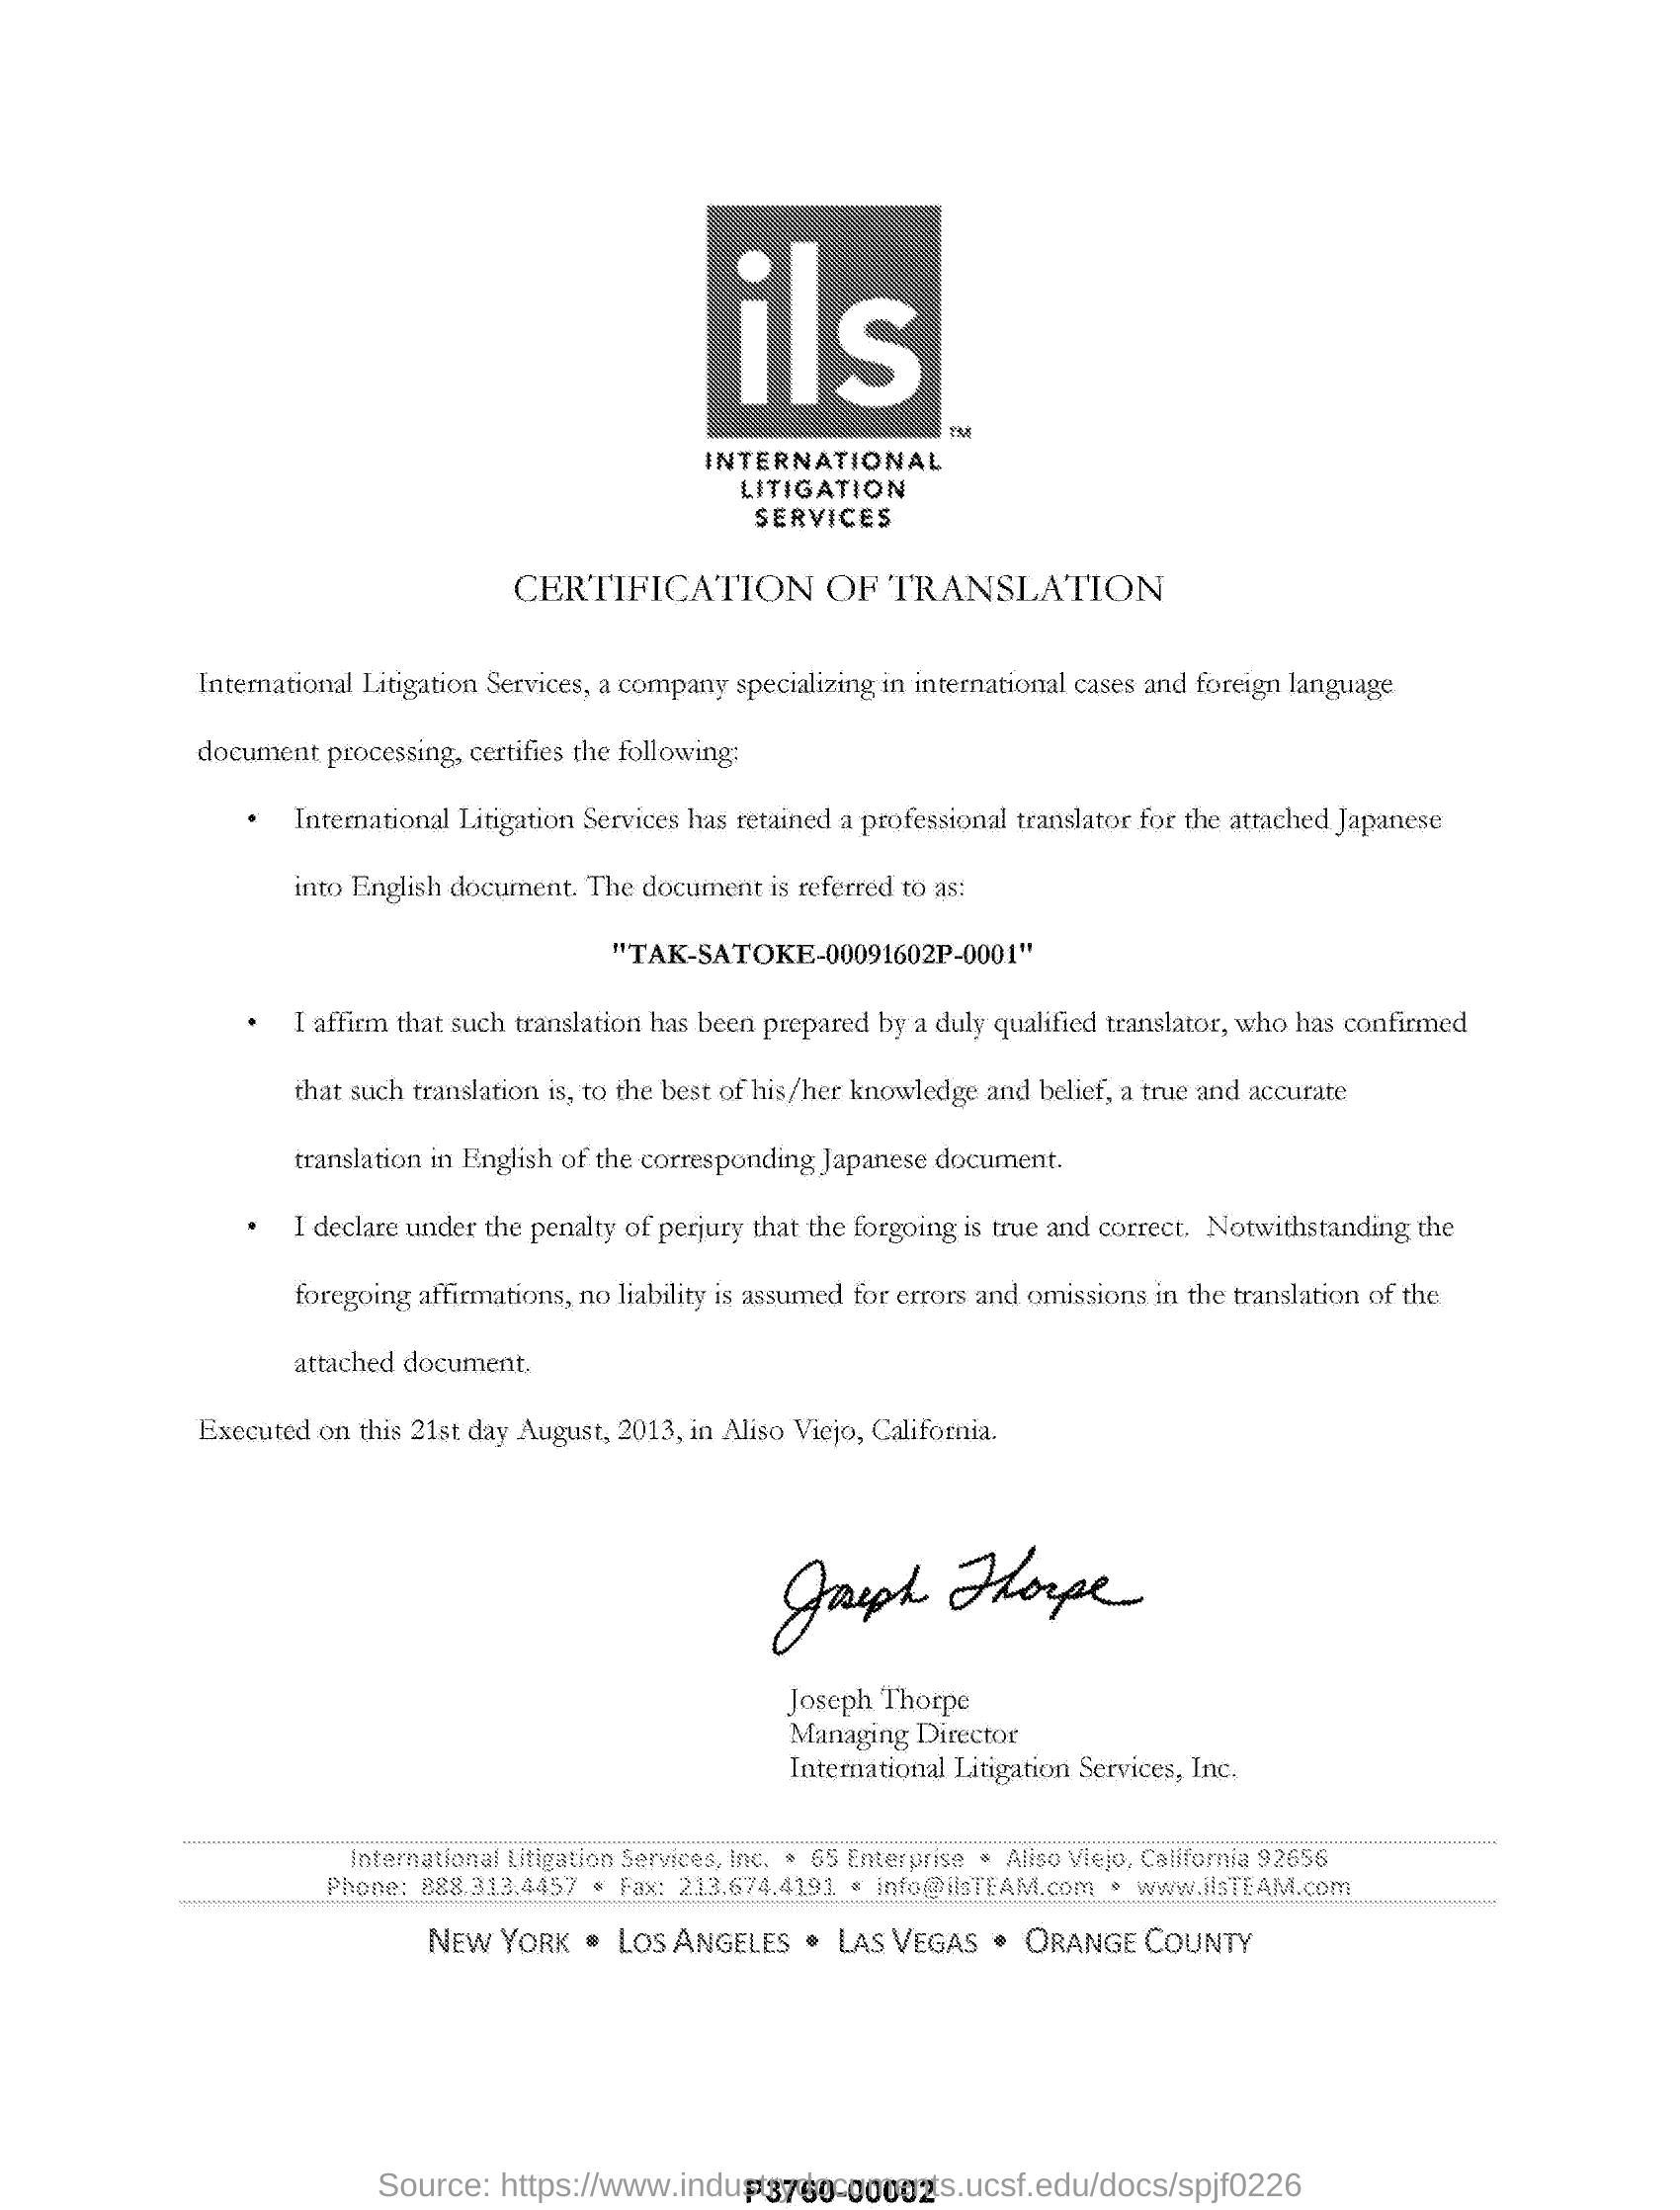}
        \end{minipage} \quad 
        \begin{minipage}[f]{0.6\textwidth} 
        \vspace{2mm}
        \small
        {\color{prompt}\textbf{Prompt:}} Explain what's this document for.  \\
    
        {\color{prompt}\textbf{Response:}} This is a Certification of Translation issued by International Litigation Services (ILS), a company specializing in international cases and foreign language document processing. The certification affirms that the attached Japanese into English document has been translated by a professionally qualified translator, and that the translation is true and accurate to the best of the translator's knowledge and belief. \\

        {\color{prompt}\textbf{Prompt:}} Who signed this document?  \\
    
        {\color{prompt}\textbf{Response:}} Joseph Thorpe \\

        {\color{prompt}\textbf{Prompt:}} When and where was this document issued?  \\
    
        {\color{prompt}\textbf{Response:}} 21st day August, 2013 in Aliso Viejo, California \\
        
        \end{minipage}
    \end{tcolorbox}
\end{figure*}

\begin{figure*}[t]
    % \textbf{Image captioning and OCR}
    \centering
    \begin{tcolorbox}[rounded corners, colback=white, colframe=black, left=5pt, right=5pt, top=5pt, bottom=5pt]
        \begin{minipage}[ft]{0.35\textwidth} 
            \includegraphics[width=\linewidth]{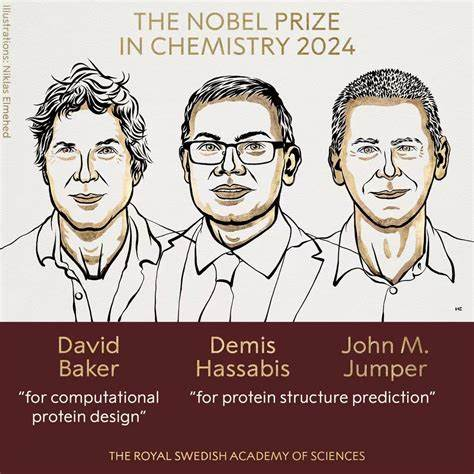}
        \end{minipage} \quad 
        \begin{minipage}[f]{0.6\textwidth} 
        \vspace{2mm}
        \small
        {\color{prompt}\textbf{Prompt:}} Explain the content in this picture.  \\
    
        {\color{prompt}\textbf{Response:}} The image is an illustration of three individuals, each with their names and contributions to the 2024 Nobel Prize in Chemistry listed below them. The text at the top reads "THE NOBEL PRIZE IN CHEMISTRY 2024." Below the names, there are two quotes indicating their respective contributions: \\
        
        1. \textbf{David Baker}:\\  - "for computational protein design" \\
        2. \textbf{Demis Hassabis}:\\   - "for protein structure prediction" \\
        3. \textbf{John M. Jumper}:\\    - "for protein structure prediction" \\
        % 1. \textbf{David Baker}:
        % \begin{itemize}
        %     \item "for computational protein design"
        % \end{itemize}
        % 2. \textbf{Demis Hassabis}:
        % \begin{itemize}
        %     \item "for protein structure prediction"
        % \end{itemize}
        % 3. \textbf{John M. Jumper}:
        % \begin{itemize}
        %     \item "for protein structure prediction"
        % \end{itemize}
        
        At the bottom of the image, it states "THE ROYAL SWEDISH ACADEMY OF SCIENCES." \\
        
        The illustration style is simple and cartoon-like, with each person depicted in a similar manner, wearing collared shirts. The background is plain white, and the text is in black and gold colors for emphasis. The artist\'s name, Niklas Elmehed, is credited on the left side of the image. \\
        \end{minipage}
    \end{tcolorbox}
\end{figure*}

\begin{figure*}[t]
    % \textbf{Image captioning and OCR}
    \centering
    \begin{tcolorbox}[rounded corners, colback=white, colframe=black, left=5pt, right=5pt, top=5pt, bottom=5pt]
        \begin{minipage}[ft]{0.35\textwidth} 
            \includegraphics[width=\linewidth]{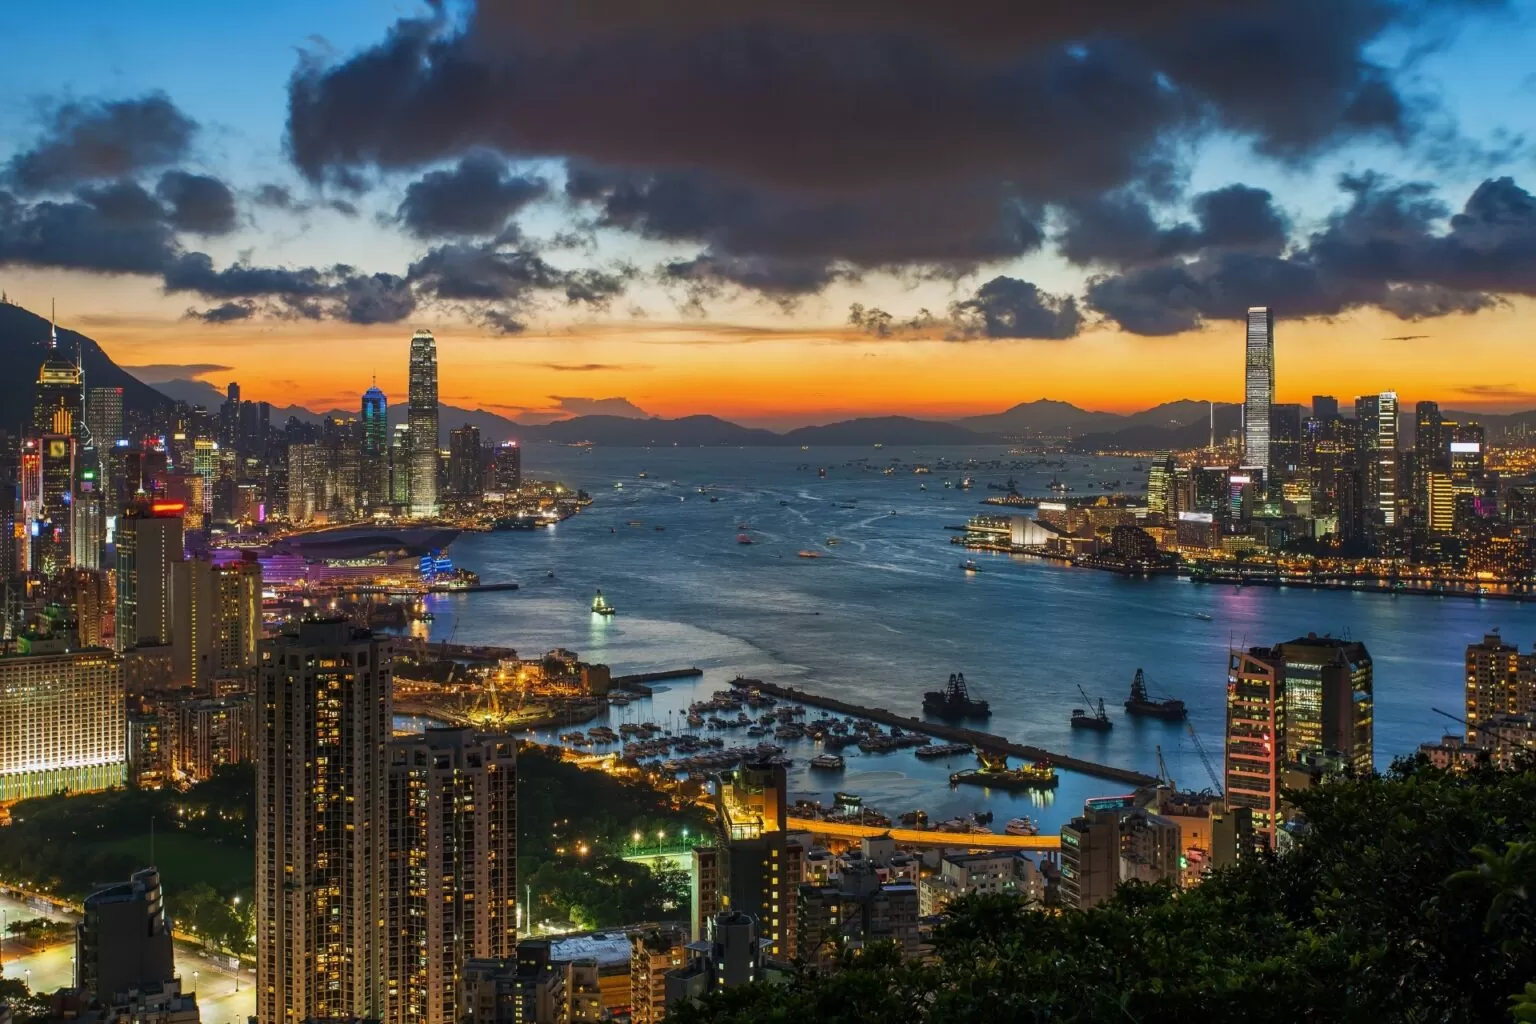}
        \end{minipage} \quad 
        \begin{minipage}[f]{0.6\textwidth} 
        \vspace{2mm}
        \small
        {\color{prompt}\textbf{Prompt:}} Describe this image in detail.  \\
    
        {\color{prompt}\textbf{Response:}} The image depicts a panoramic view of a bustling cityscape at dusk or early evening, with the skyline illuminated by artificial lights against a backdrop of a vibrant sky transitioning from blue to orange hues. The city is densely packed with high-rise buildings, including skyscrapers and office towers, some of which are lit up, creating a striking contrast with the darkening sky. \\
        
        In the foreground, there is a mix of residential and commercial buildings, with some areas appearing to be under construction as evidenced by cranes and exposed structures. A large body of water runs through the center of the image, reflecting the lights from the buildings and boats. Several boats and ships are visible on the water, suggesting active maritime traffic. \\
        
        The background features a range of mountains, partially obscured by clouds, adding depth to the scene. The overall atmosphere is one of urban vibrancy and modernity, with the interplay of natural and man-made elements creating a dynamic and visually captivating landscape. \\
        
        \end{minipage}
    \end{tcolorbox}
\end{figure*}
